# Supplementary material for: AutoTune: Controller Tuning for High-Speed Flight
Source: arXiv:2103.10698 source file (2022-02-08)
Supplement: Supplementary file 1 [file appendices.tex]

\section{Supplementary}

\subsection{Tracks} \label{app:tracks}

\begin{center}
\includegraphics[width=0.49\linewidth]{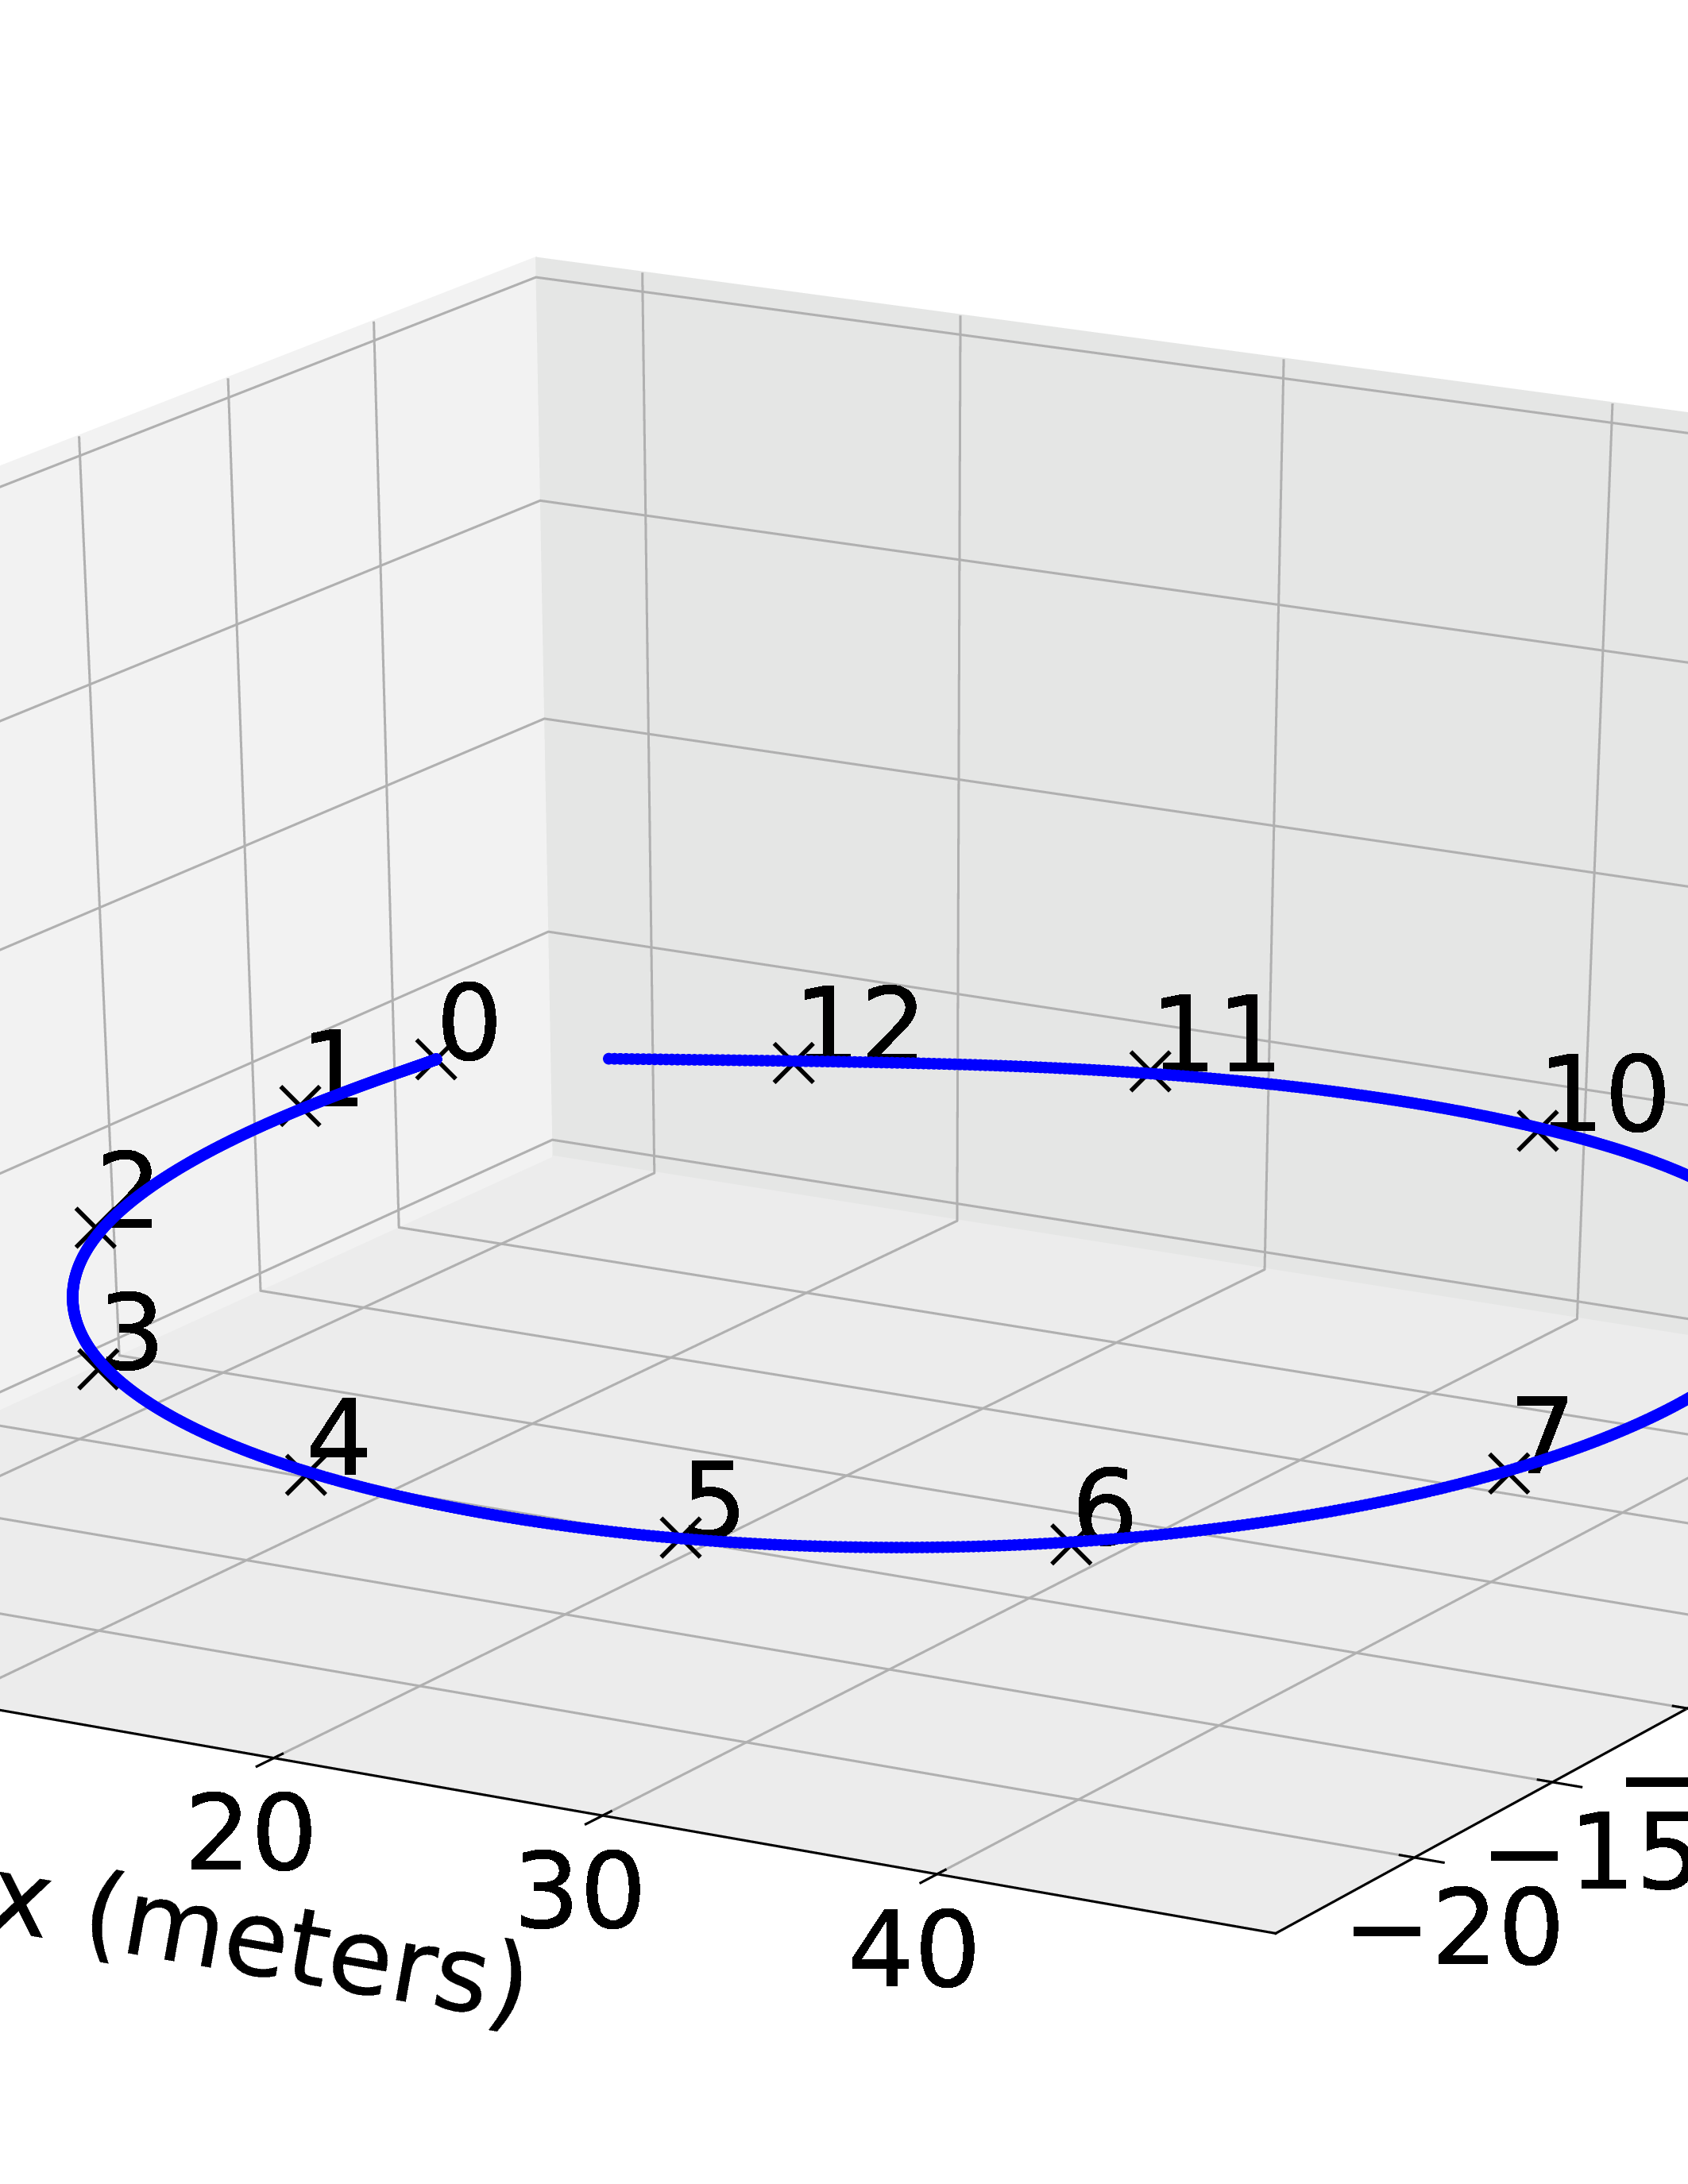}
\includegraphics[width=0.49\linewidth]{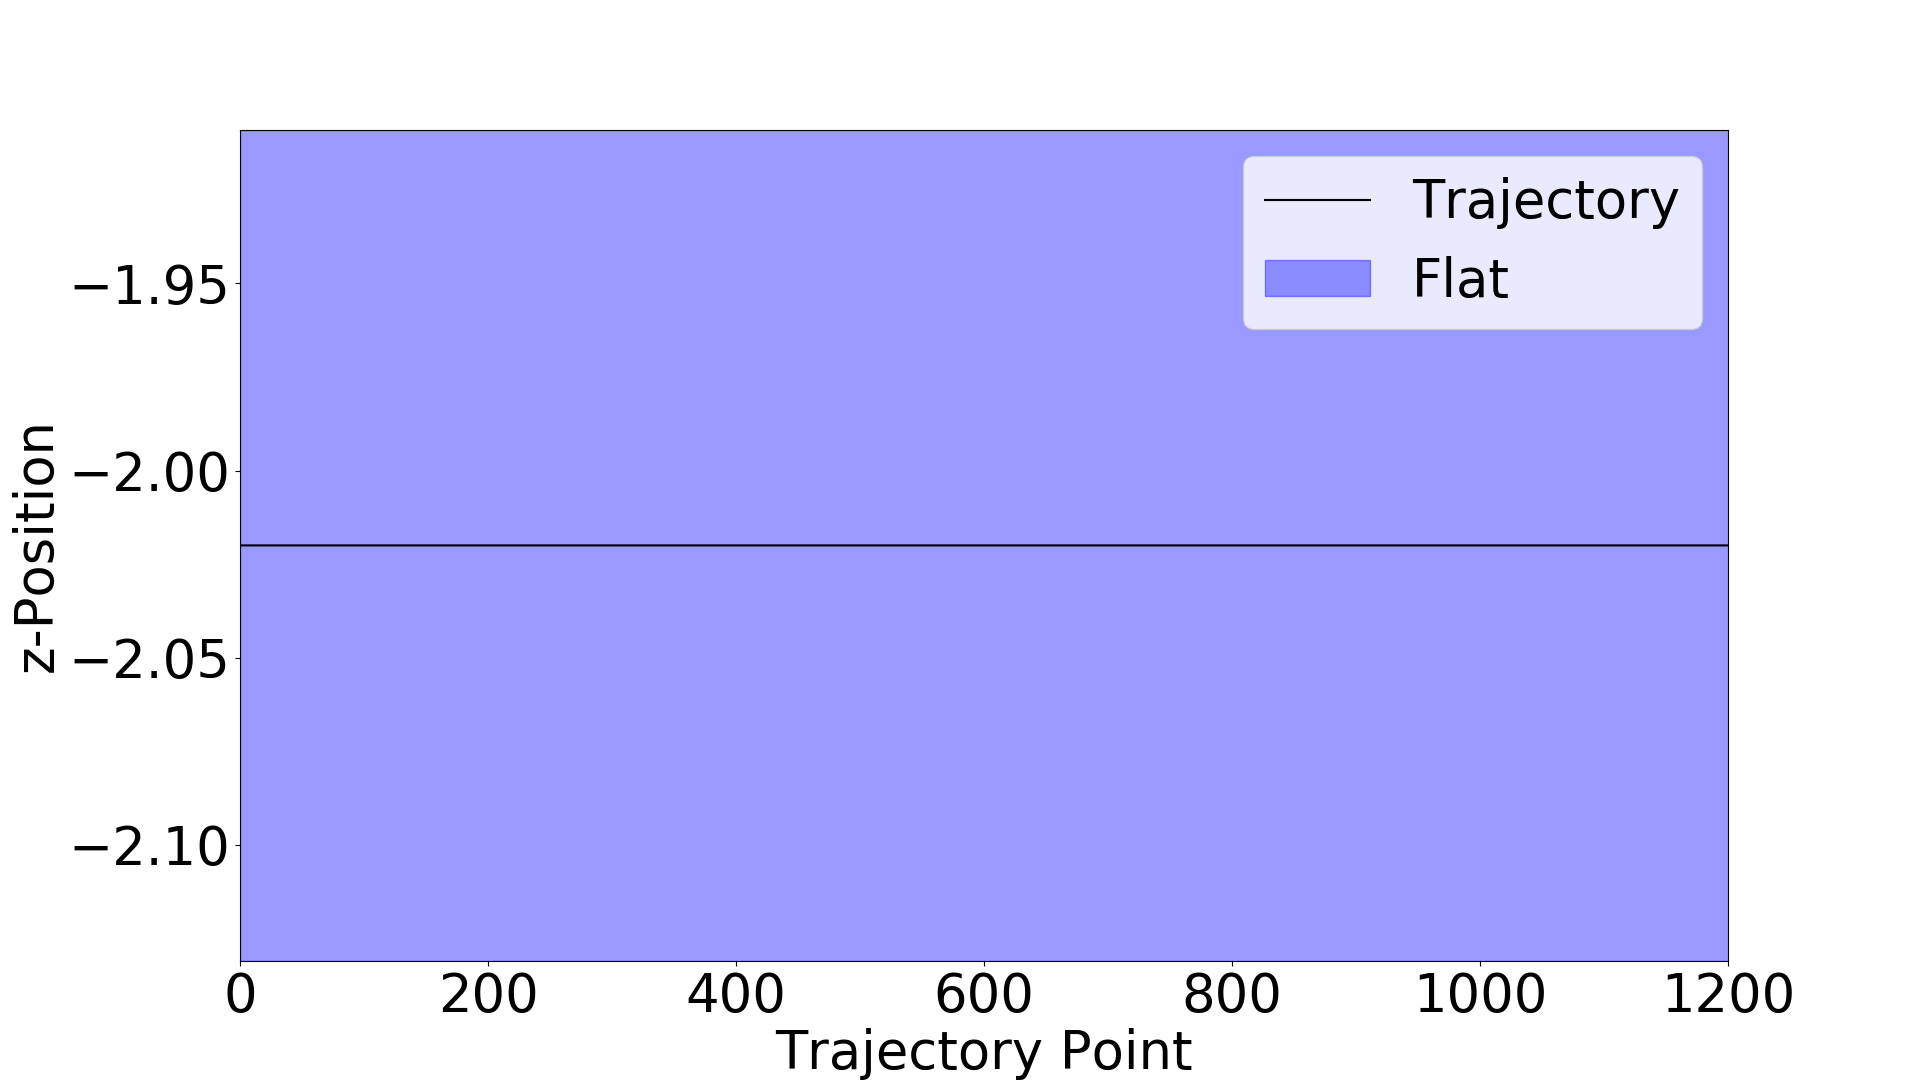}
\captionof{figure}{Circle track.}
\label{fig:appendix_soccer_easy}

\includegraphics[width=0.49\linewidth]{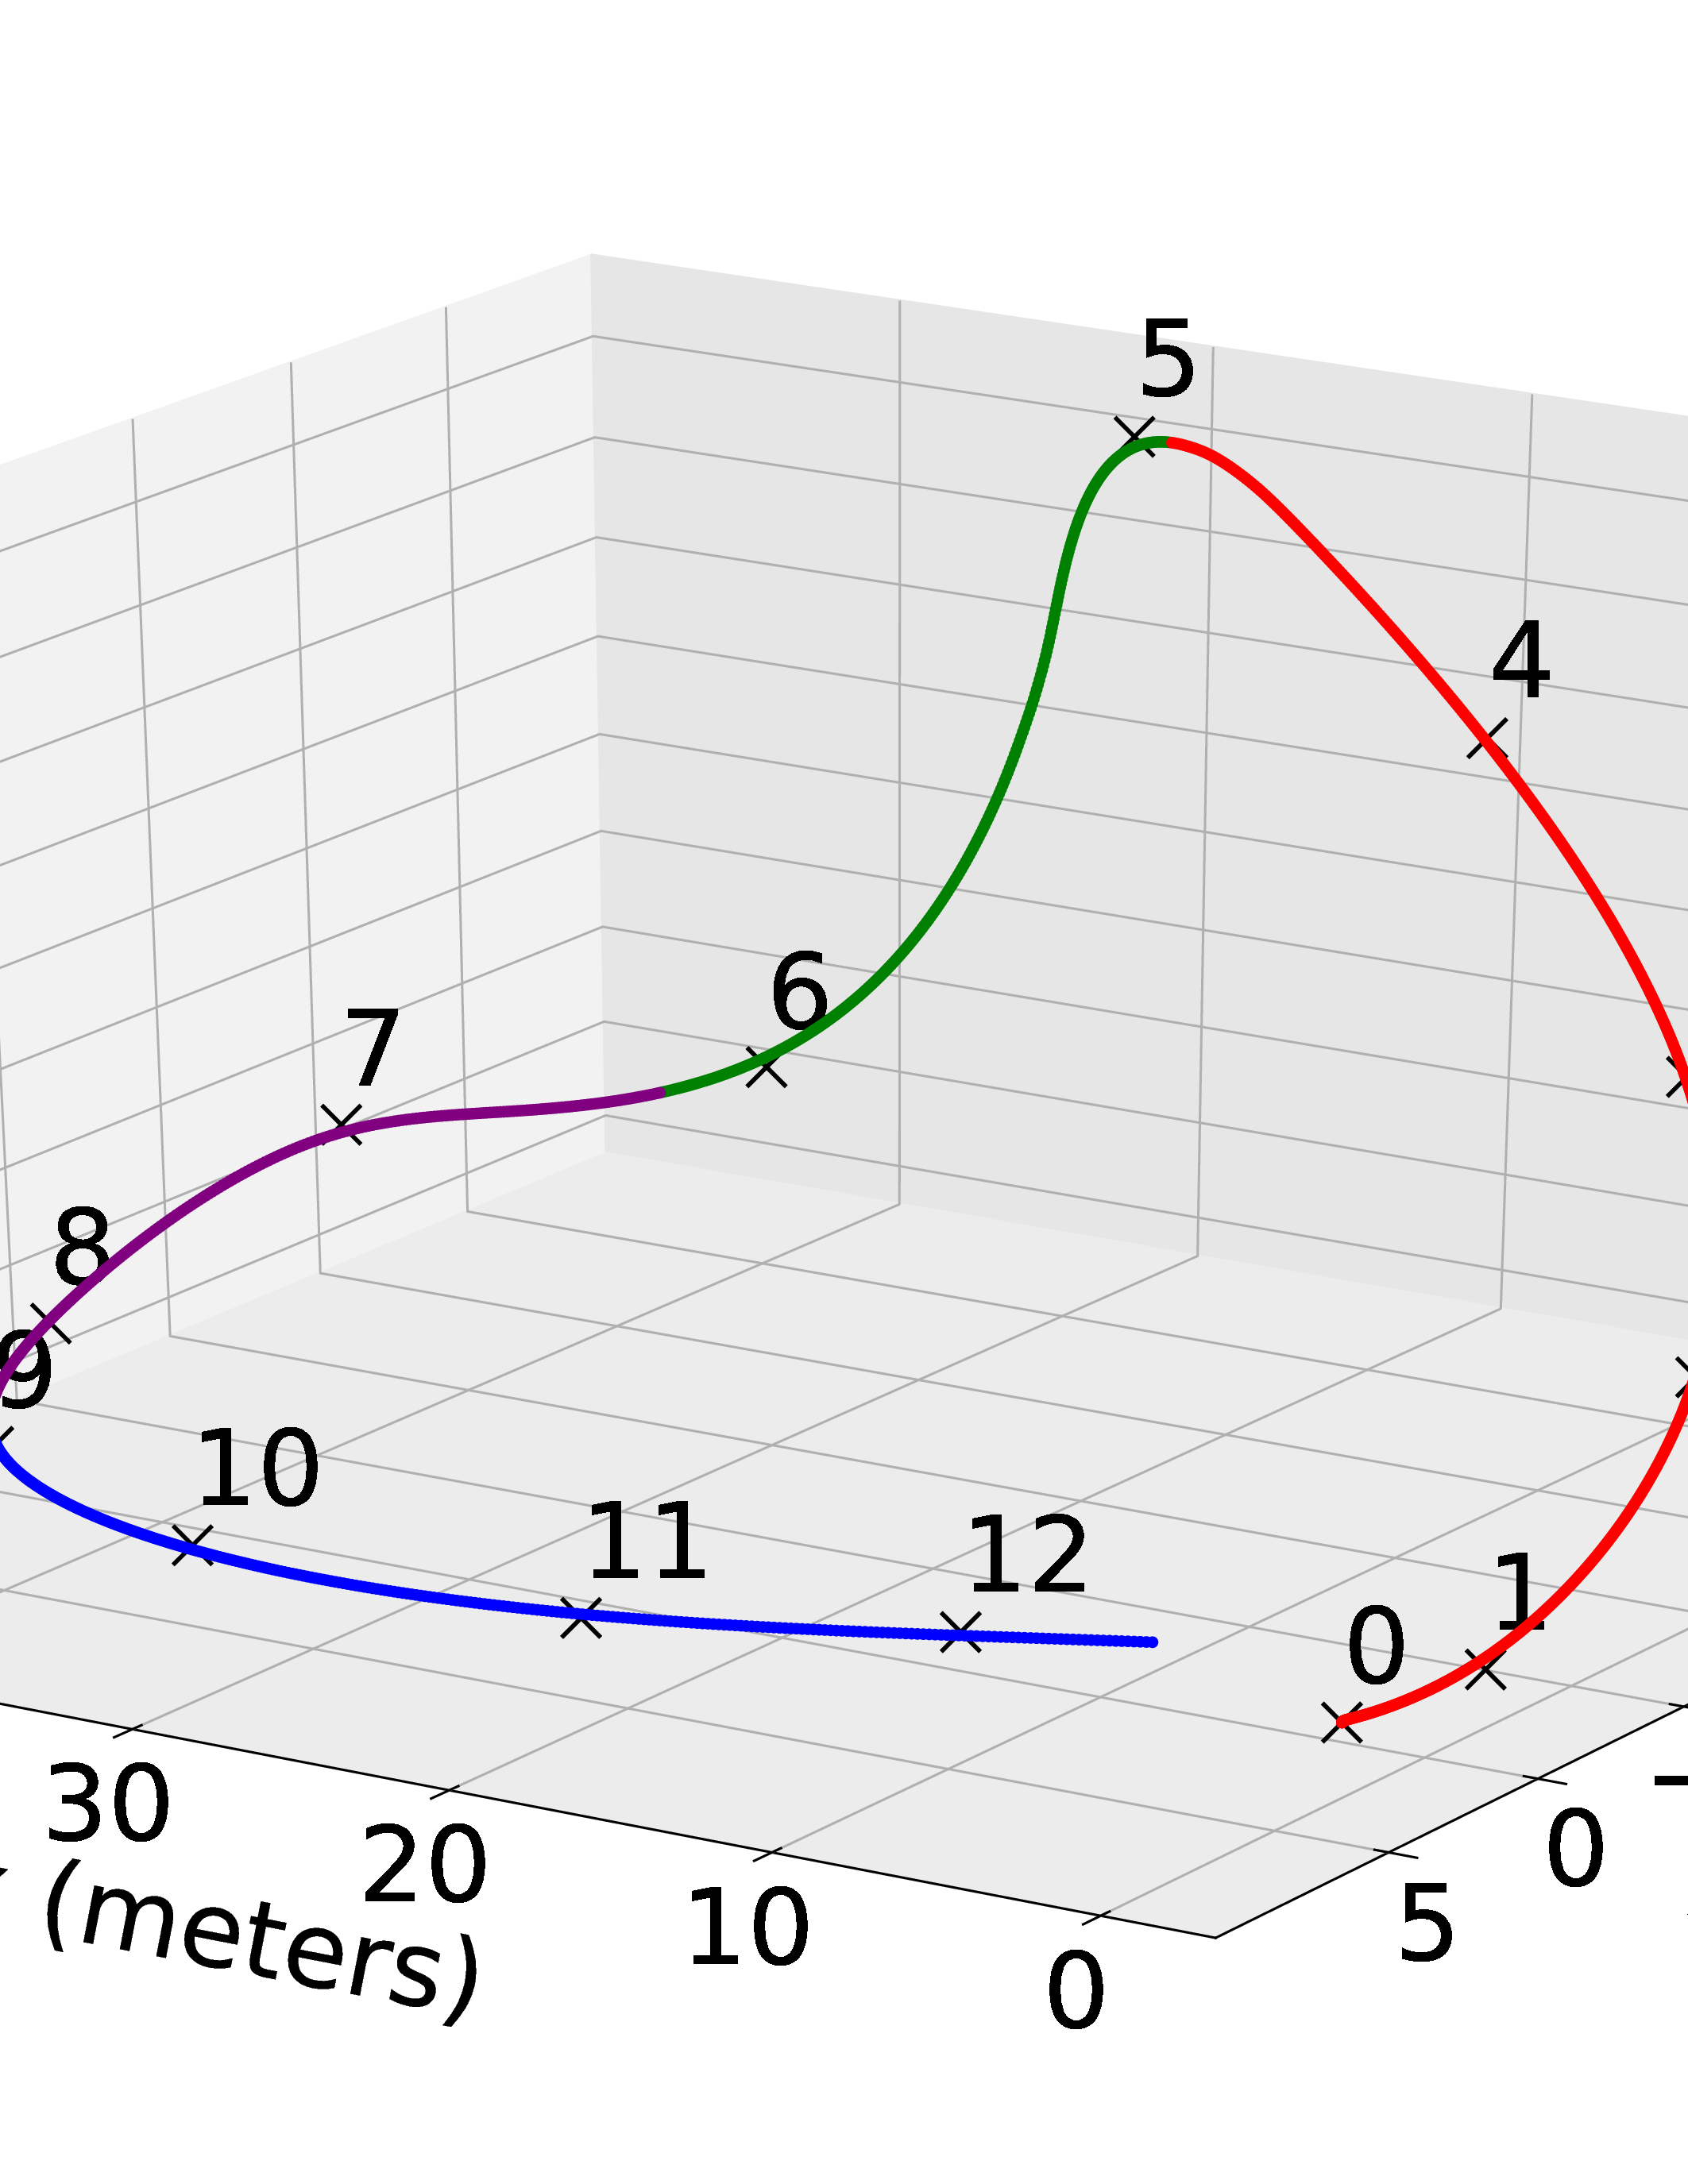}
\includegraphics[width=0.49\linewidth]{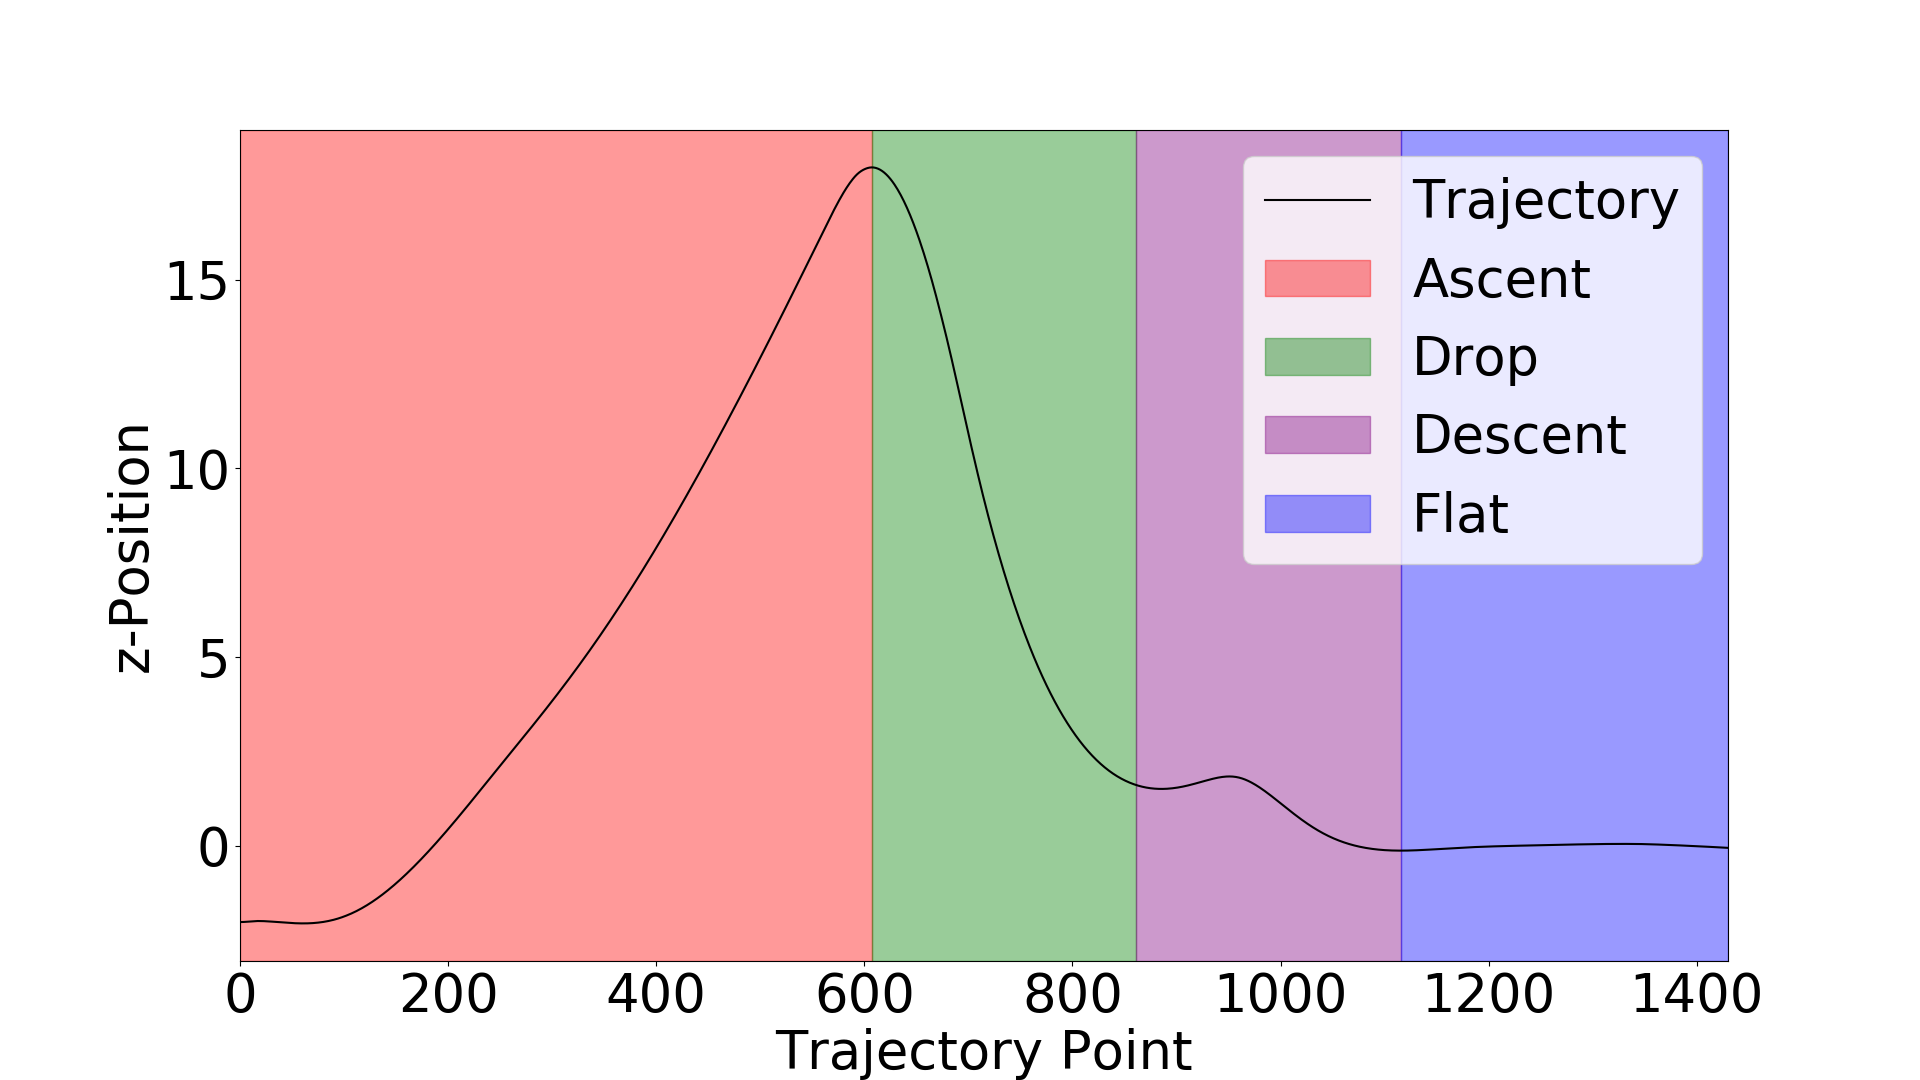}
\captionof{figure}{Drop track.}
\label{fig:appendix_drop_easy}

\includegraphics[width=0.49\linewidth]{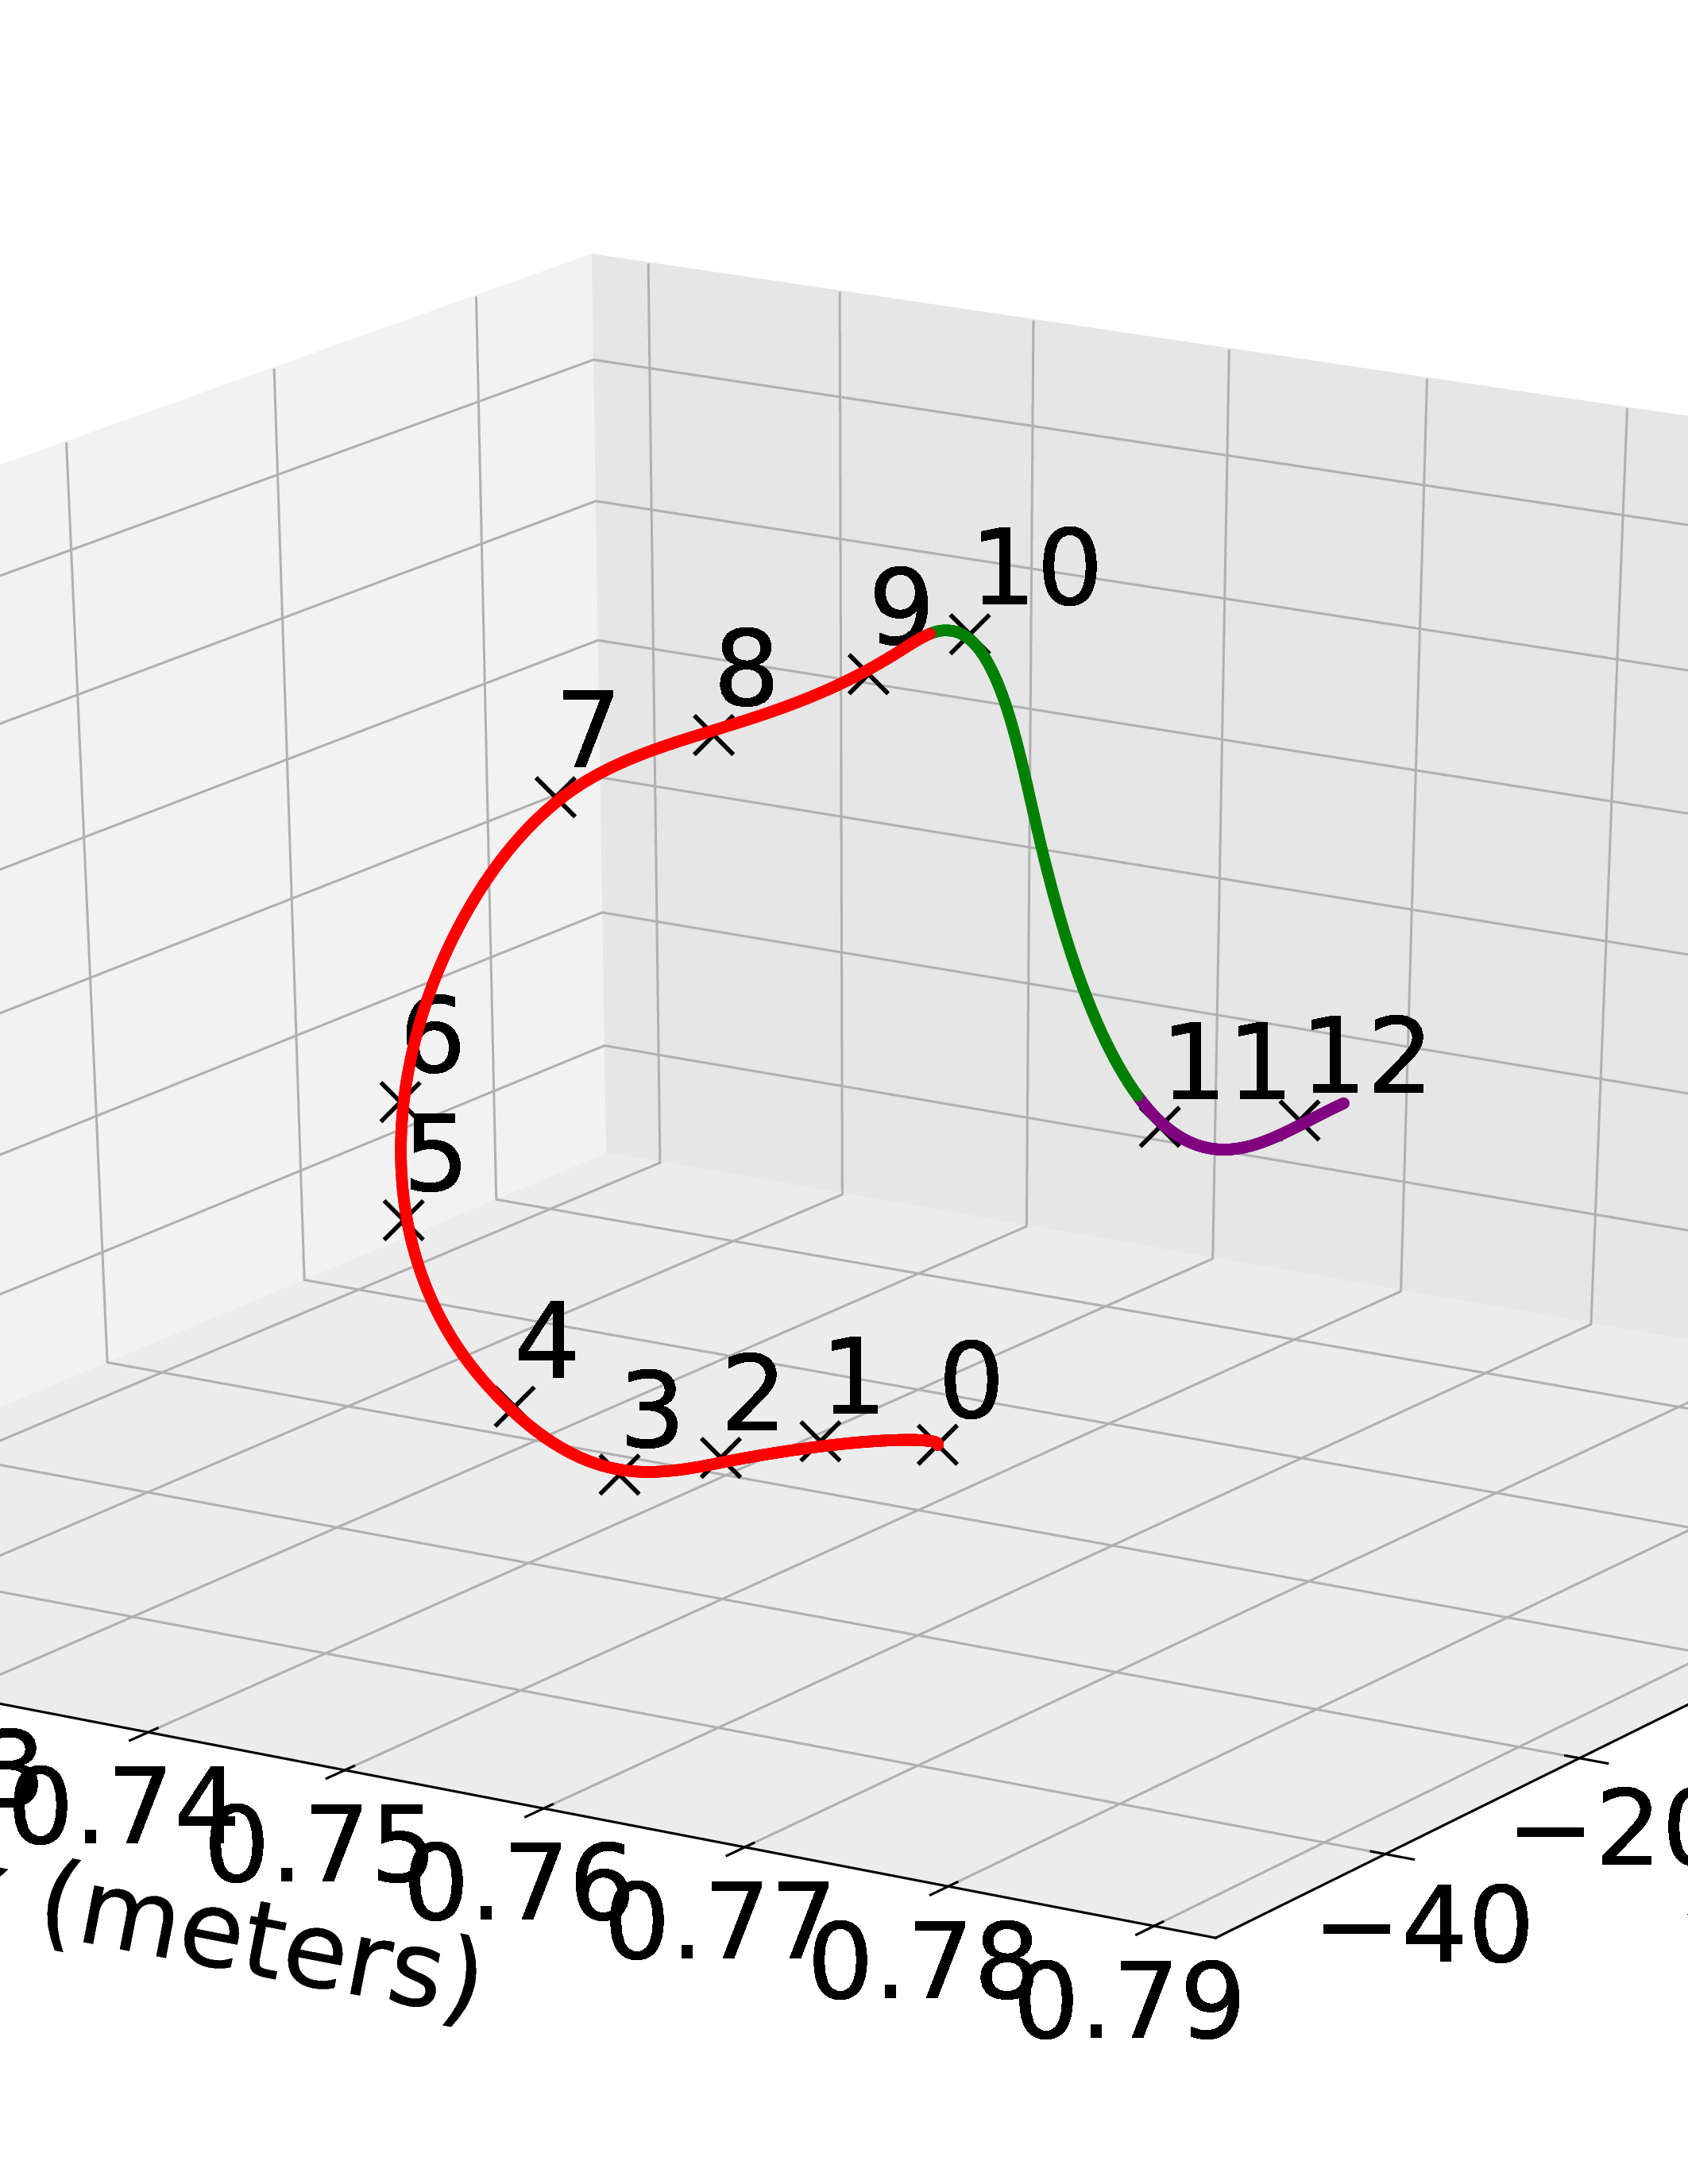}
\includegraphics[width=0.49\linewidth]{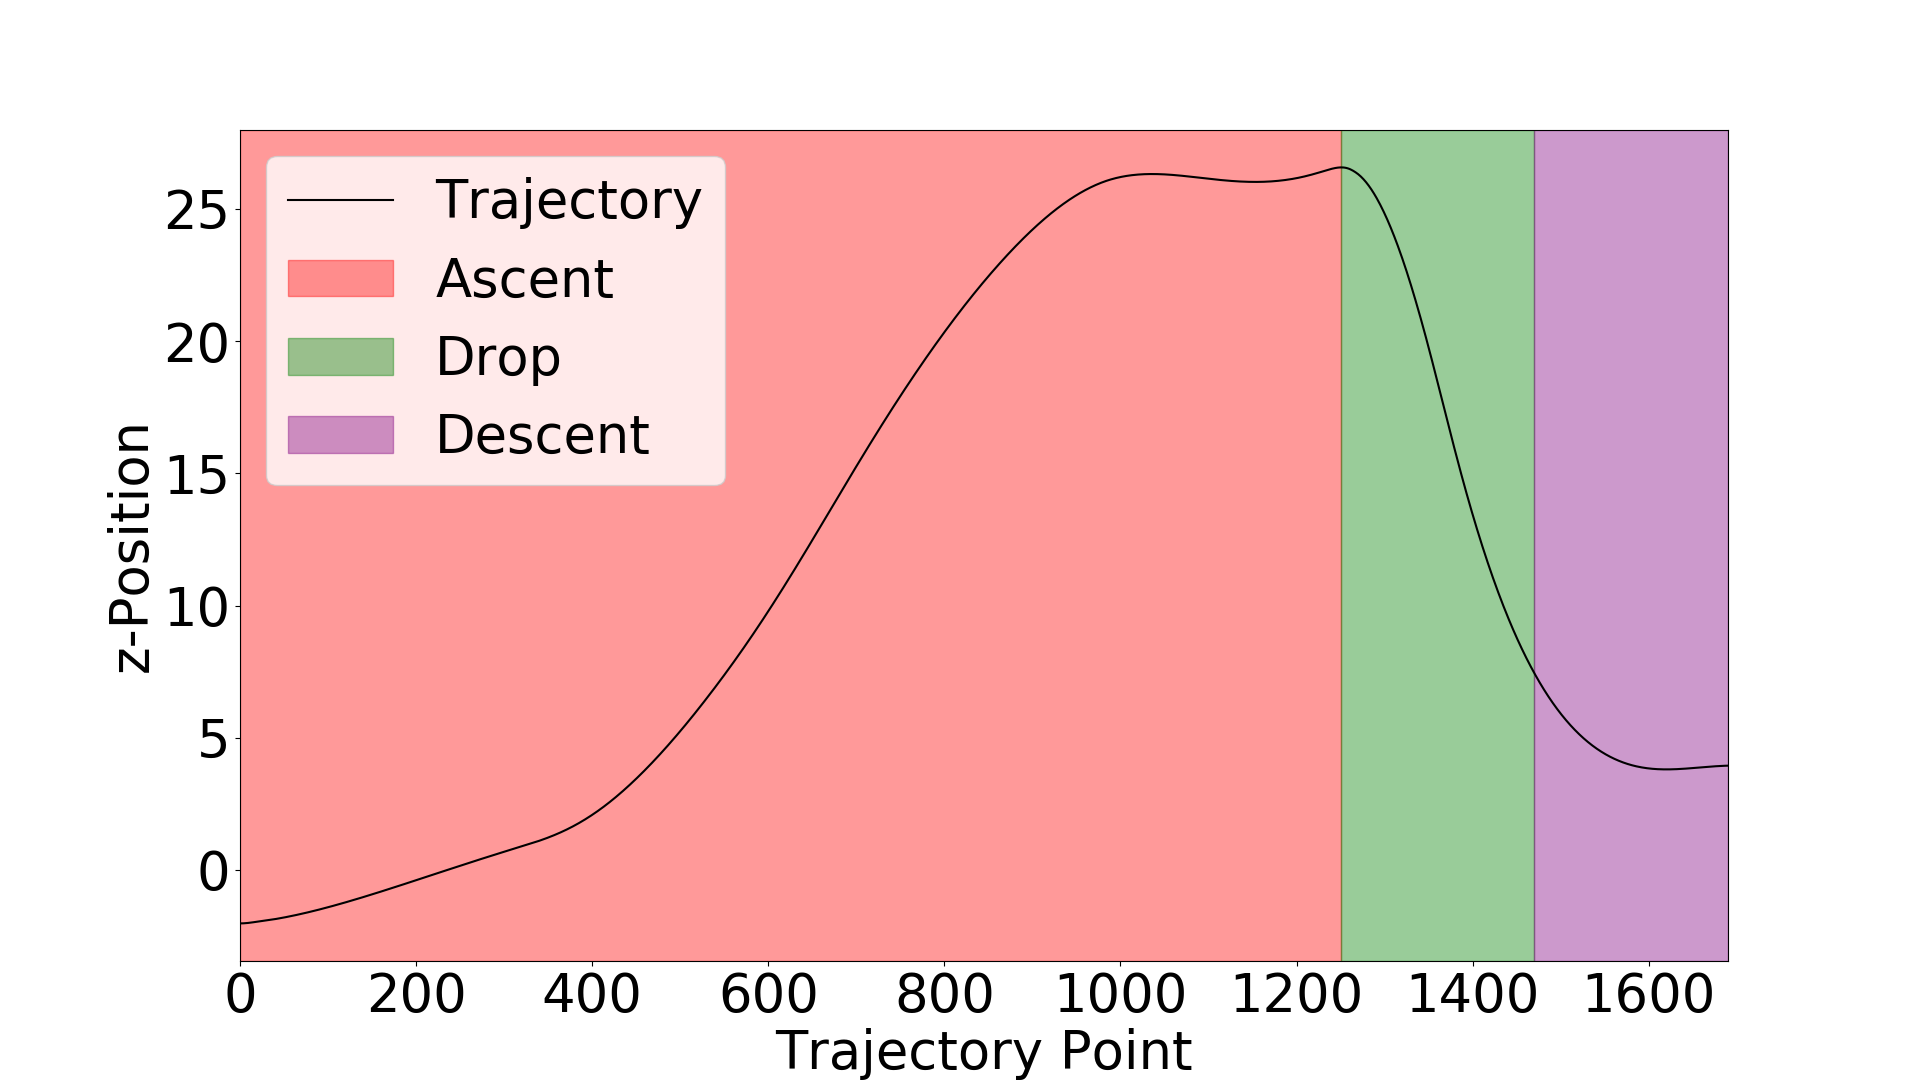}
\captionof{figure}{Flip track.}
\label{fig:appendix_flip_easy}

\includegraphics[width=0.49\linewidth]{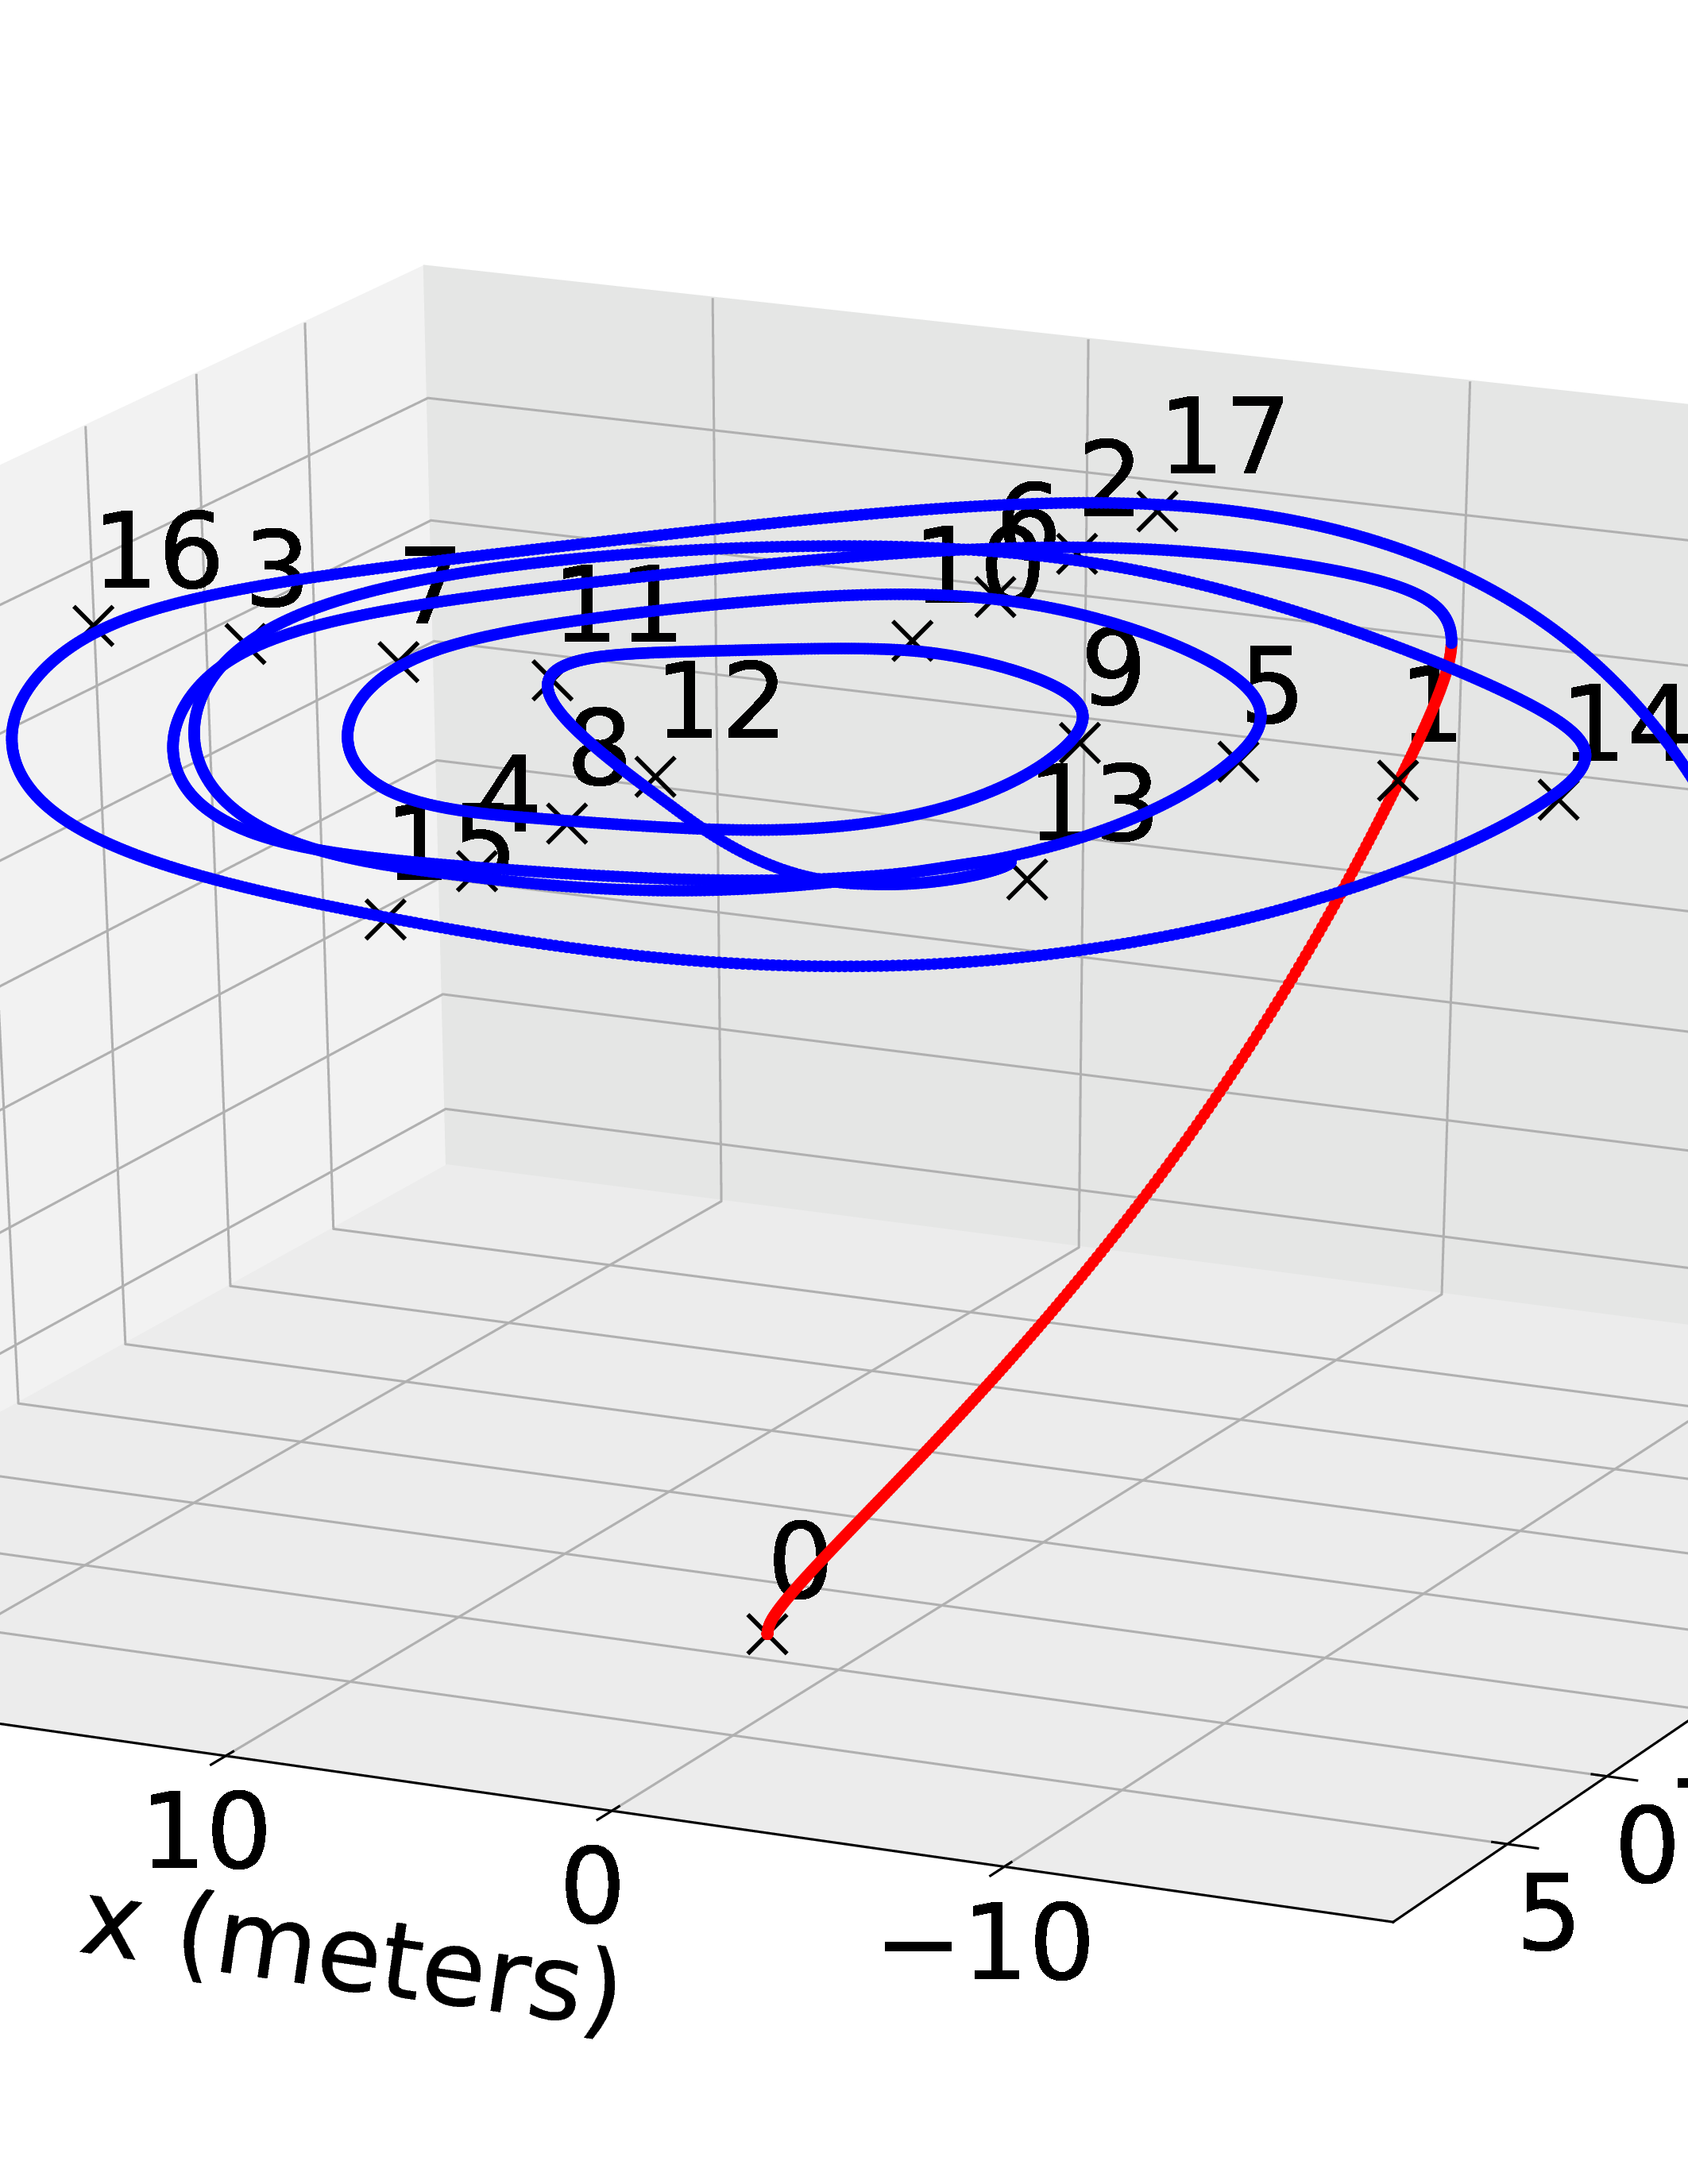}
\includegraphics[width=0.49\linewidth]{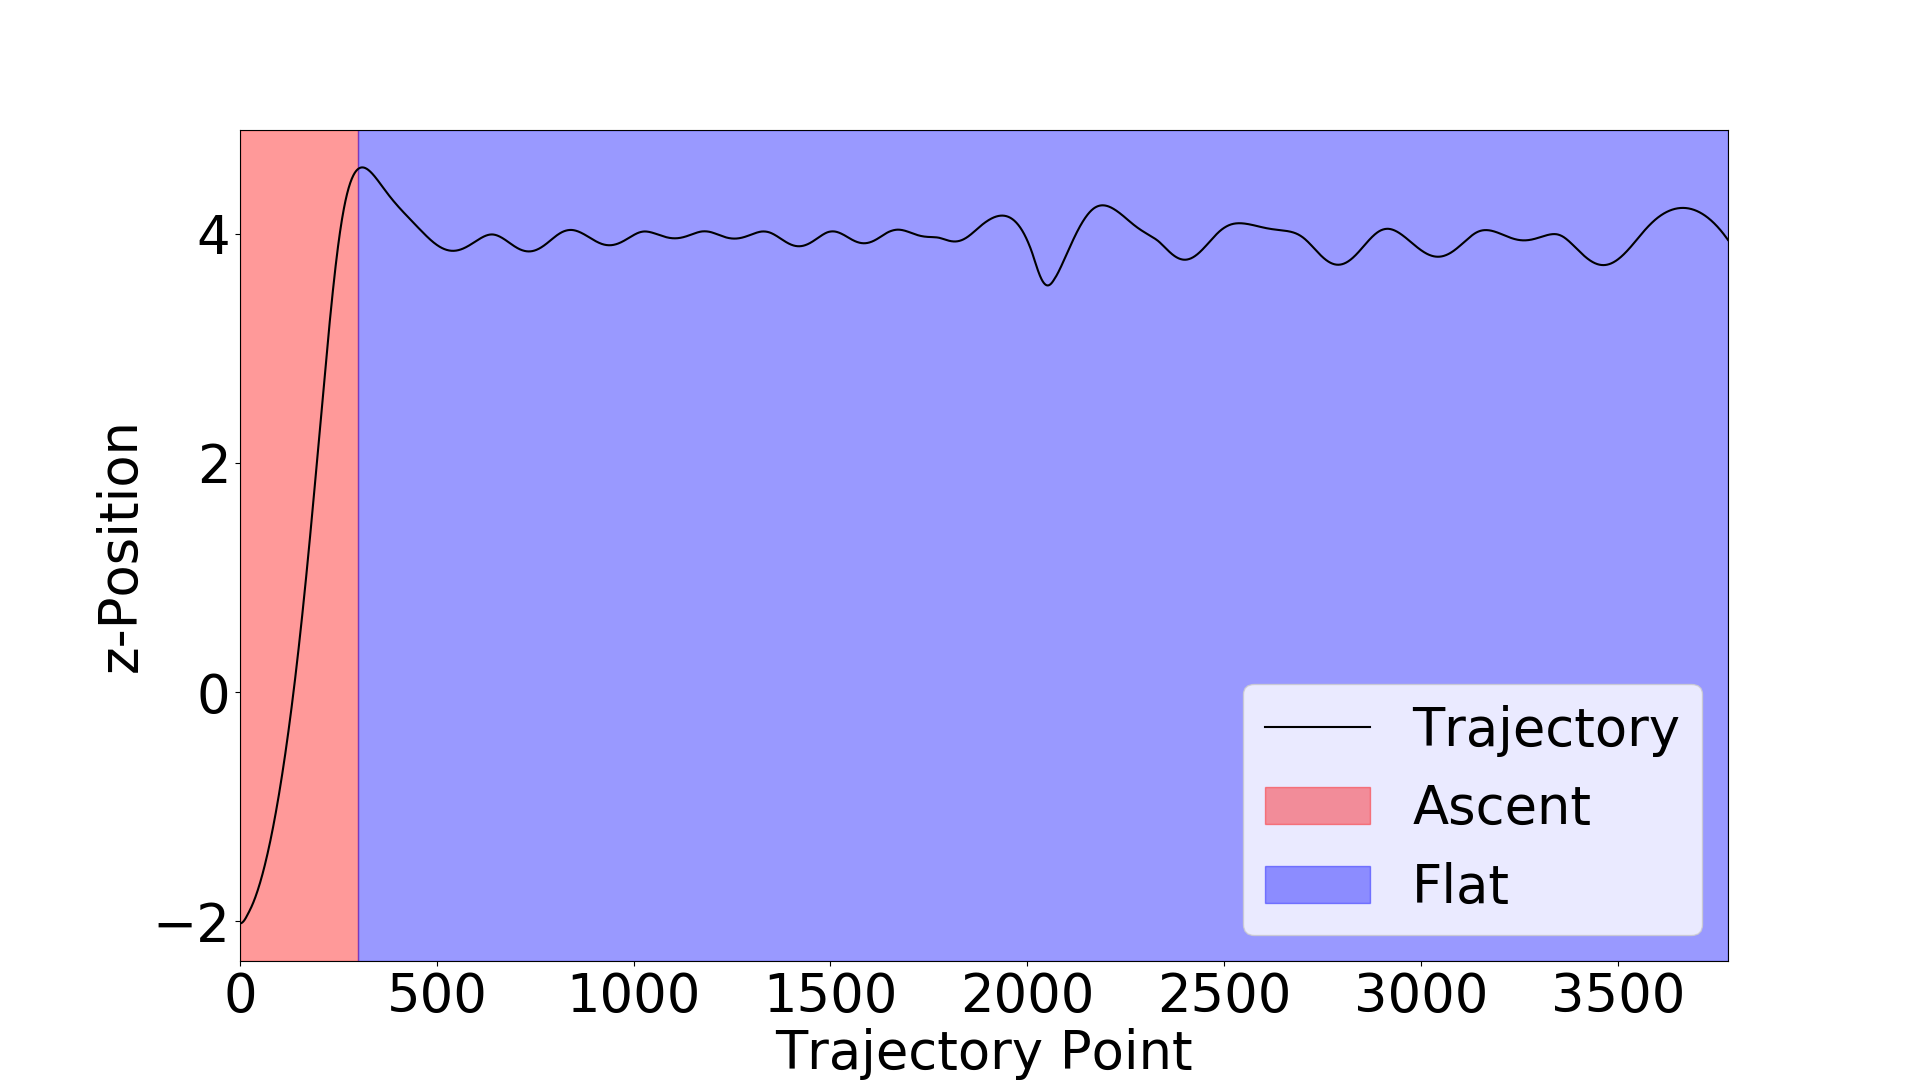}
\captionof{figure}{Spiral track.}
\label{fig:appendix_spiral}

\includegraphics[width=0.49\linewidth]{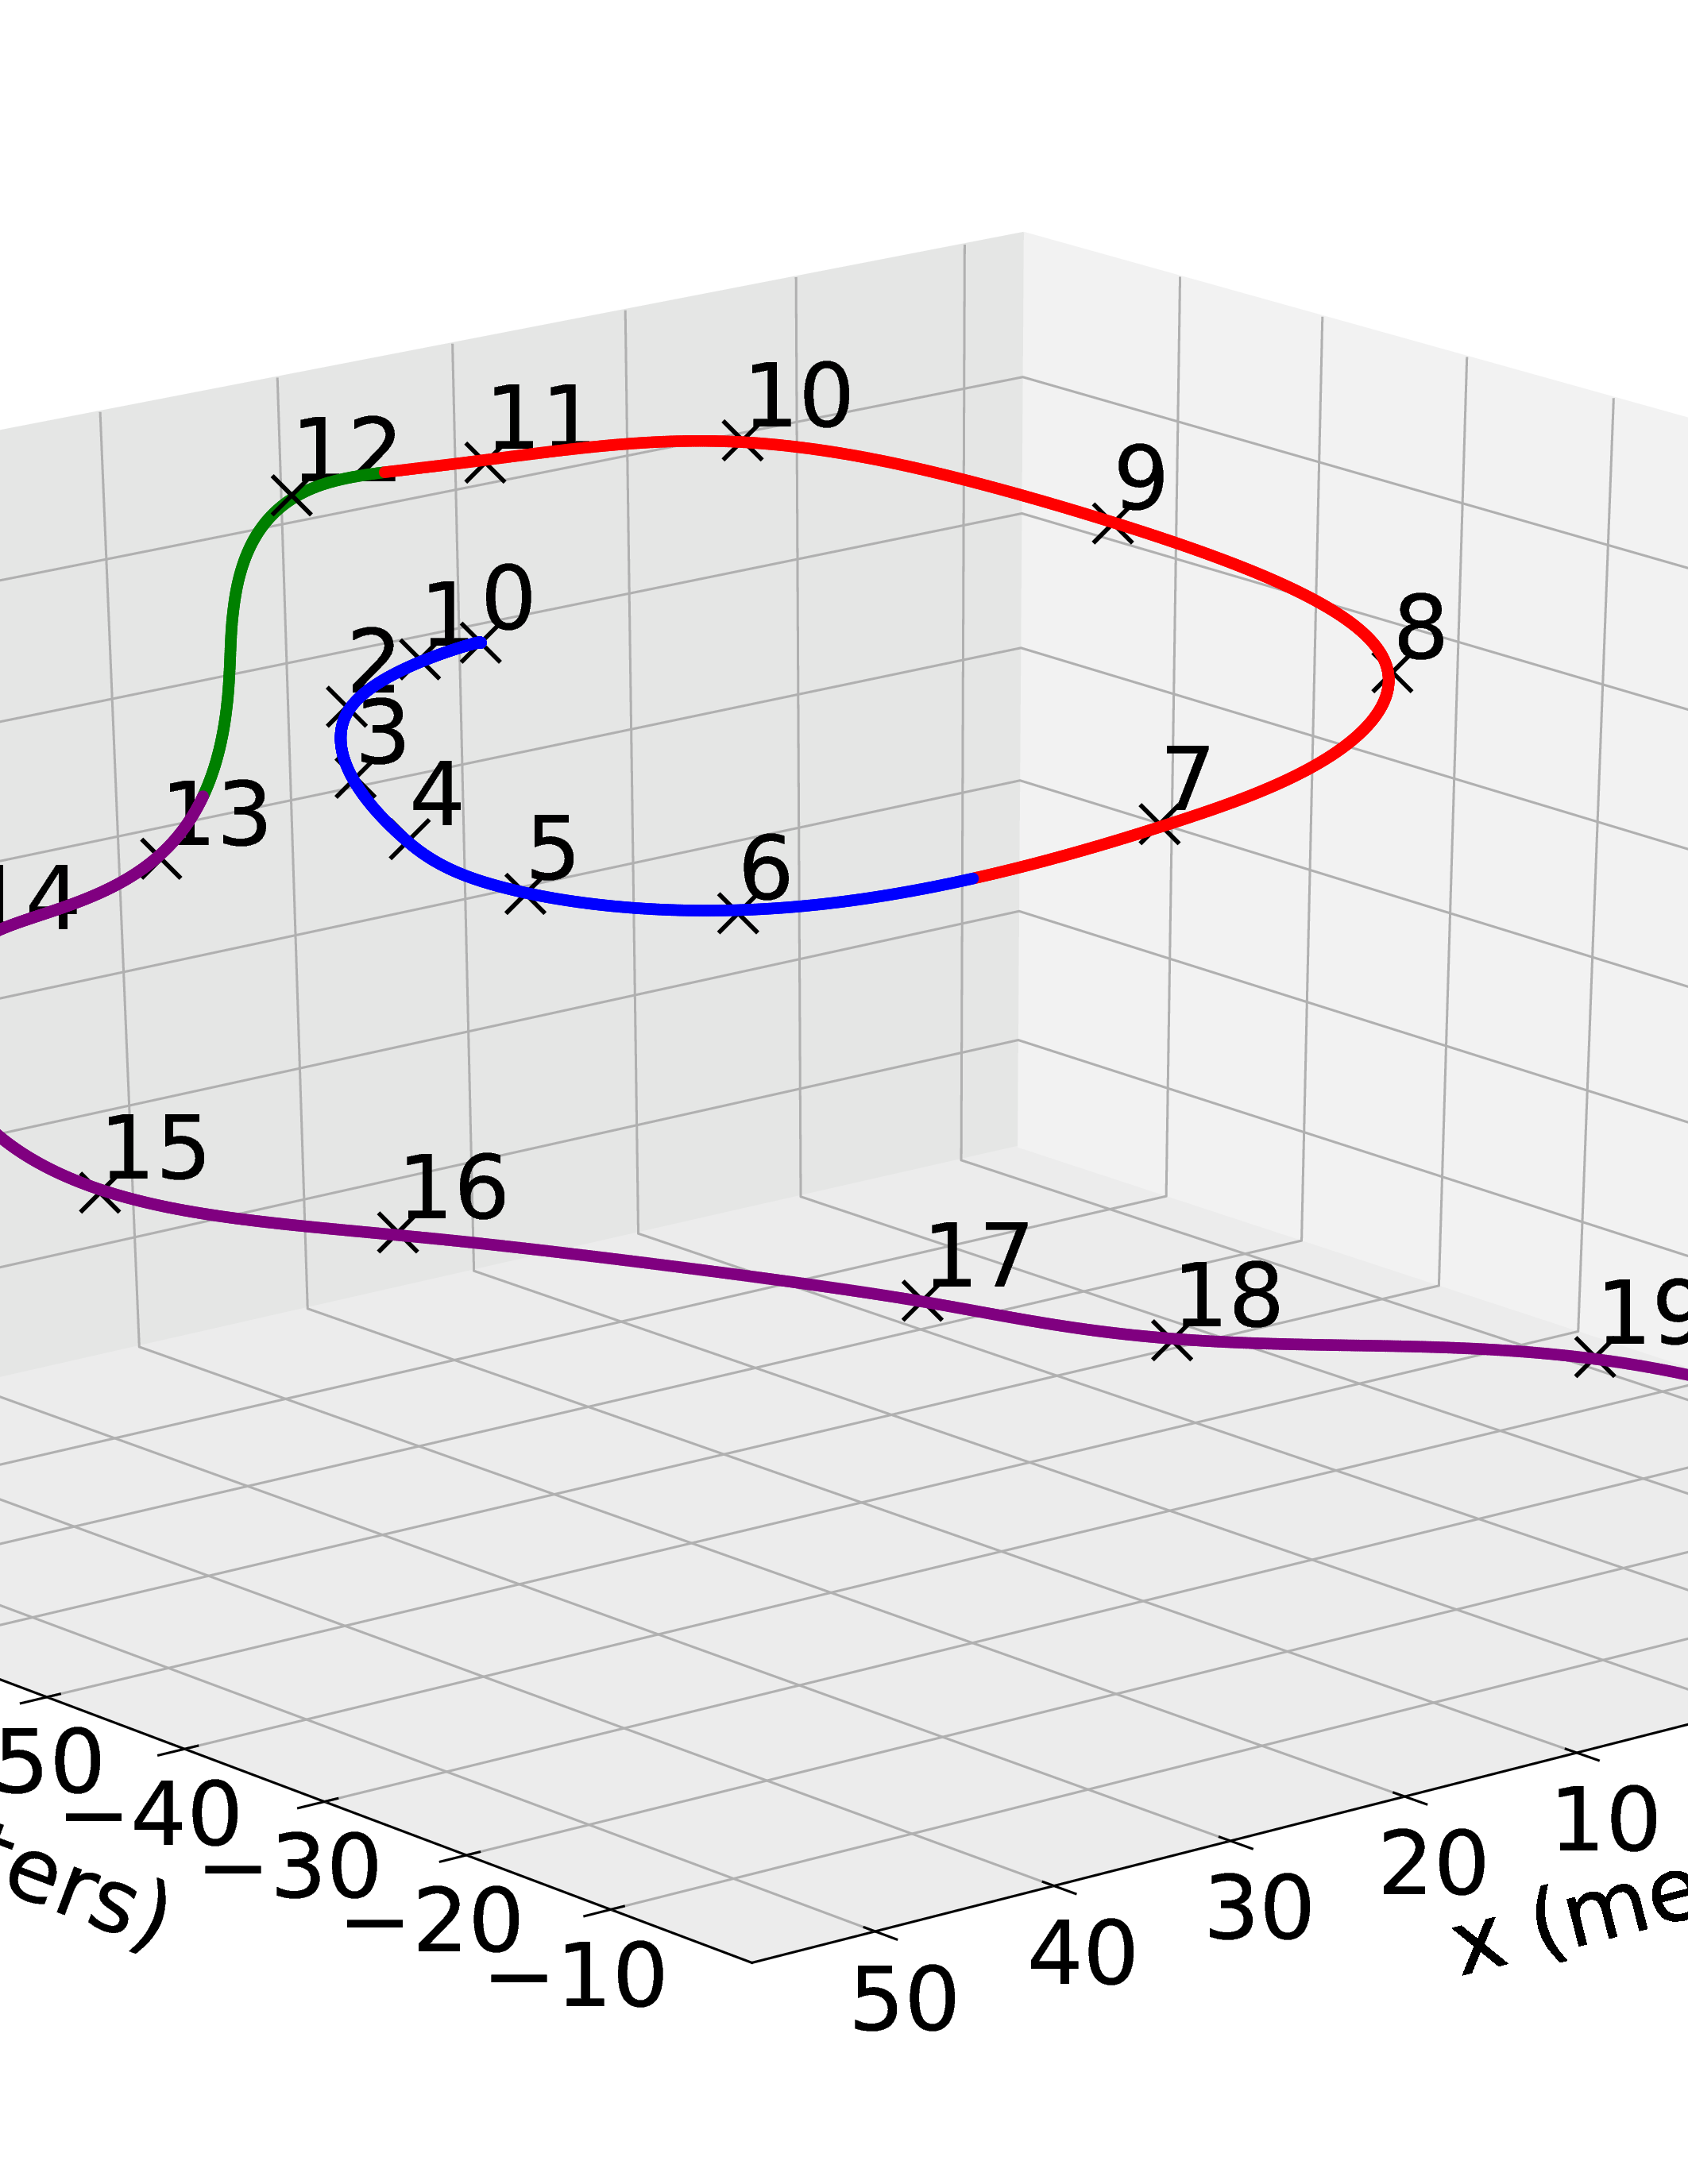}
\includegraphics[width=0.49\linewidth]{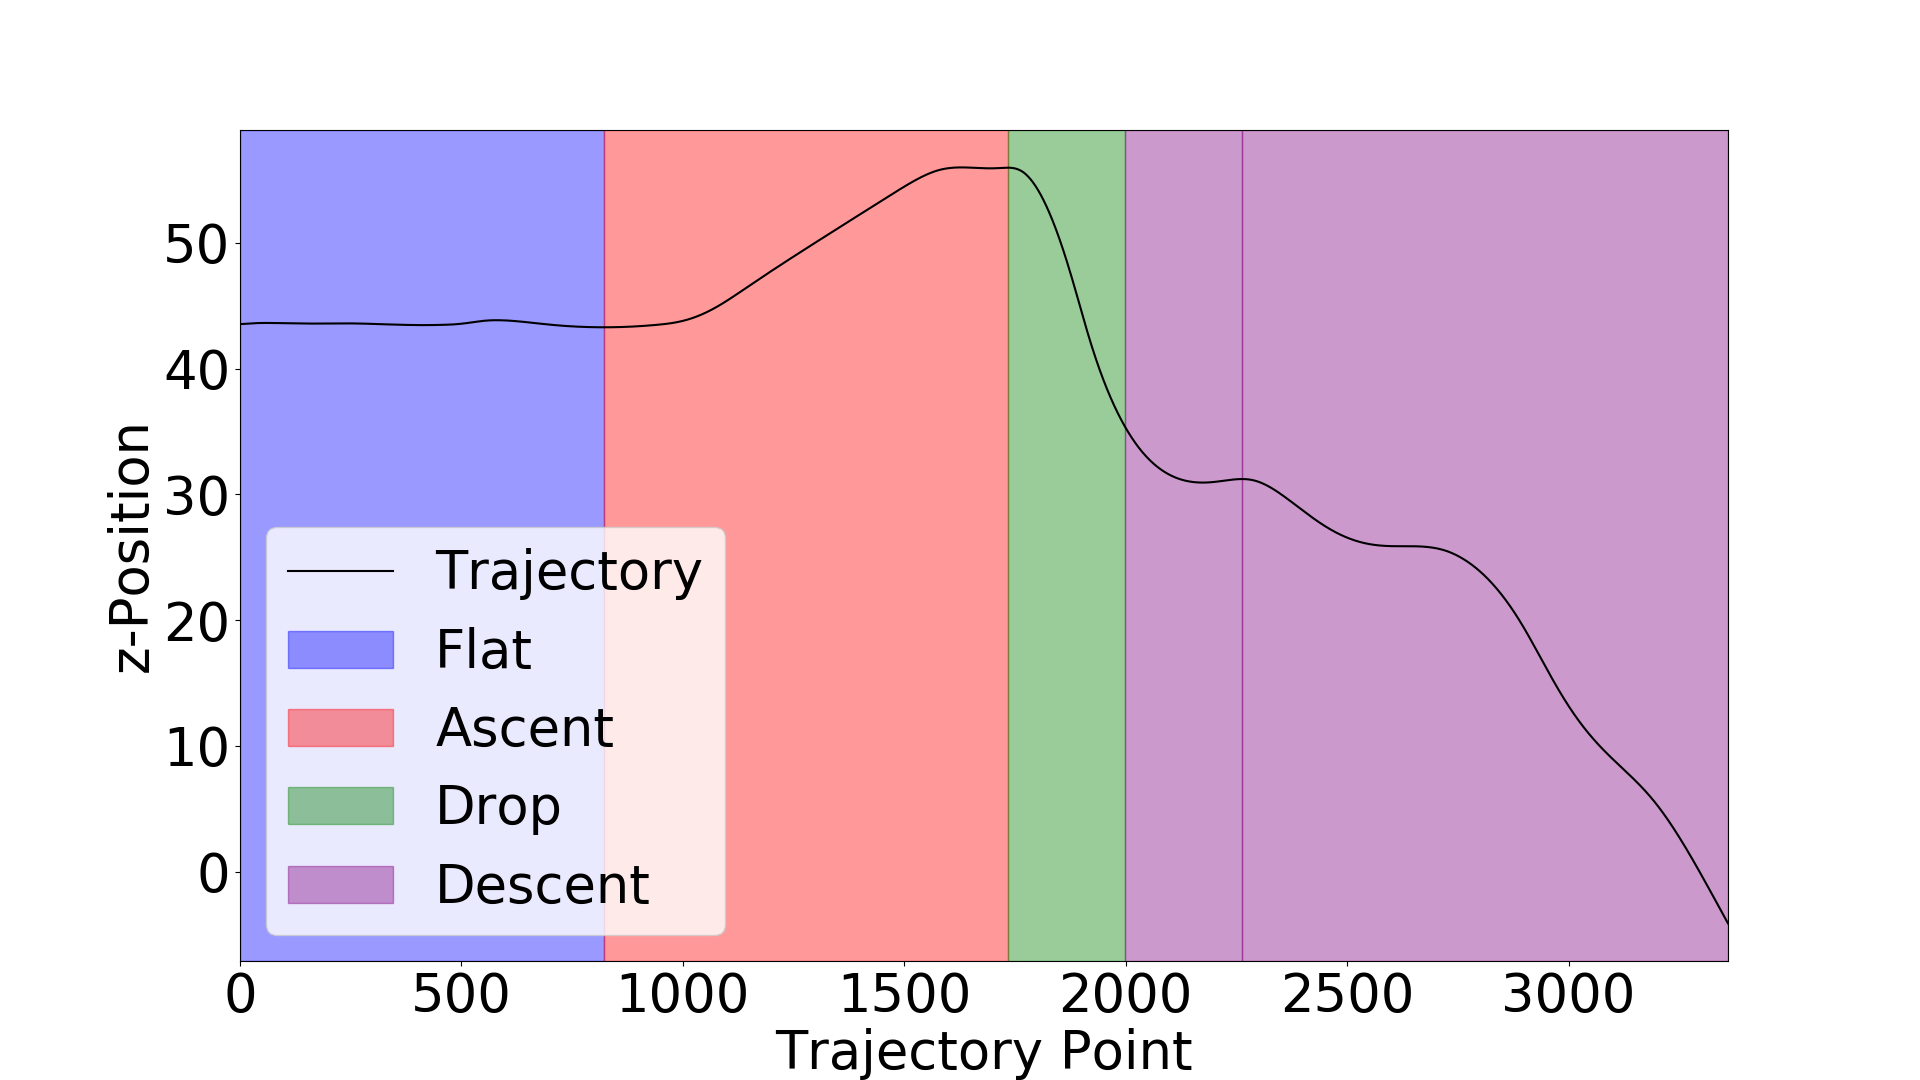}
\captionof{figure}{Qualifier track.}
\label{fig:appendix_qualifier}

\includegraphics[width=0.49\linewidth]{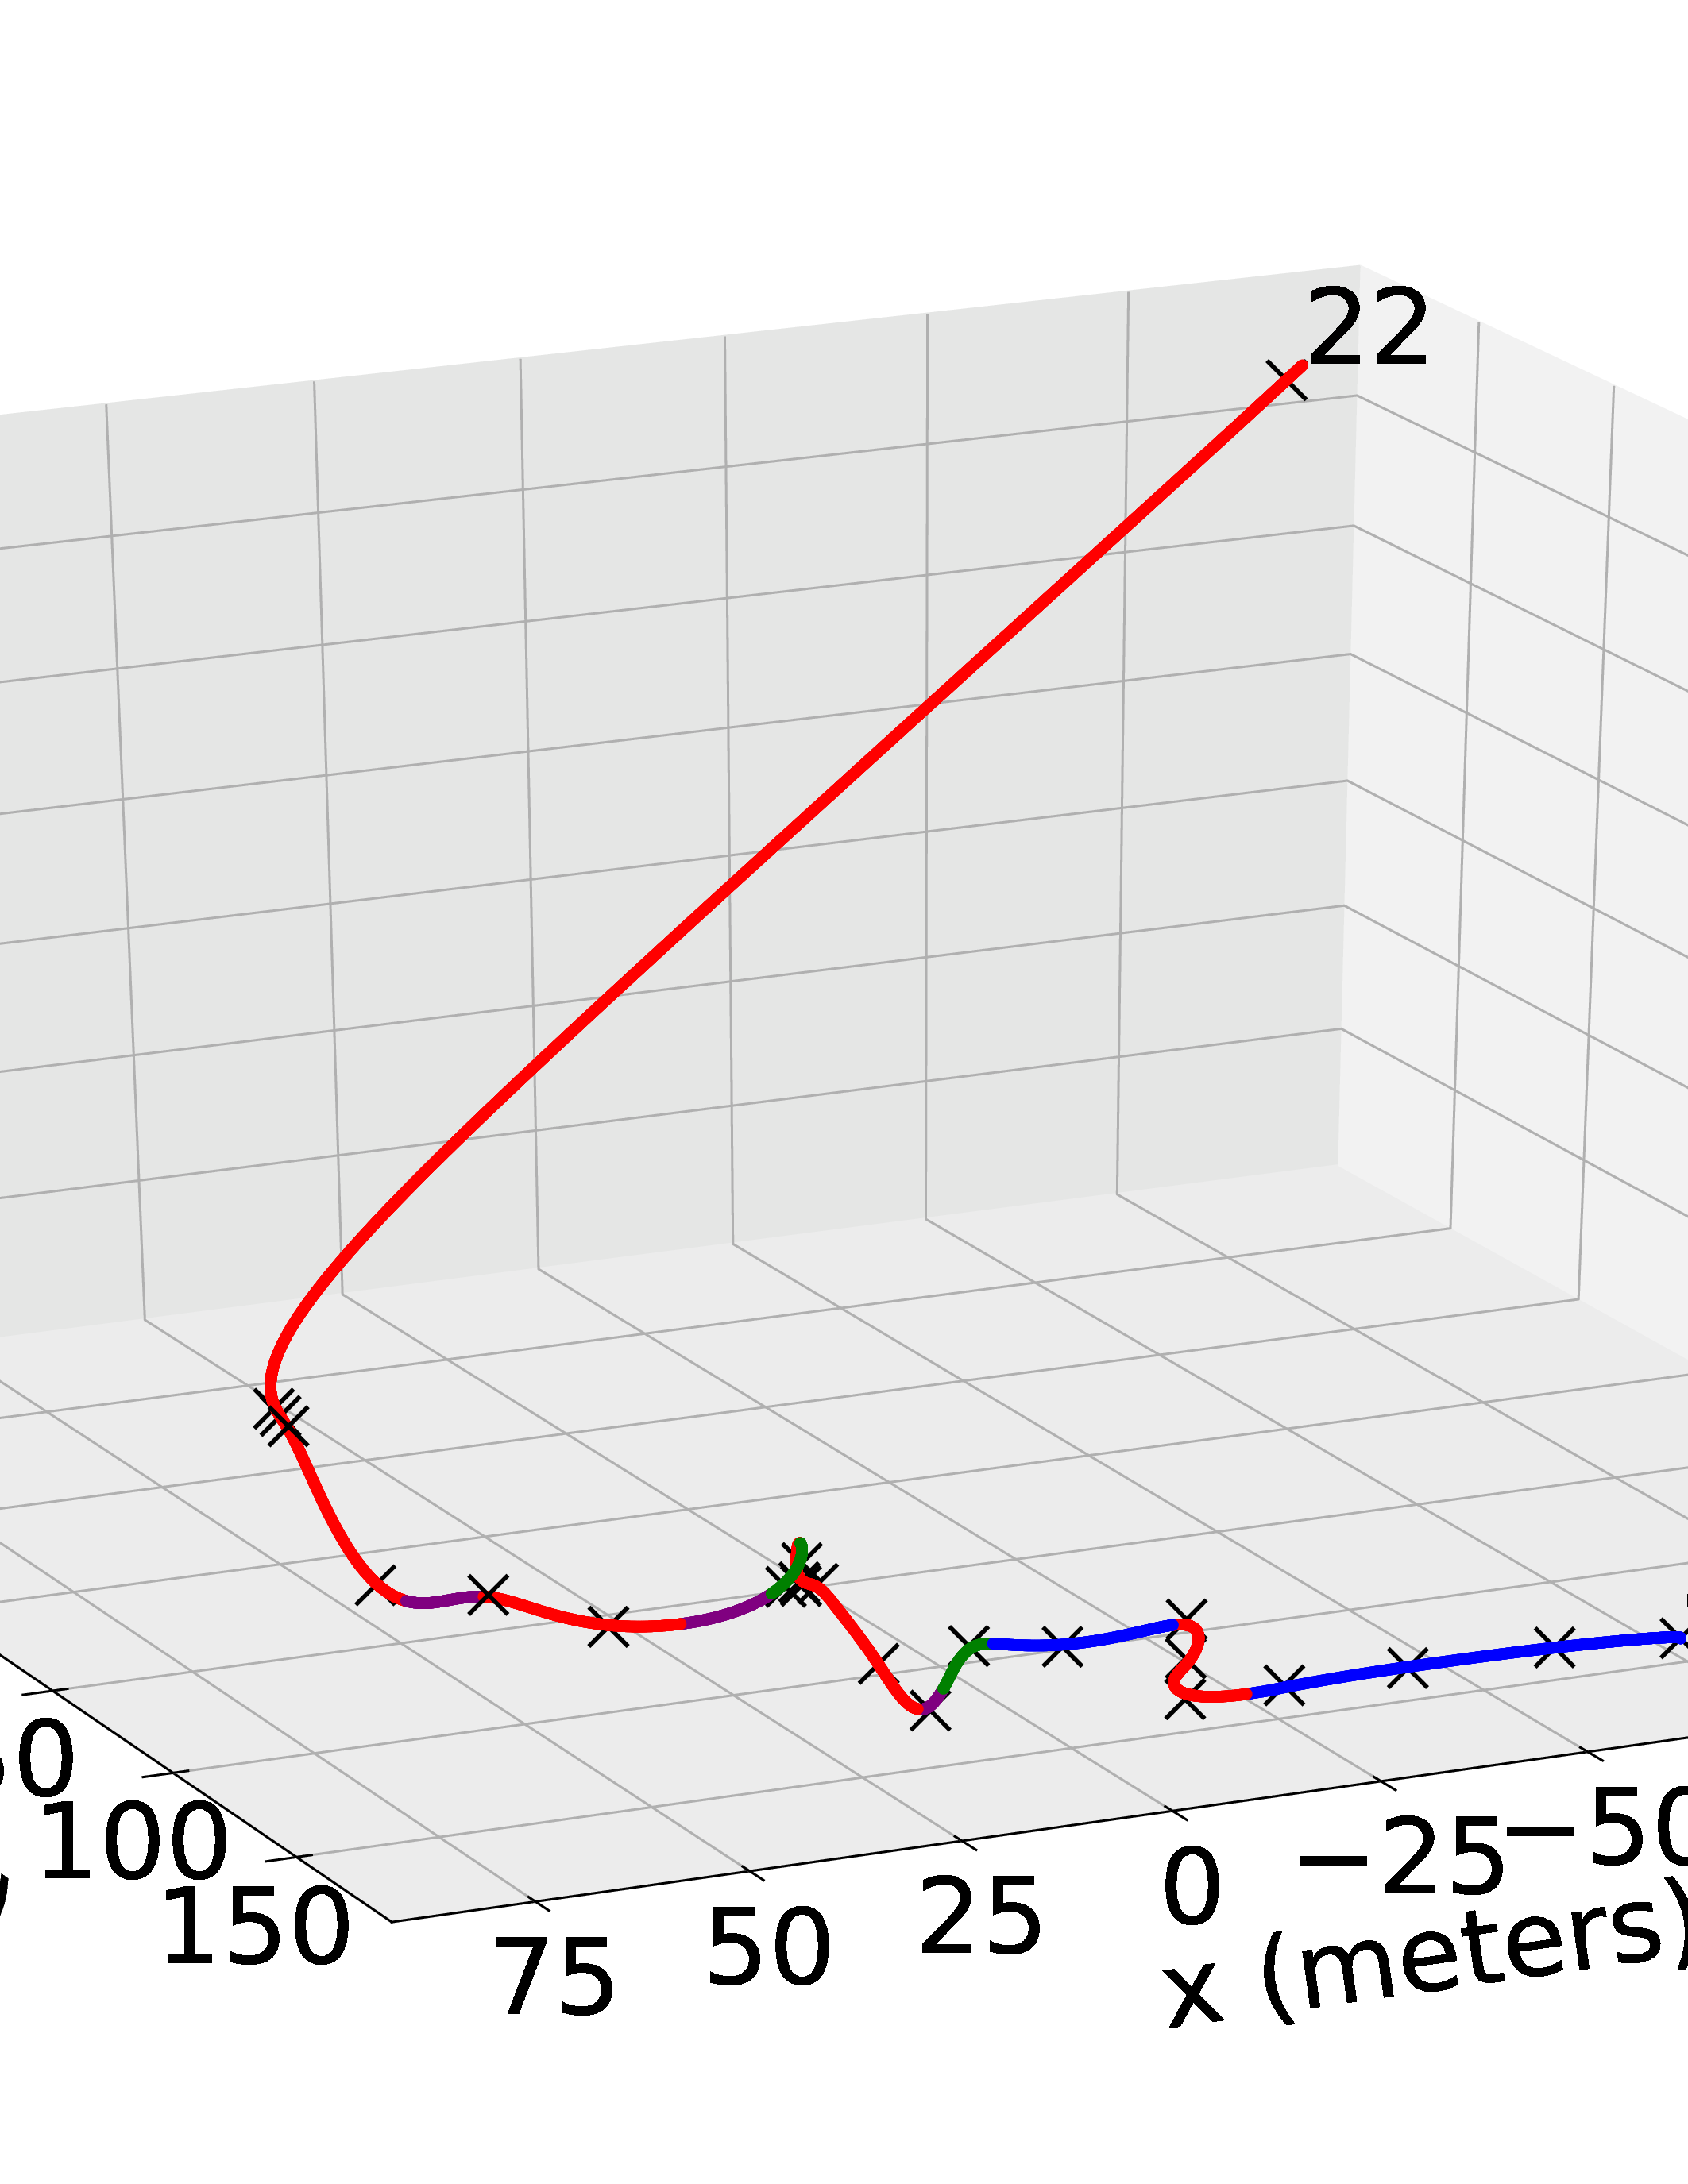}
\includegraphics[width=0.49\linewidth]{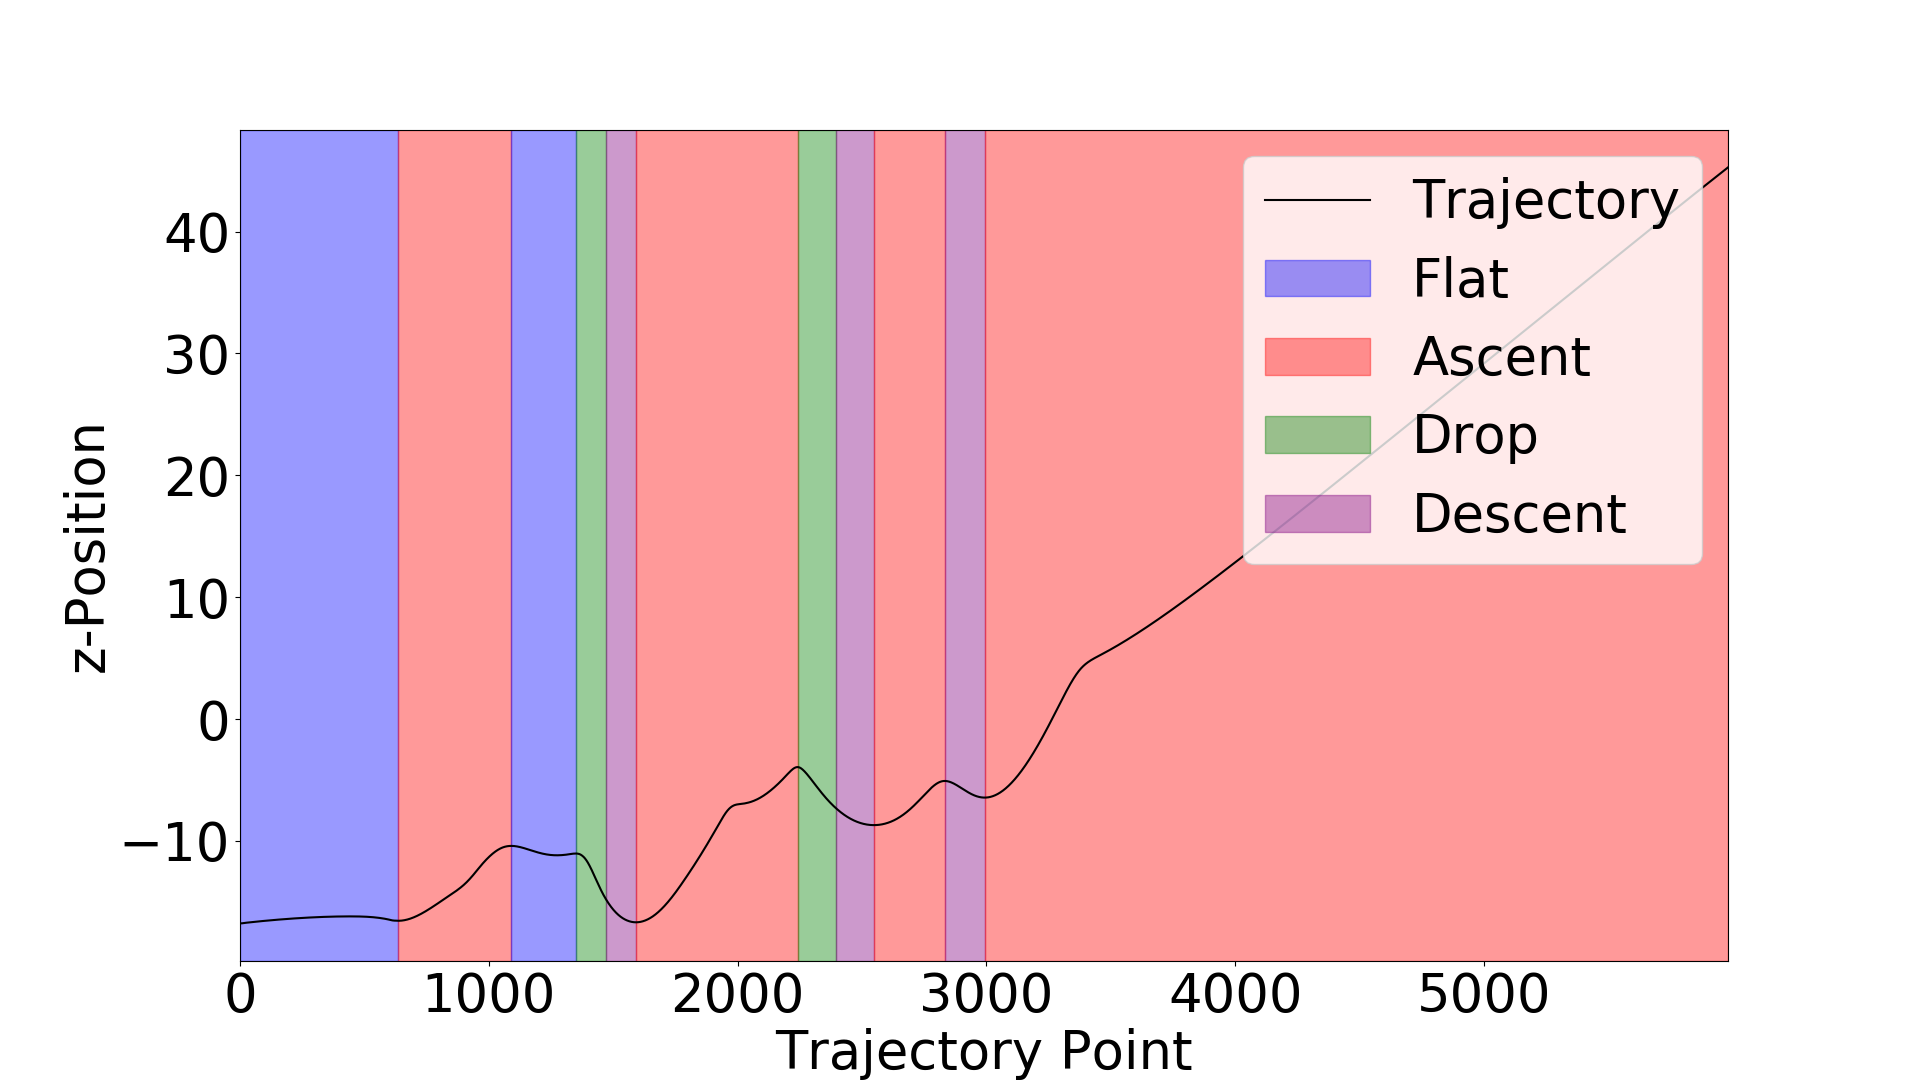}
\captionof{figure}{Final track.}
\label{fig:appendix_final}

\includegraphics[width=0.49\linewidth]{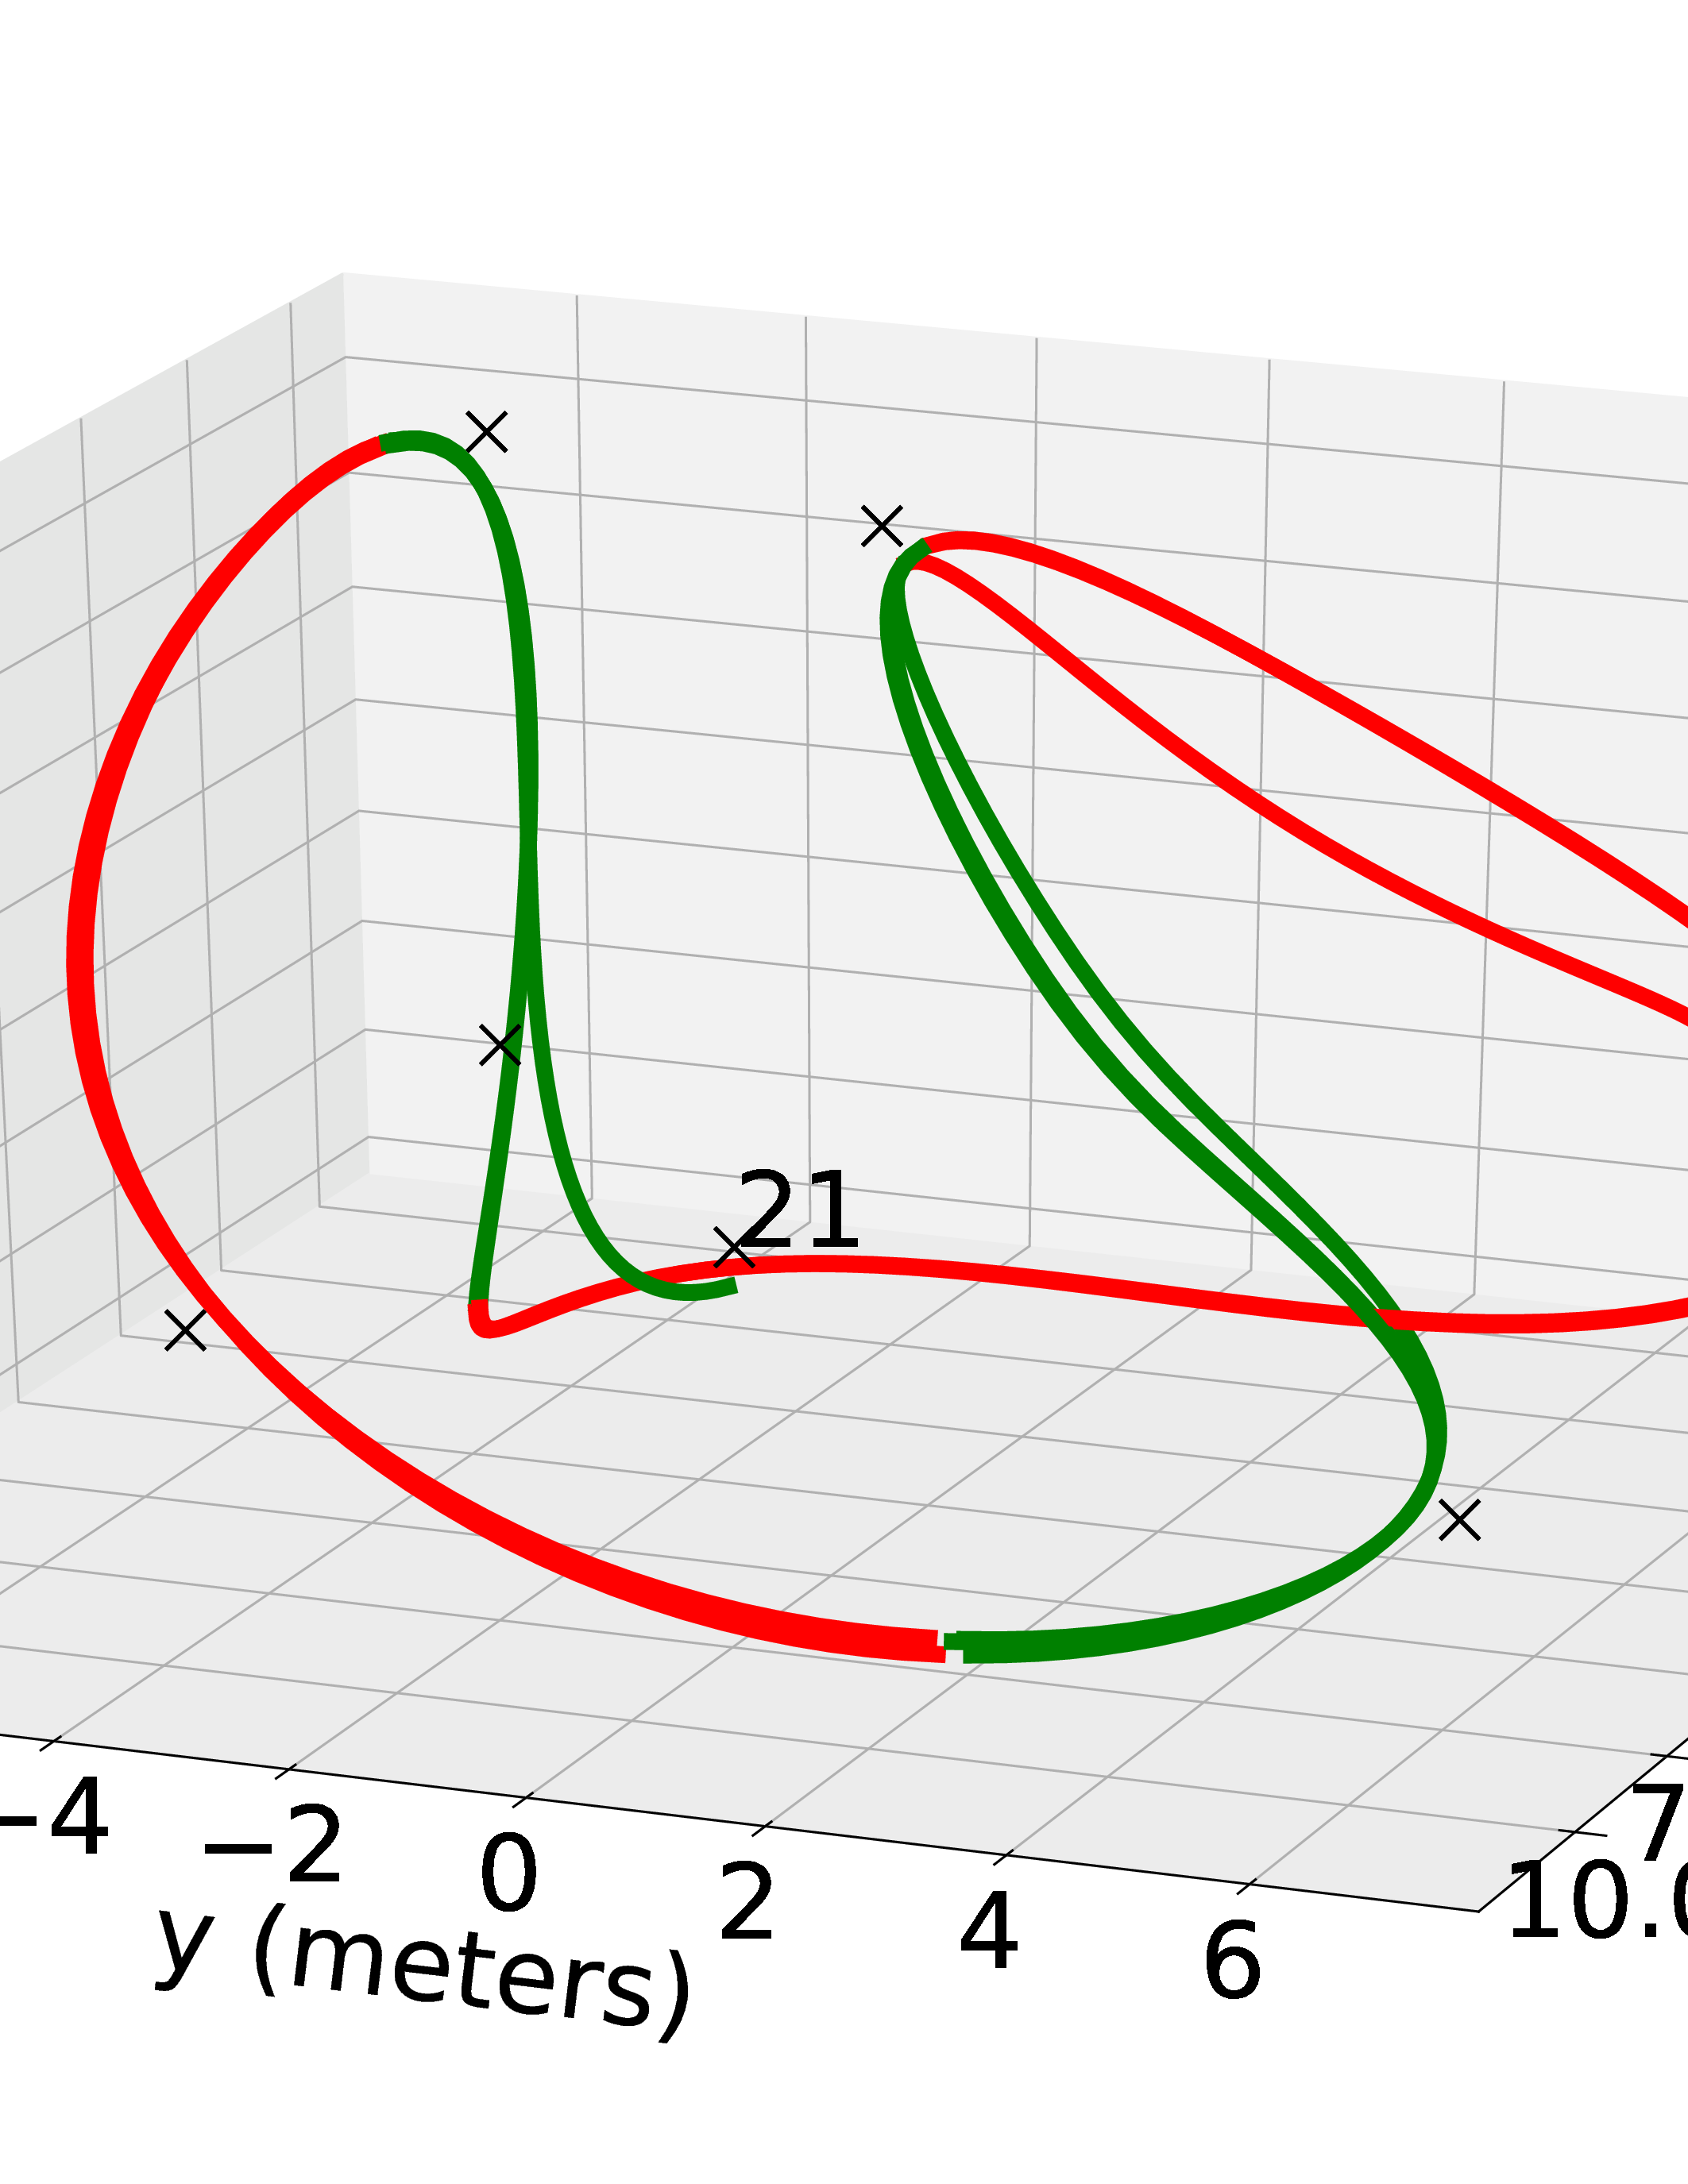}
\includegraphics[width=0.49\linewidth]{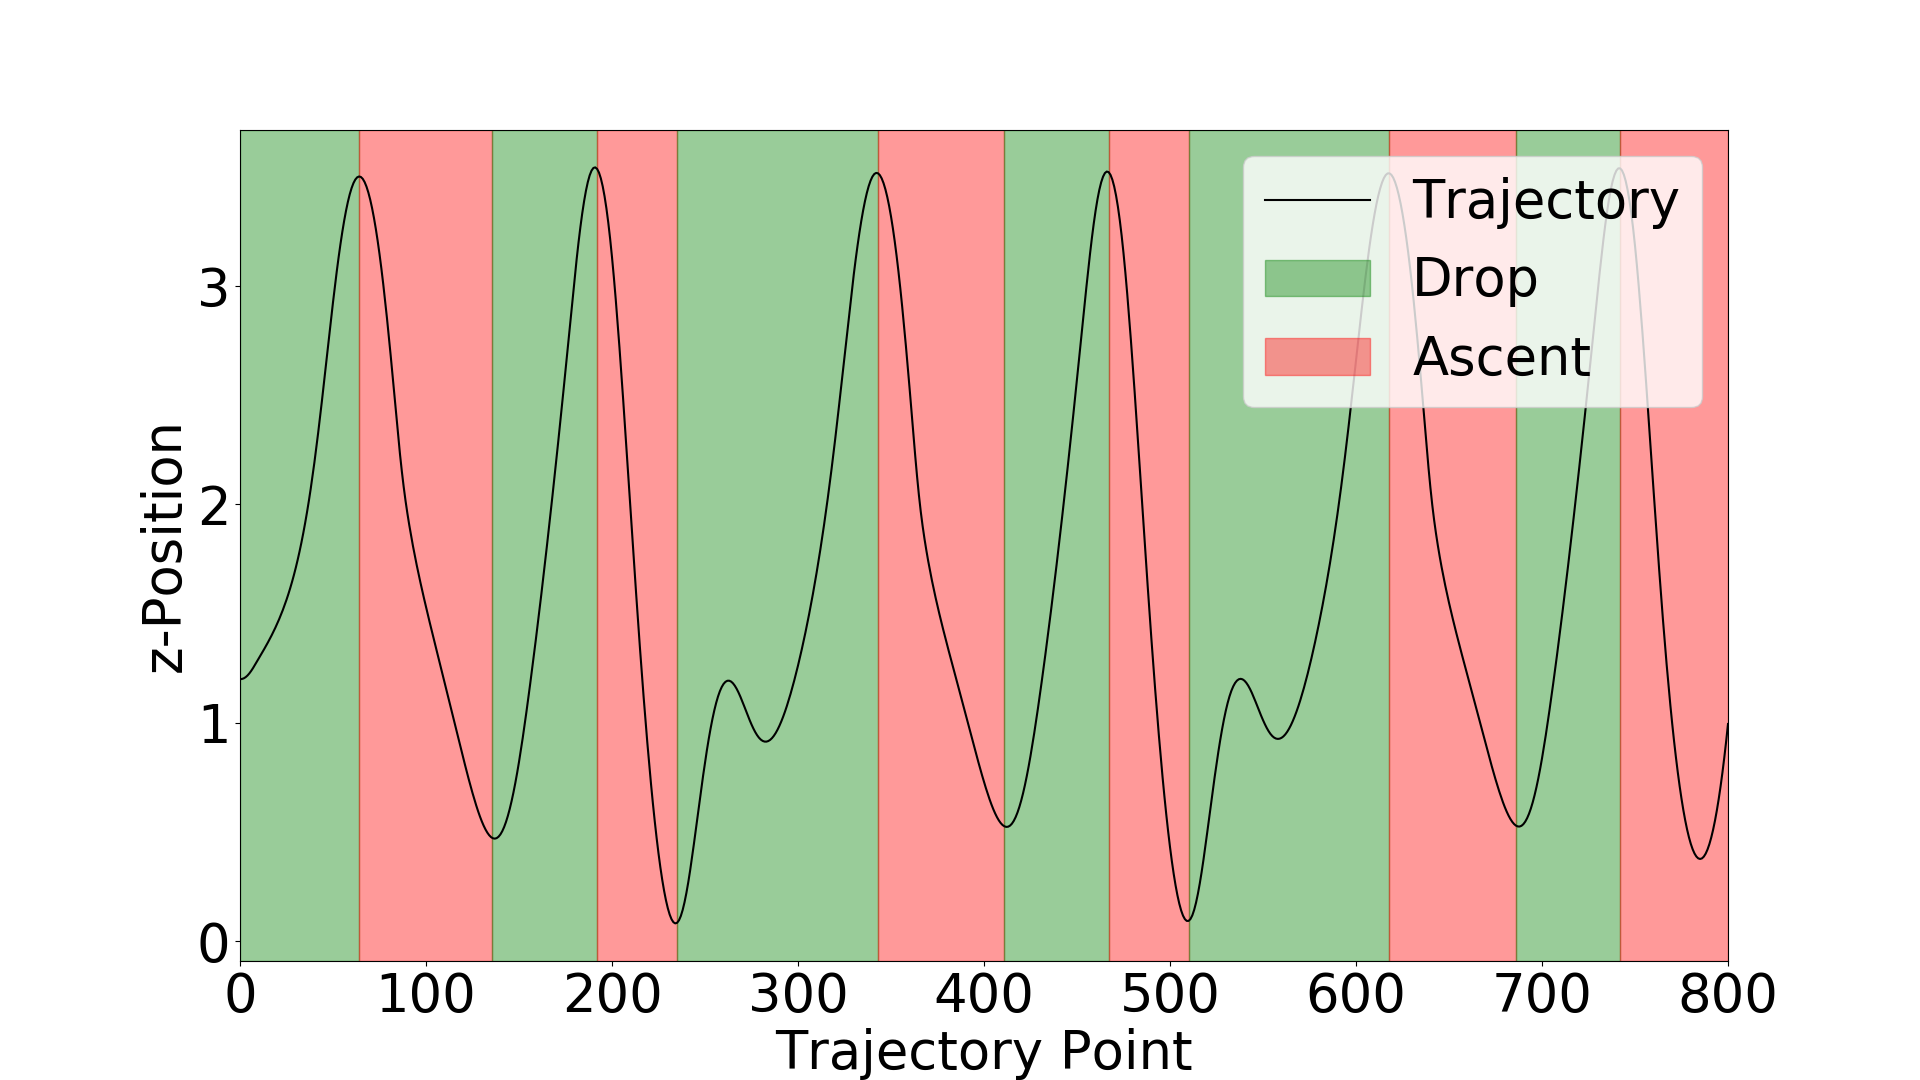}
\captionof{figure}{SplitS track.}
\label{fig:appendix_real}
\end{center}

Specifically, we select the following maneuvers:
\begin{itemize}
    \item Circle: 2D maneuver with a radius of $r=\SI{16}{\meter}$. Consists of 12 waypoints at an average of \SI{9}{\meter} distance.
    \item Drop: Ascent of $\SI{21}{\meter}$ in z over $\SI{50}{\meter}$ length followed by a steep descent of $\SI{16}{\meter}$ in height. Ends with a semi-circle with radius $r=\SI{16}{\meter}$. Consists of 12 waypoints at an average of \SI{10}{\meter} distance.
    \item Flip: Ascent of $\SI{25}{\meter}$ in z over $\SI{117}{\meter}$ length, with an half-loop in z of $\SI{14}{\meter}$ radius. Ends with a steep descent of $r=\SI{20}{\meter}$ over $\SI{28}{\meter}$ length. Consists of 12 waypoints at an average of \SI{13}{\meter} distance.
    \item Spiral: Ascent of $\SI{6}{\meter}$ followed by a spiral made of three planar circles of $30$, $22$, and $16$ meters in the clockwise direction followed by a half a circle with radius $r=\SI{6}{\meter}$. Then the drone follows two planar circles of $30$ and $38$ meters in a counter-clockwise direction. Consists of 17 waypoints at an average of \SI{13}{\meter} distance.
    \item Qualifier: Track used for the qualification round of the 2019 AirSim Game of Drones competition. Made of an ascending circle of $\SI{160}{\meter}$, a $\SI{23}{\meter}$ drop in height over $\SI{25}{\meter}$ length and a long straight descent of $\SI{148}{\meter}$ length. Consists of 20 waypoints at an average of \SI{16}{\meter} distance.
    \item Final: Track used for the final round of the 2019 AirSim Game of Drones competition. Made of a $\SI{209}{\meter}$ long segment with a hairpin and loop, followed by a $\SI{40}{\meter}$ ascent over approximately $\SI{296}{\meter}$. Consists of 22 waypoints at an average of \SI{22}{\meter} distance.
\end{itemize}
Eventually, in the real world we fly an aggressive trajectory, that we call SplitS, composed of 21 waypoints with abrupt changes in the flight direction and speeds in the range $8-15\SI{}{\meter\per\second}$. The SplitS trajectory consists of a sequence of ascents and drops of $\SI{3}{\meter}$ in height repeated three times.
The trajectories of these maneuvers are illustrated in Section~\ref{app:tracks}.
All maneuvers start and end in the hover condition.

\subsection{Training Data and Feature Selection}

The training data consists of $14$ time-optimal trajectories, each annotated with a set of parameters that allows the controller to successfully track the trajectory.
In total, the training trajectories are divided into $73$ segments: $13$ flat, $22$ ascent, $23$ descent, and $15$ steep.
\rebuttal{For each segment type, we train a Gradient Boosting regressor on the relative data with default parameters}. We extract five features from each segment, namely the number of points in the segment, the slope of the line connecting the first and last point of the segment, as well as their difference in height, and the mean velocity and acceleration.
These features were selected with a cross-validation procedure over a wider set of features. Specifically, during the selection process we considered the following features: the number of points in the segment, the slope of the line connecting the first and last point of the segment, as well as their difference in height, velocity and acceleration, and the minimum, the mean and the maximum velocity and acceleration.
We evaluated each feature combination by predicting the controller initial parameters on the qualifier track and then by computing the root-mean-square error (RMSE) of the predicted parameters with respect to the optimal parameters in the training data.
Finally, we selected the feature combination that minimized the RMSE.

\subsection{Implementation Choices} \label{subsec:implementation_choices}

\rebuttal{We use the MPC formulation of Falanga~\cite{Falanga2018}, without perception constraints, and the time-optimal planner described by Foehn~\cite{Foehn2020}.
We use the AirSim SimpleFlight quadrotor configuration. The quadrotor weights $1.0$ kg and can generate thrust to weight ratio up to $4.179$.
We choose the MPC control frequency to be $200$ Hz with horizon step $0.05$.
Rather than optimize over the entire optimization landscape, we fix some parameters of the controller to obtain a reduced, but representative, subspace.
In particular, we tune the MPC state costs (Q\_pos\_xy, Q\_pos\_z, Q\_attitude, Q\_velocity) and the horizon length, while we fix the MPC input costs (R\_thrust, R\_pitchroll, R\_yaw) to $1.0$, which we experimentally saw to be not very important to performance.
Moreover, we bound the inputs to match the limits of the simulator, by fixing the maximum pitch-roll to $10.0$ rad/s, the maximum yaw to $3.0$ rad/s and the maximum thrust to $20.0$ N.
The same drone specifics are also used by the time-optimal planner.

We use a Gaussian distribution as proposal function for Metropolis-Hastings algorithm. The distribution is centered on the last set of parameters accepted and has variance $5$, which we empirically found to be effective for our task.
At each iteration, the M-H algorithm proposes a new set of parameters by sampling them from the Gaussian distribution.
When updating the parameters of a segment, the variance of the preceding segments is reduced by $25\%$.
This maintains global optimality but makes the controller close to the previous solution in the preceding segments.
We use $e^{-2\sqrt{t}}$, where $t$ is the lap time with added penalty for missed waypoints, as cost function for the M-H algorithm.
}

% \begin{figure*}
%     \centering
%     \setlength{\tabcolsep}{0pt}
%     \begin{tabular}{ccc}
%     \resizebox{0.33\linewidth}{!}{\input{images/tickzfiles/mean}} &
%     \resizebox{0.33\linewidth}{!}{\input{images/tickzfiles/max}} &
%     \resizebox{0.33\linewidth}{!}{\input{images/tickzfiles/error}} \\
%       (a) &
%       (b) &
%       (c) \\
%     \end{tabular}
%     \caption{Results in the real world. After tuning the parameters in simulation, we evaluate the best configuration found by AutoTune on a physical platform. We compare the performance with the controller default parameters. We perform three runs and report the statistics of the mean (a) and max (b) tracking error. We also report the error as a function of time (c) for the best run of our and the default setting. AutoTune consistently improves performance while decreasing the variance between runs.}
%     \label{fig:auto_rw}
% \end{figure*}

\subsection{Choosing Trajectory Segmentation Conditions} \label{app:choosing_traj_segment}

\rebuttal{
Trajectory segmentation is fundamental for successfully tracking high-speed maneuvers. 
We split the trajectory into multiple segments according to the height gradient of the reference.
Specifically, we assign each point to the class \emph{flat}, \emph{ascent}, or \emph{descent} if the difference in height $g_z = z[k] - z[k+1]$ with its successor is $|g_z|<1m$.
The resulting segments are then clustered such that the minimum segment duration is $2$ seconds.
Eventually, all the descent and ascent segments with a slope higher than \SI{45}{\degree} are recursively split into two equal parts, where the first is assigned to the class \emph{steep} and the second remains assigned to the original class.

Since the segmentation conditions are crucial to the correct functioning of the proposed algorithm, we study its effects on the tracking performance.
Table~\ref{tab:choosing_traj_segment} reports the trajectory completion performance of the proposed algorithm on the Qualifier track. 
Each entry of the table is illustrated in Fig.~\ref{fig:choosing_traj_segment}.
The reported tracking performance is the best trajectory completion found by the proposed algorithm after $100$ iterations.

The results demonstrate the importance of choosing the right segmentation conditions.
By employing high thresholds on height difference and/or minimum duration, the trajectory segmentation method generates only one global segment, thus not allowing different controller behaviors along the track.
On the other hand, if the chosen thresholds are too little, then the proposed algorithm cannot find a suitable solution in the limited number of iterations.
Therefore, in future work we aim to build a parameter-free automatic segmentation procedure with change-point detection techniques generally used for time series \cite{aminikhanghahi2017KIS}.
}

\newpage

\begin{table}[t]
    \centering
    \begin{tabular}{c c c}
        \toprule
        Height Difference [m] & Min Duration [s] & Trajectory Completion [\%]\\
        \midrule
        1 & 2 & 100\\
        10 & 2 & 100\\
        20 & 2 & 65\\
        30 & 2 & 65\\
        1 & 1 & 60\\
        1 & 5 & 65\\
        \bottomrule
    \end{tabular}
    \caption{Effects of the trajectory segmentation conditions on the tracking performance. The track considered is Qualifier and the metric is the trajectory completion. We assign each point to the class \emph{flat}, \emph{ascent}, or \emph{descent} if the difference in height $g_z = z[k] - z[k+1]$ with its successor is $|g_z|<$\emph{Height Difference}. The resulting segments are then clustered such that the minimum segment duration is \emph{Min Duration} seconds.}
    \label{tab:choosing_traj_segment}
    \vspace{-3ex}
\end{table}

\begin{center}
\includegraphics[width=0.49\linewidth]{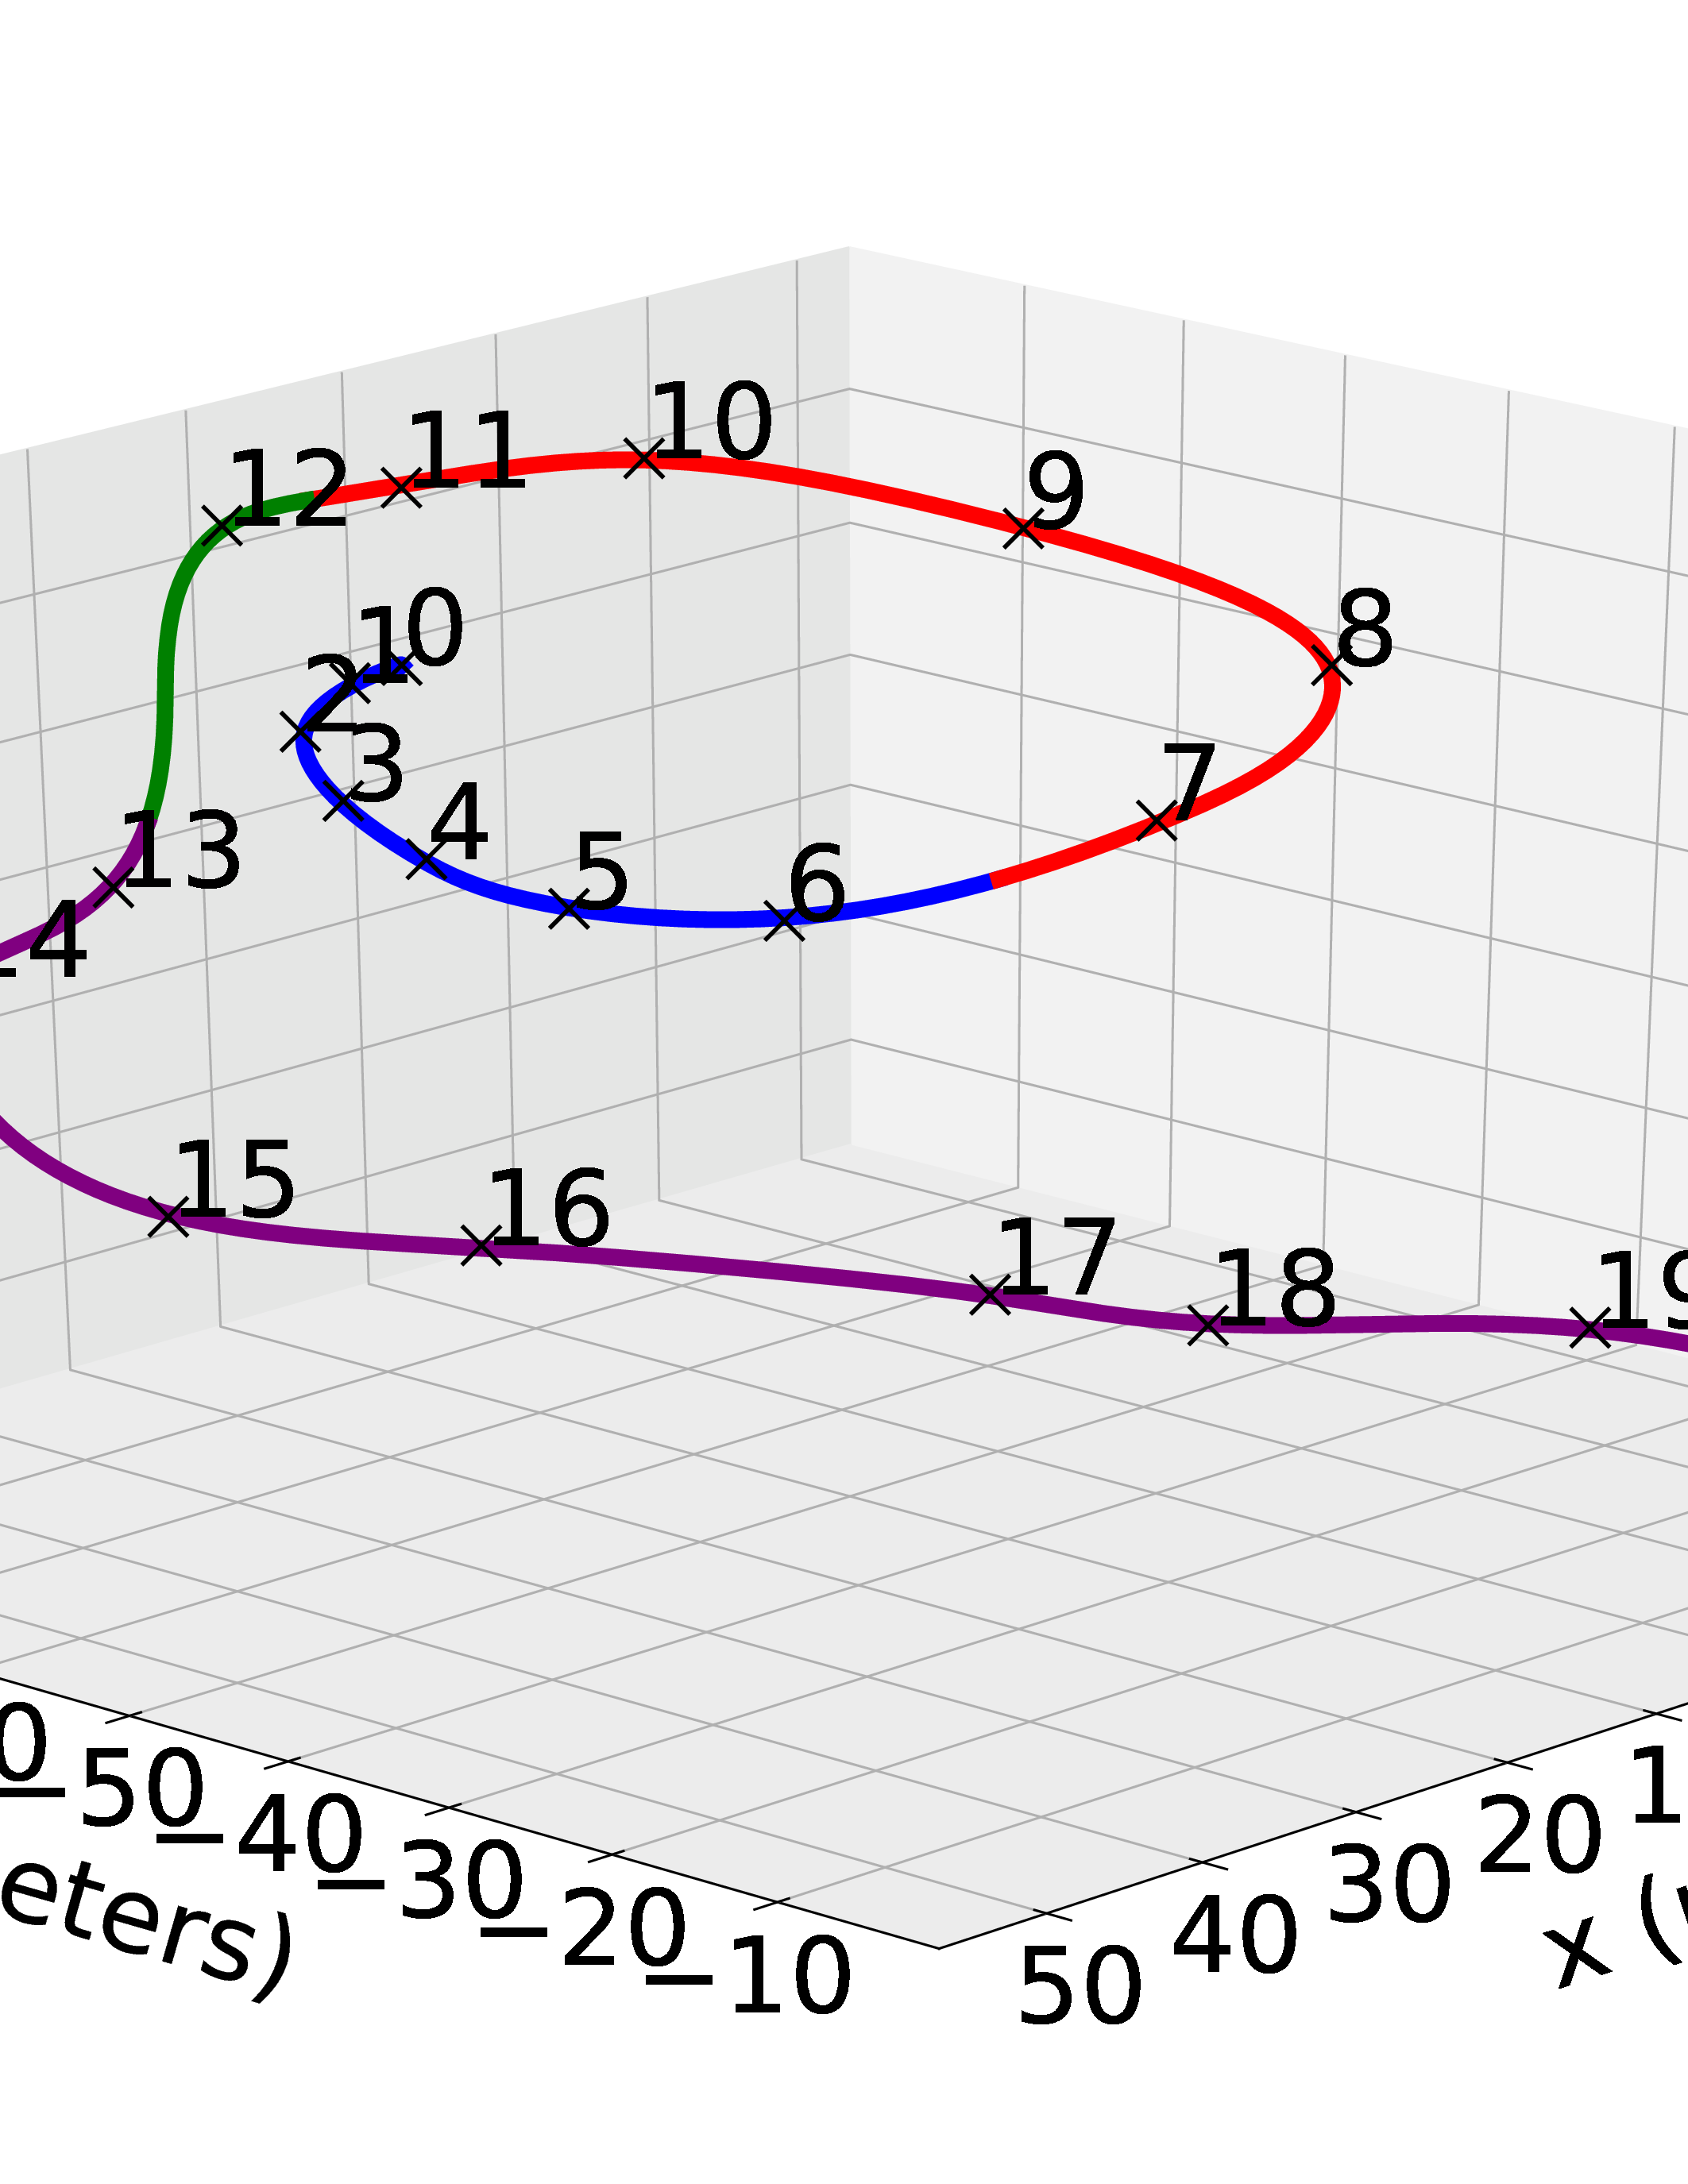}
\includegraphics[width=0.49\linewidth]{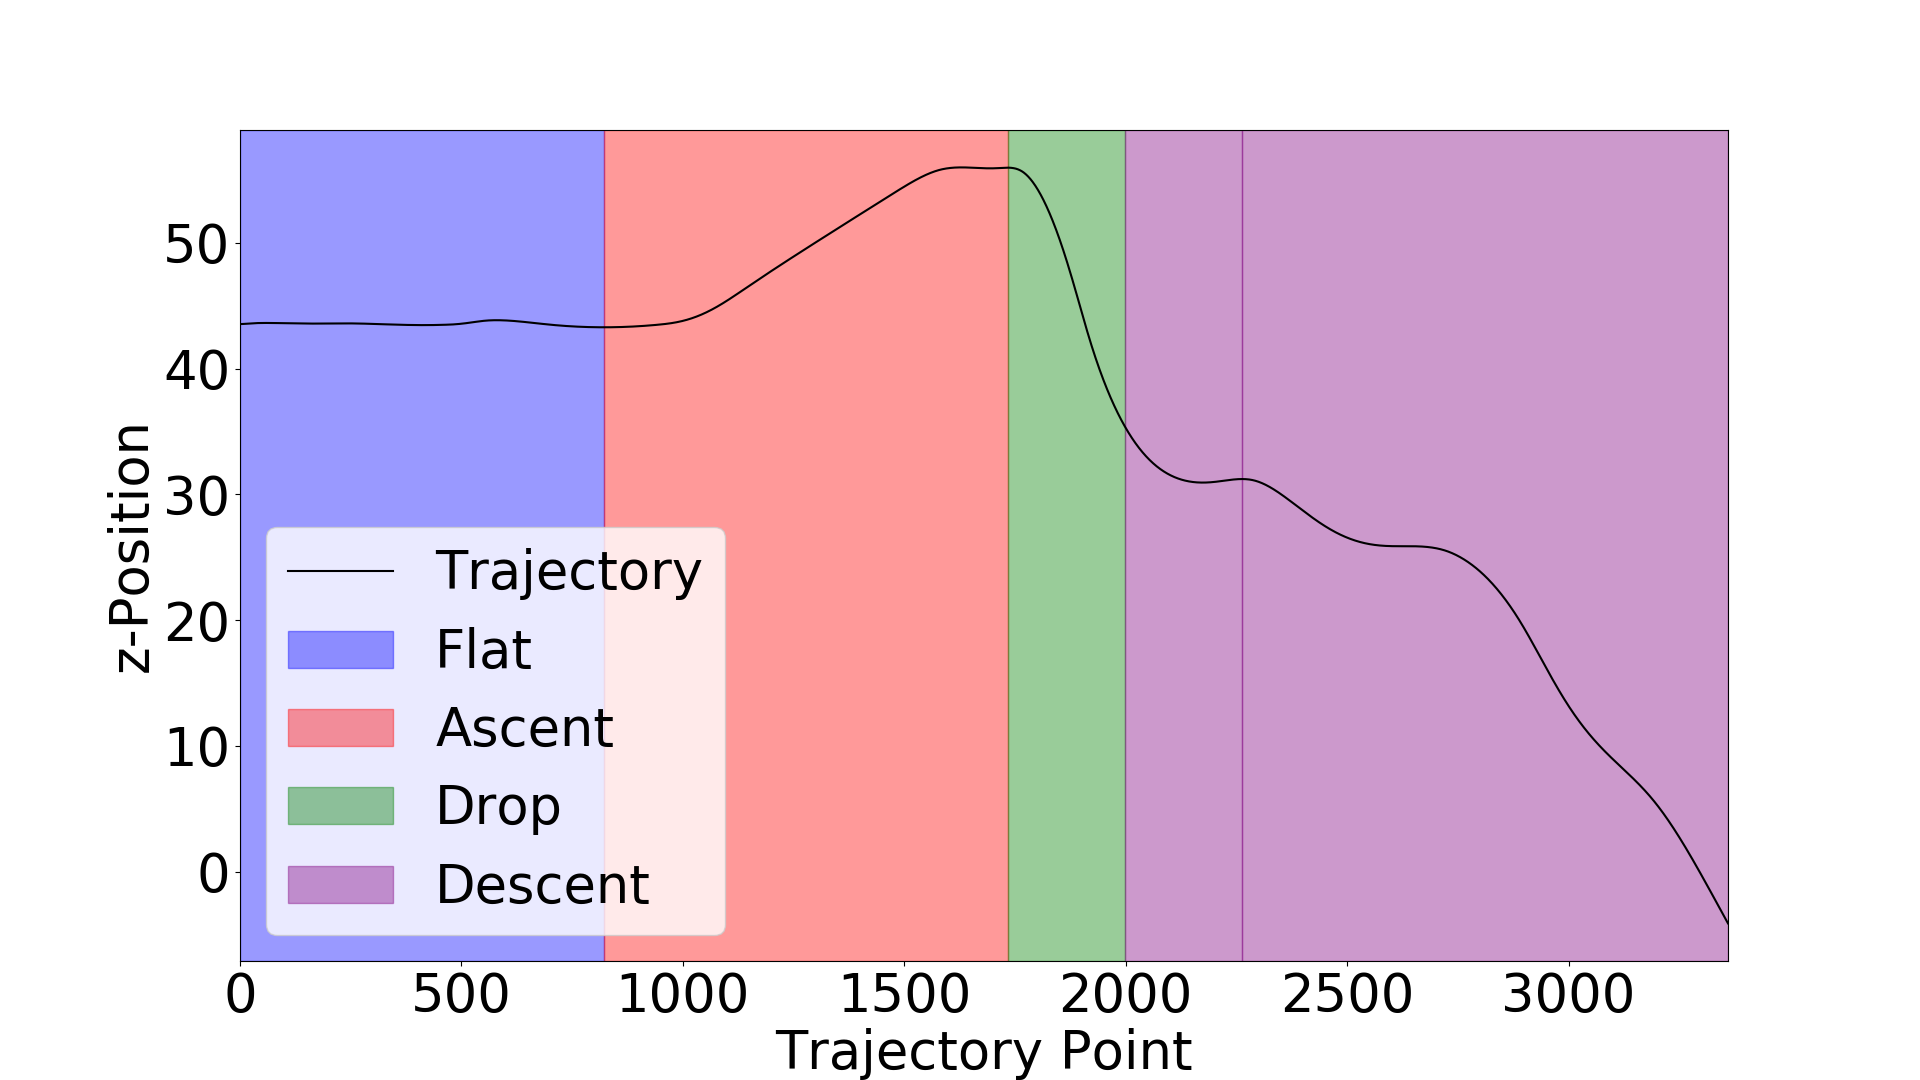}
\captionof*{figure}{Height Difference $1m$, Min Duration $2s$.}

\includegraphics[width=0.49\linewidth]{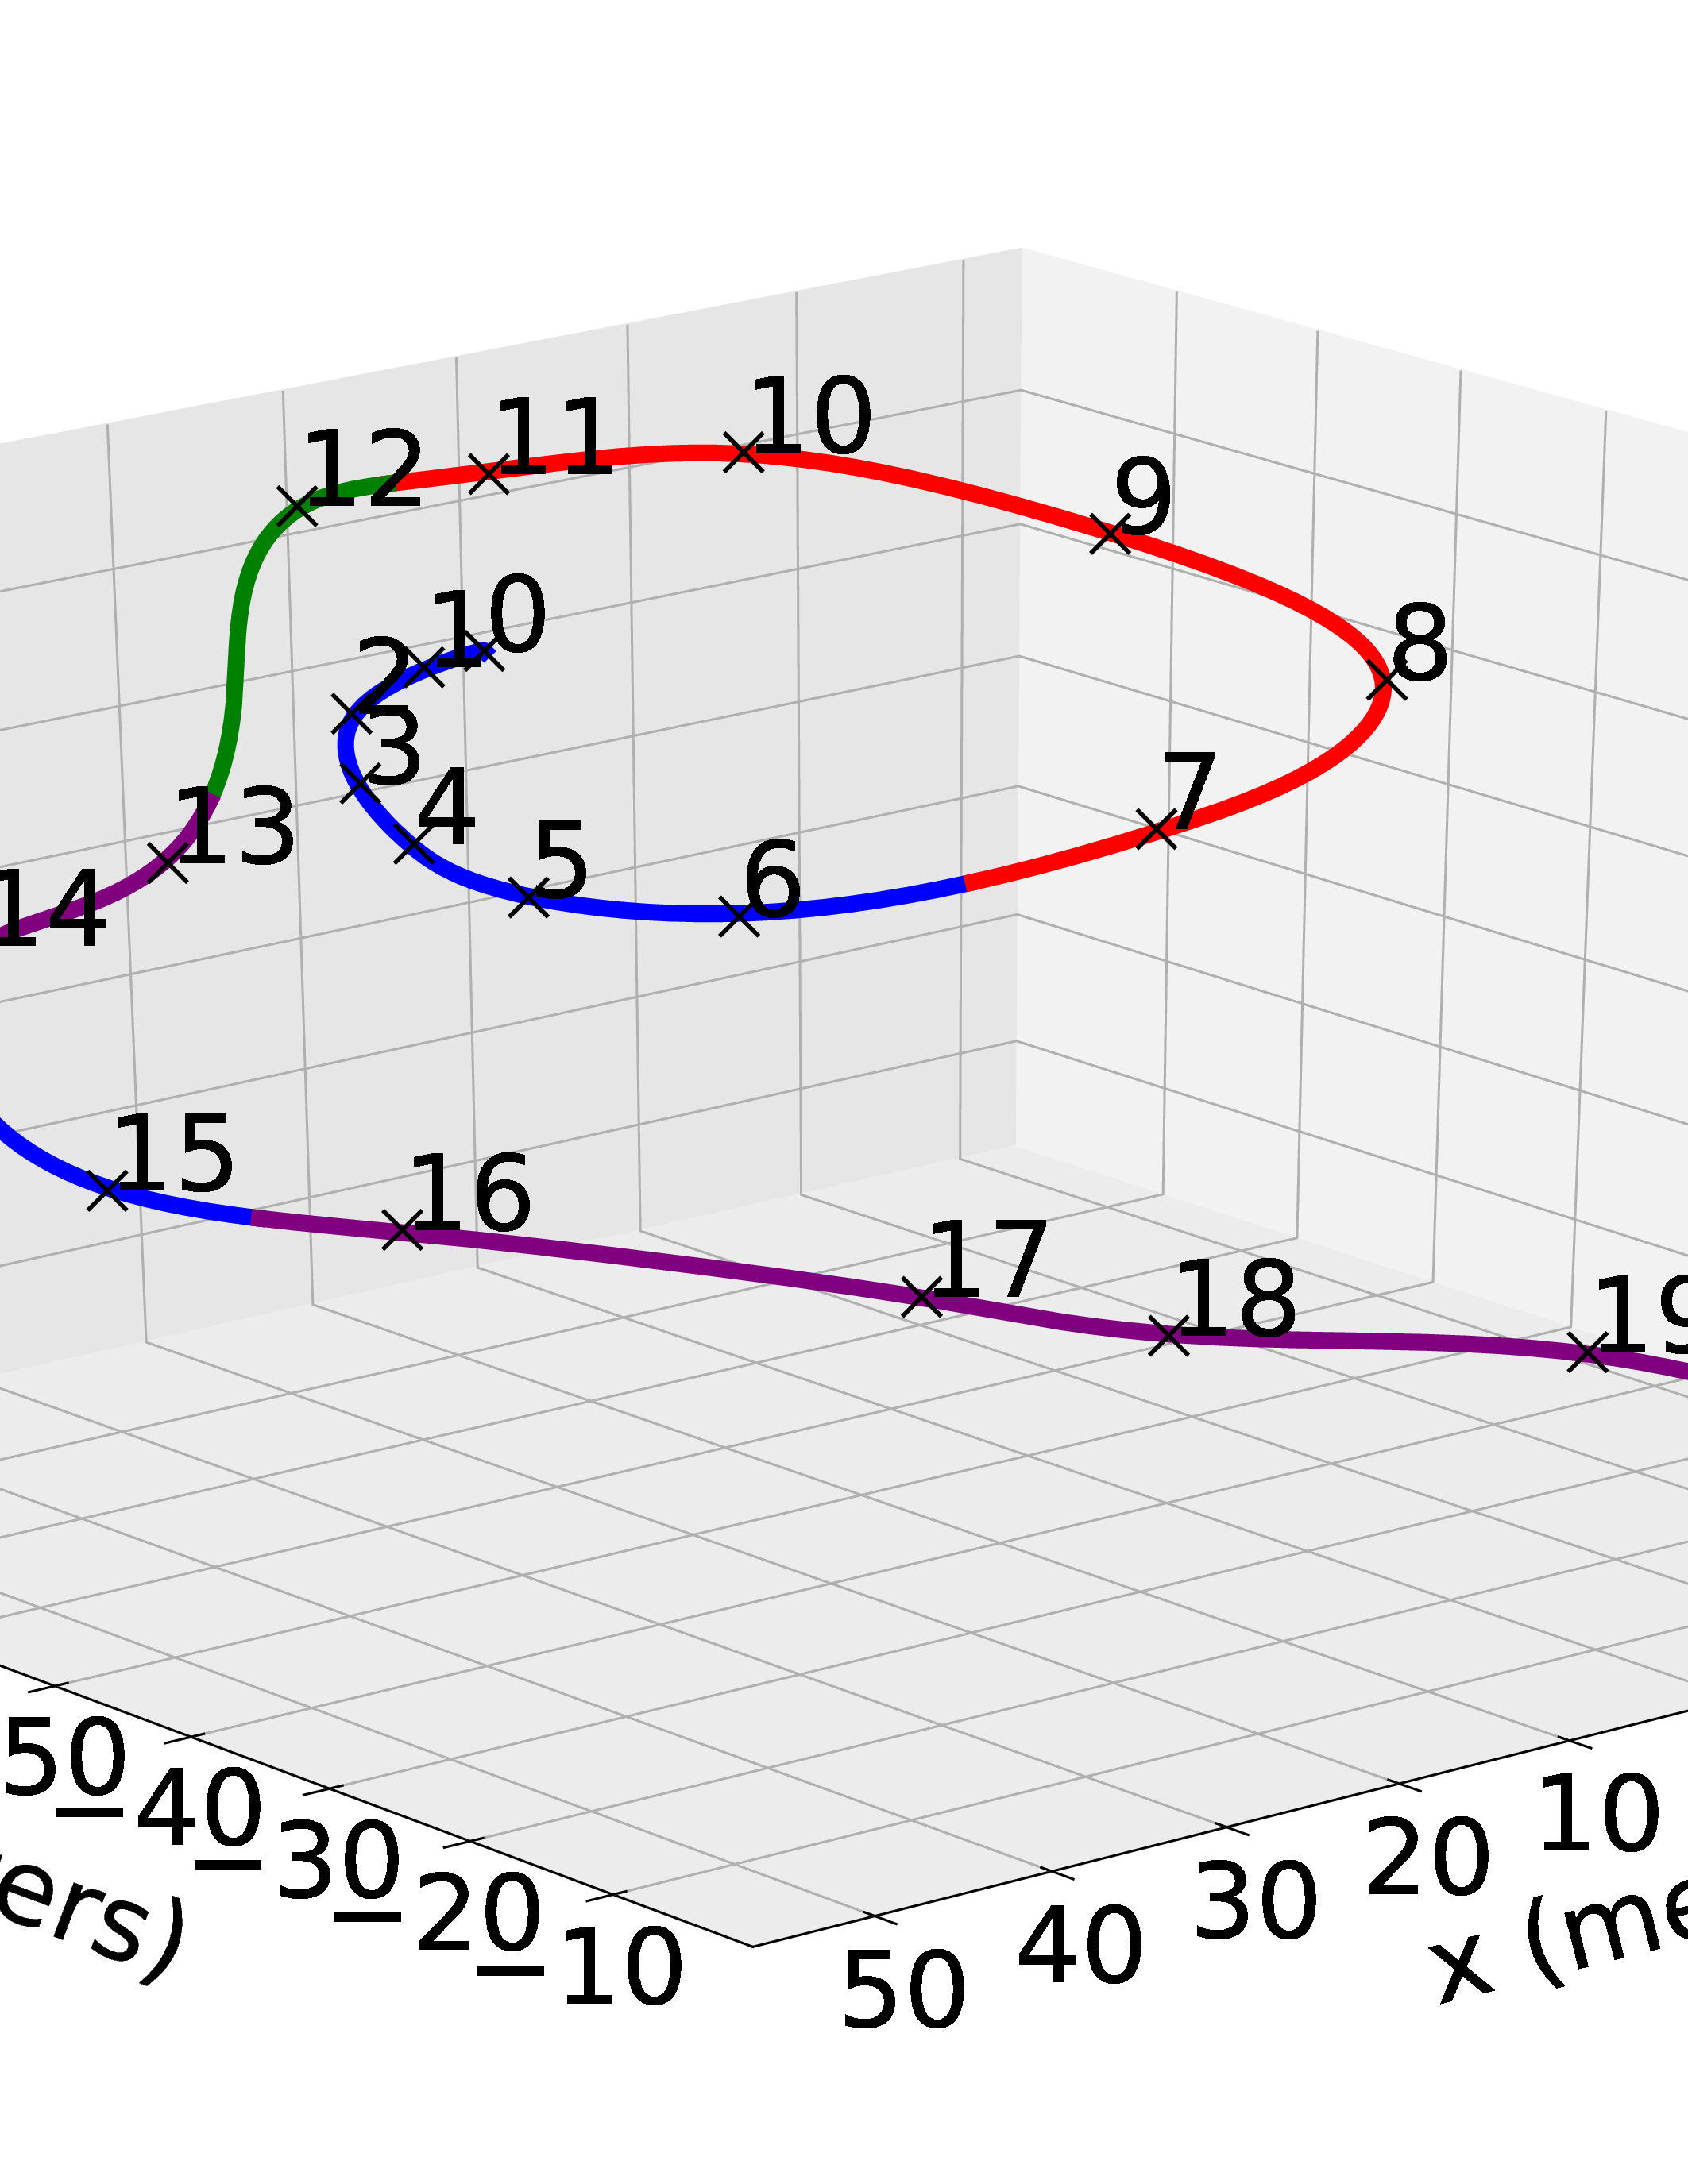}
\includegraphics[width=0.49\linewidth]{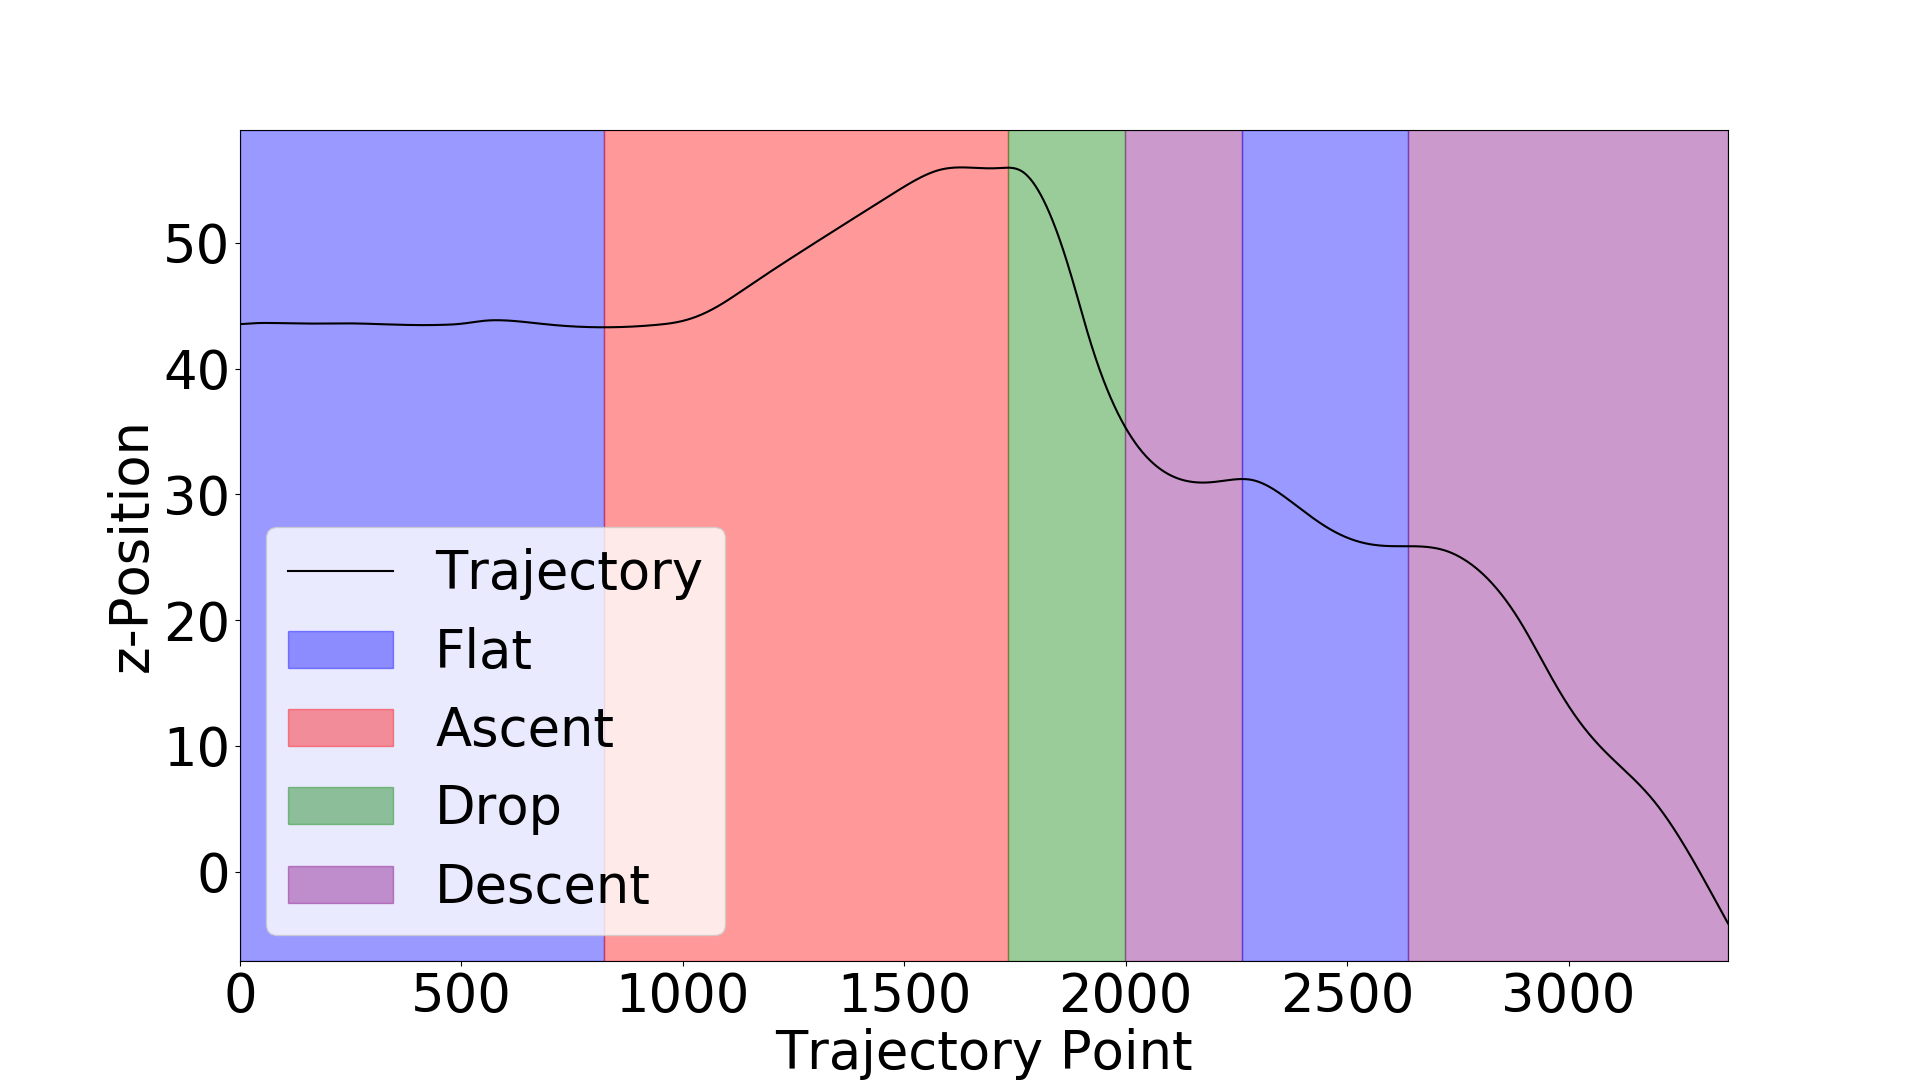}
\captionof*{figure}{Height Difference $10m$, Min Duration $2s$.}

\includegraphics[width=0.49\linewidth]{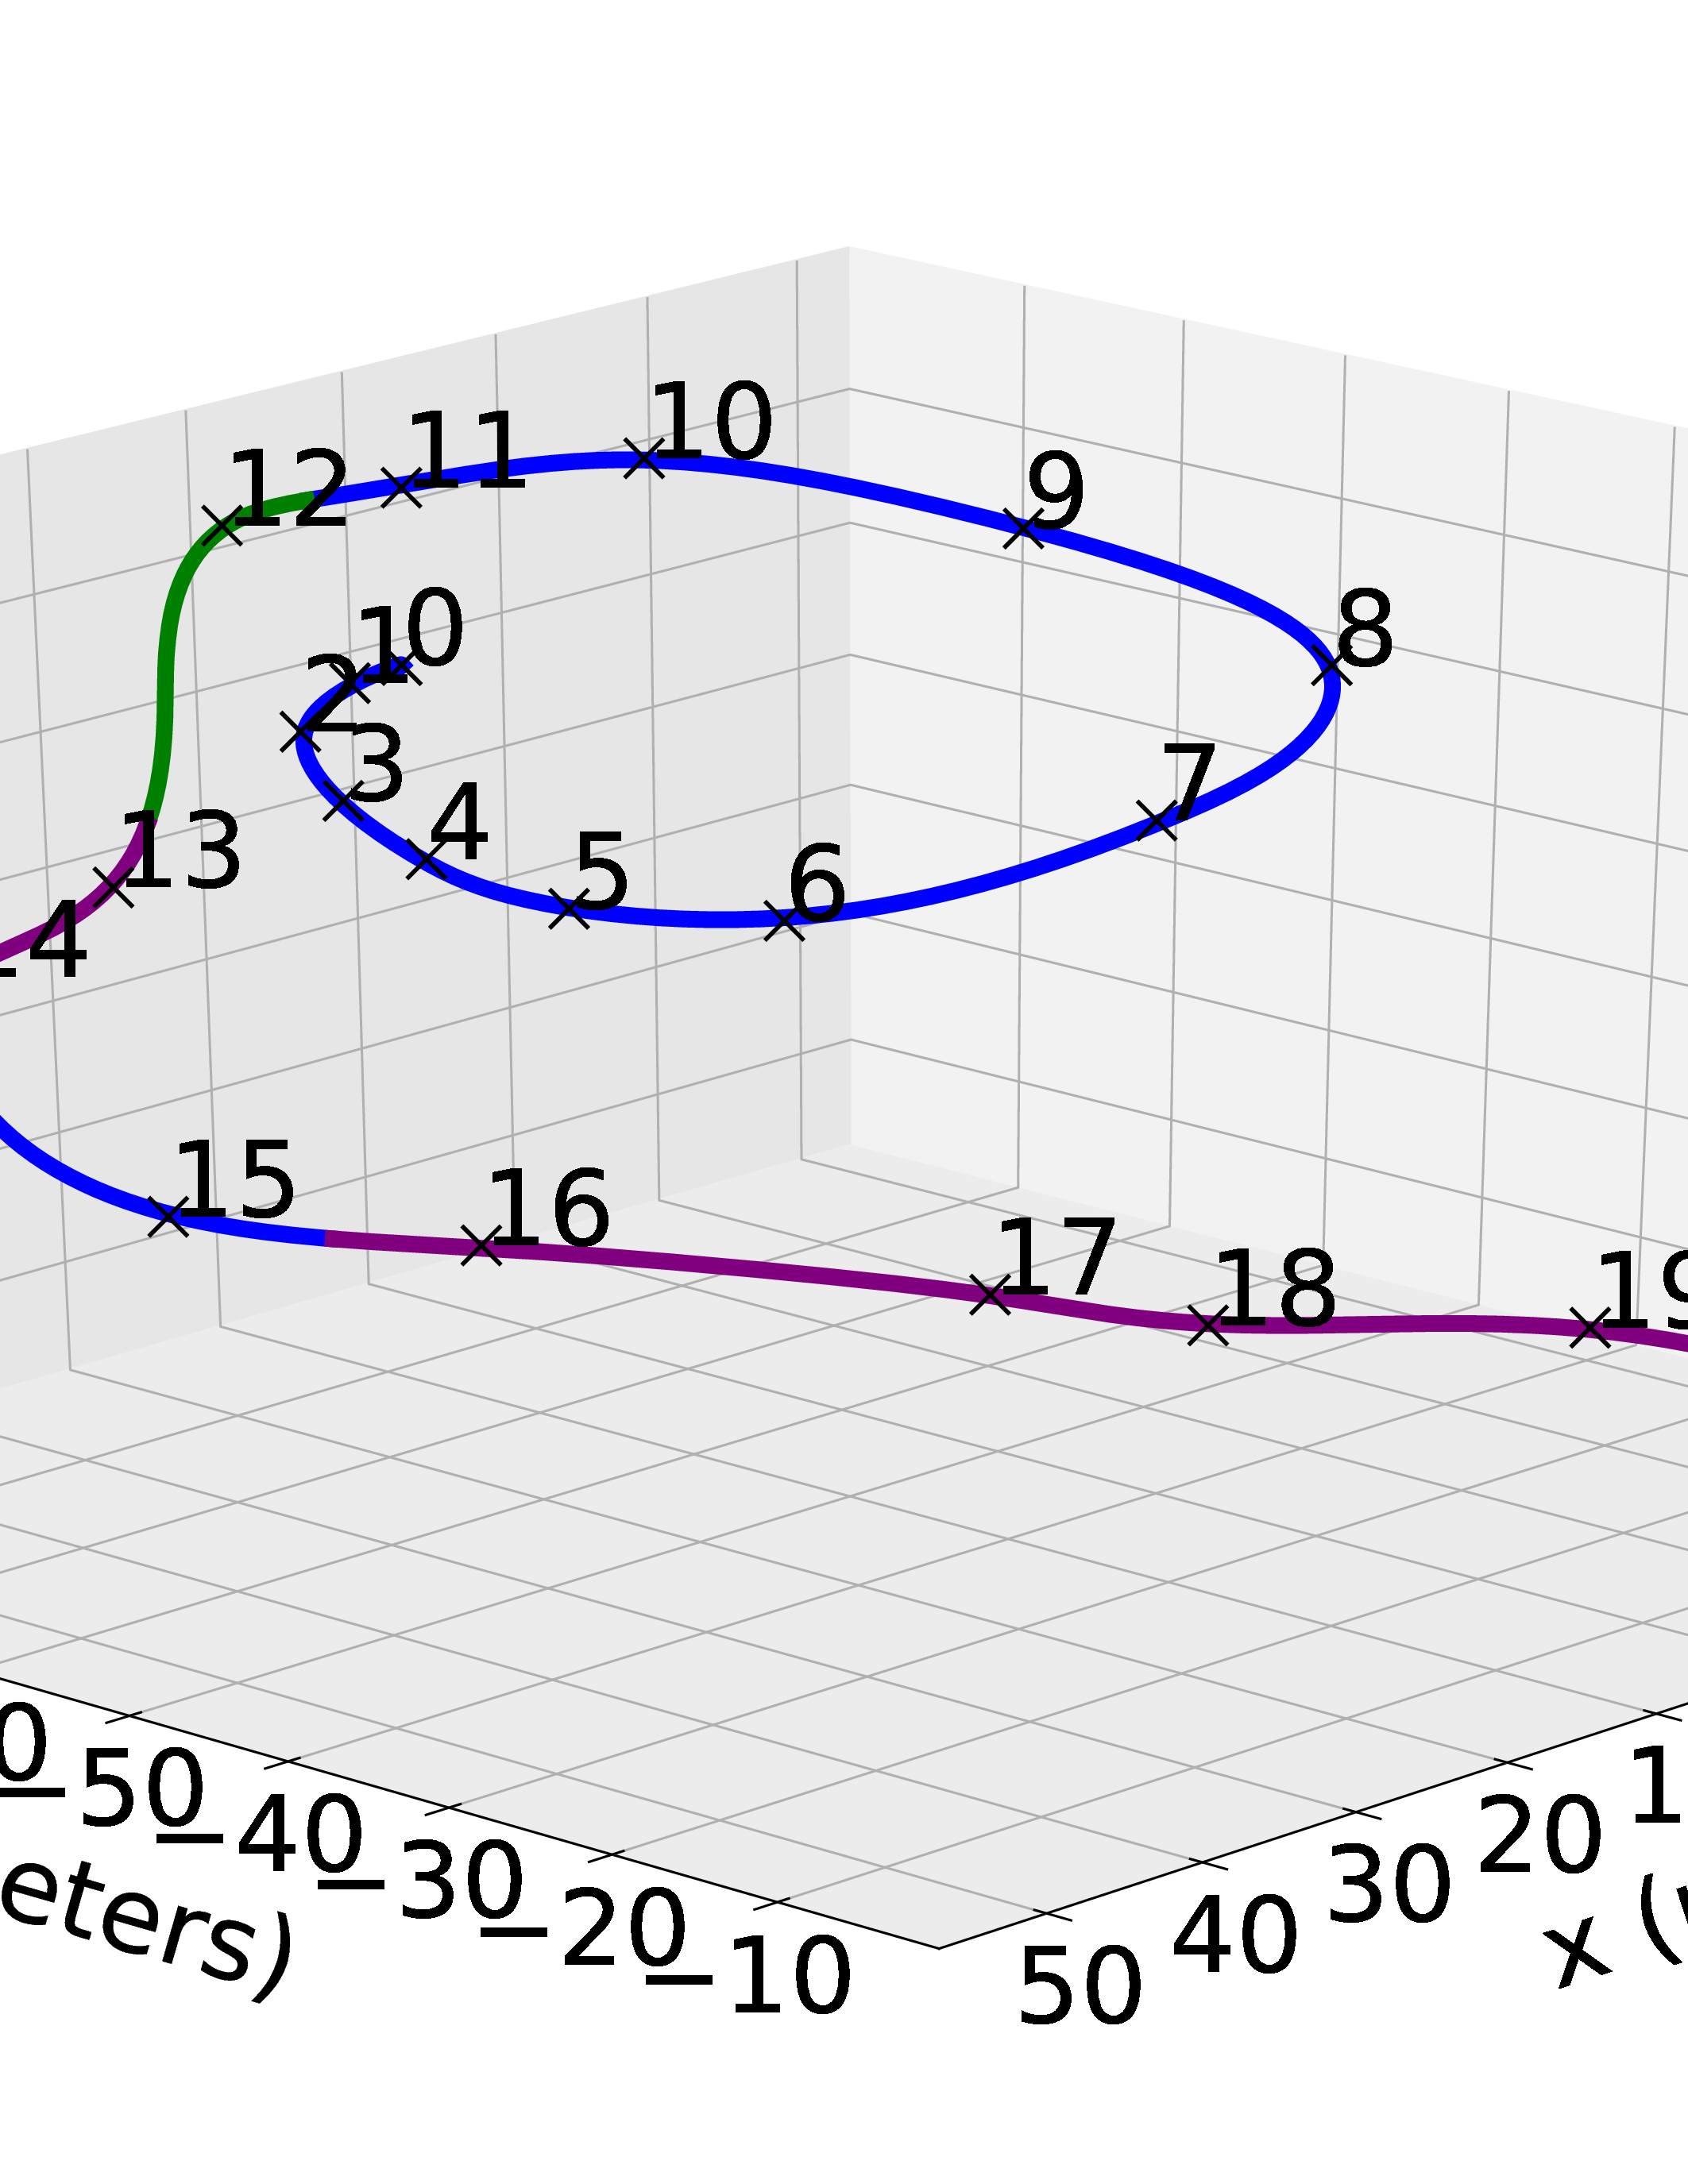}
\includegraphics[width=0.49\linewidth]{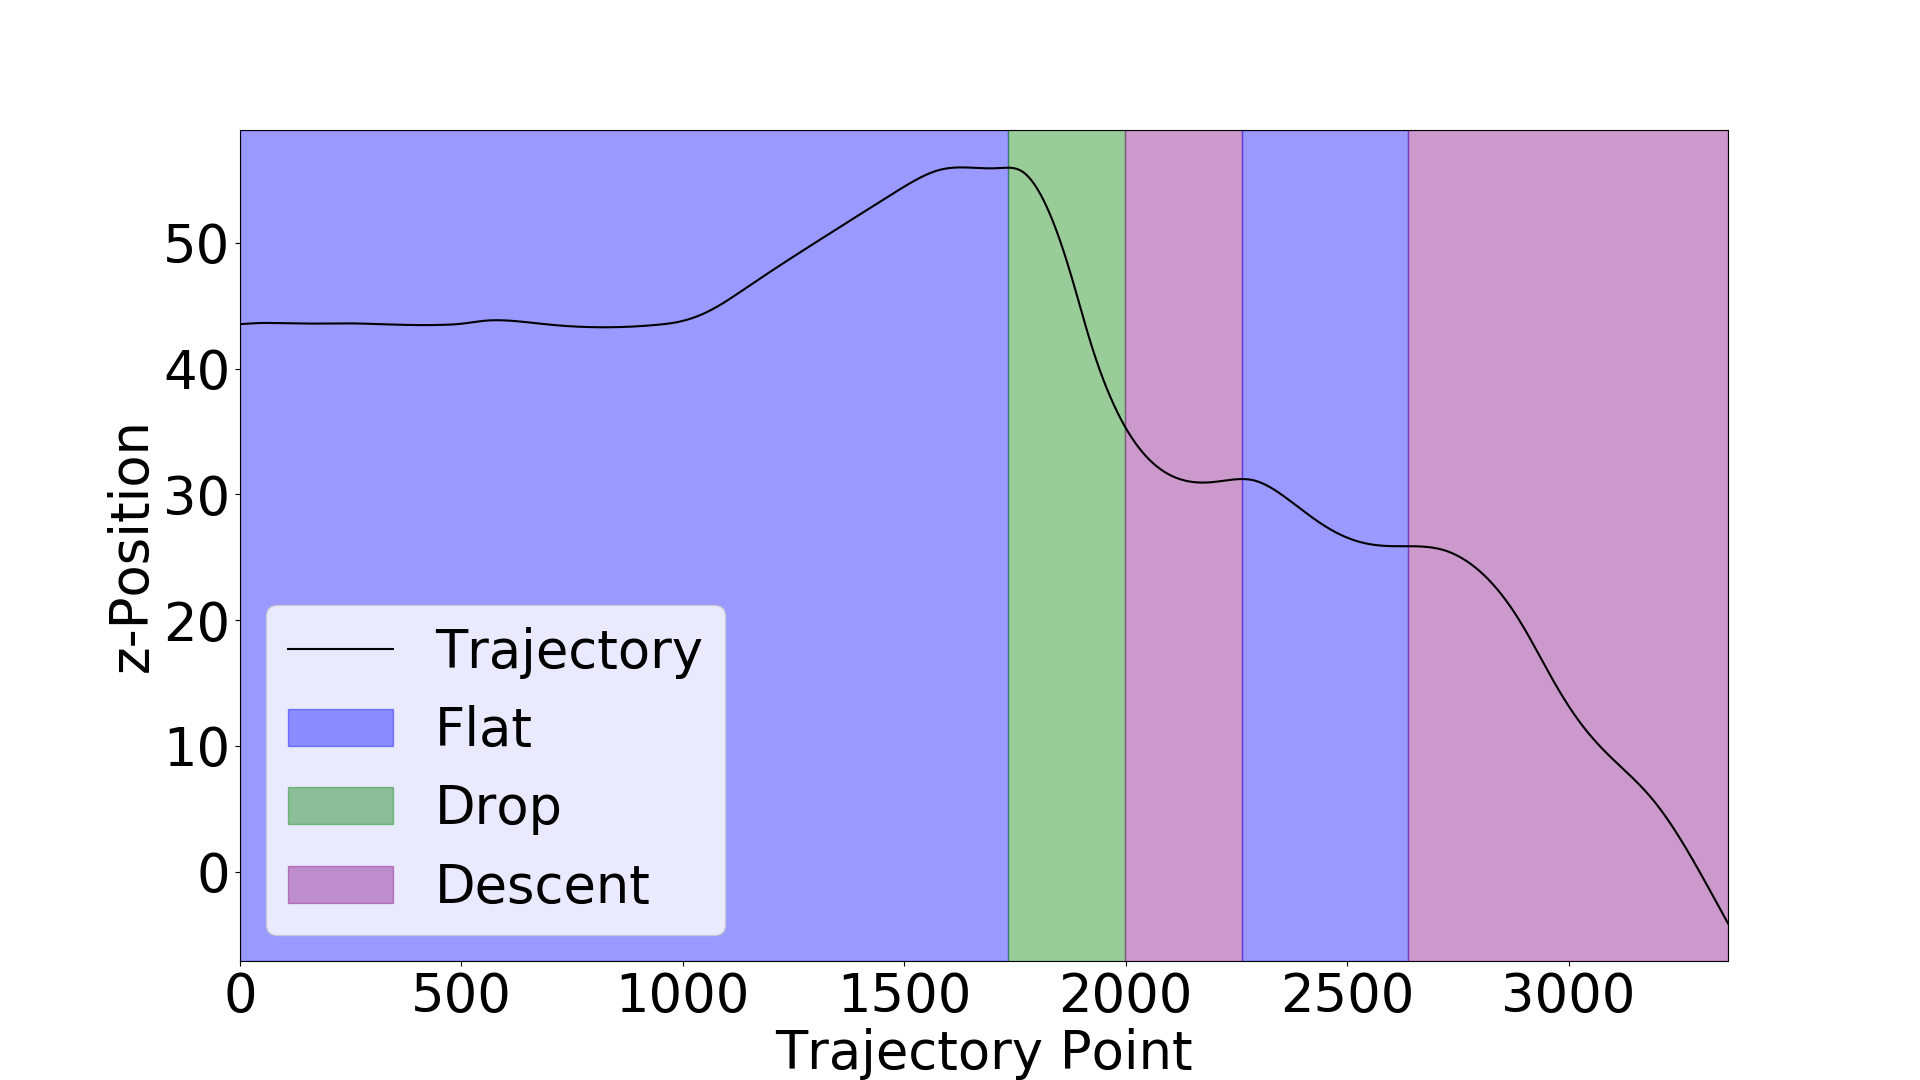}
\captionof*{figure}{Height Difference $20m$, Min Duration $2s$.}

\includegraphics[width=0.49\linewidth]{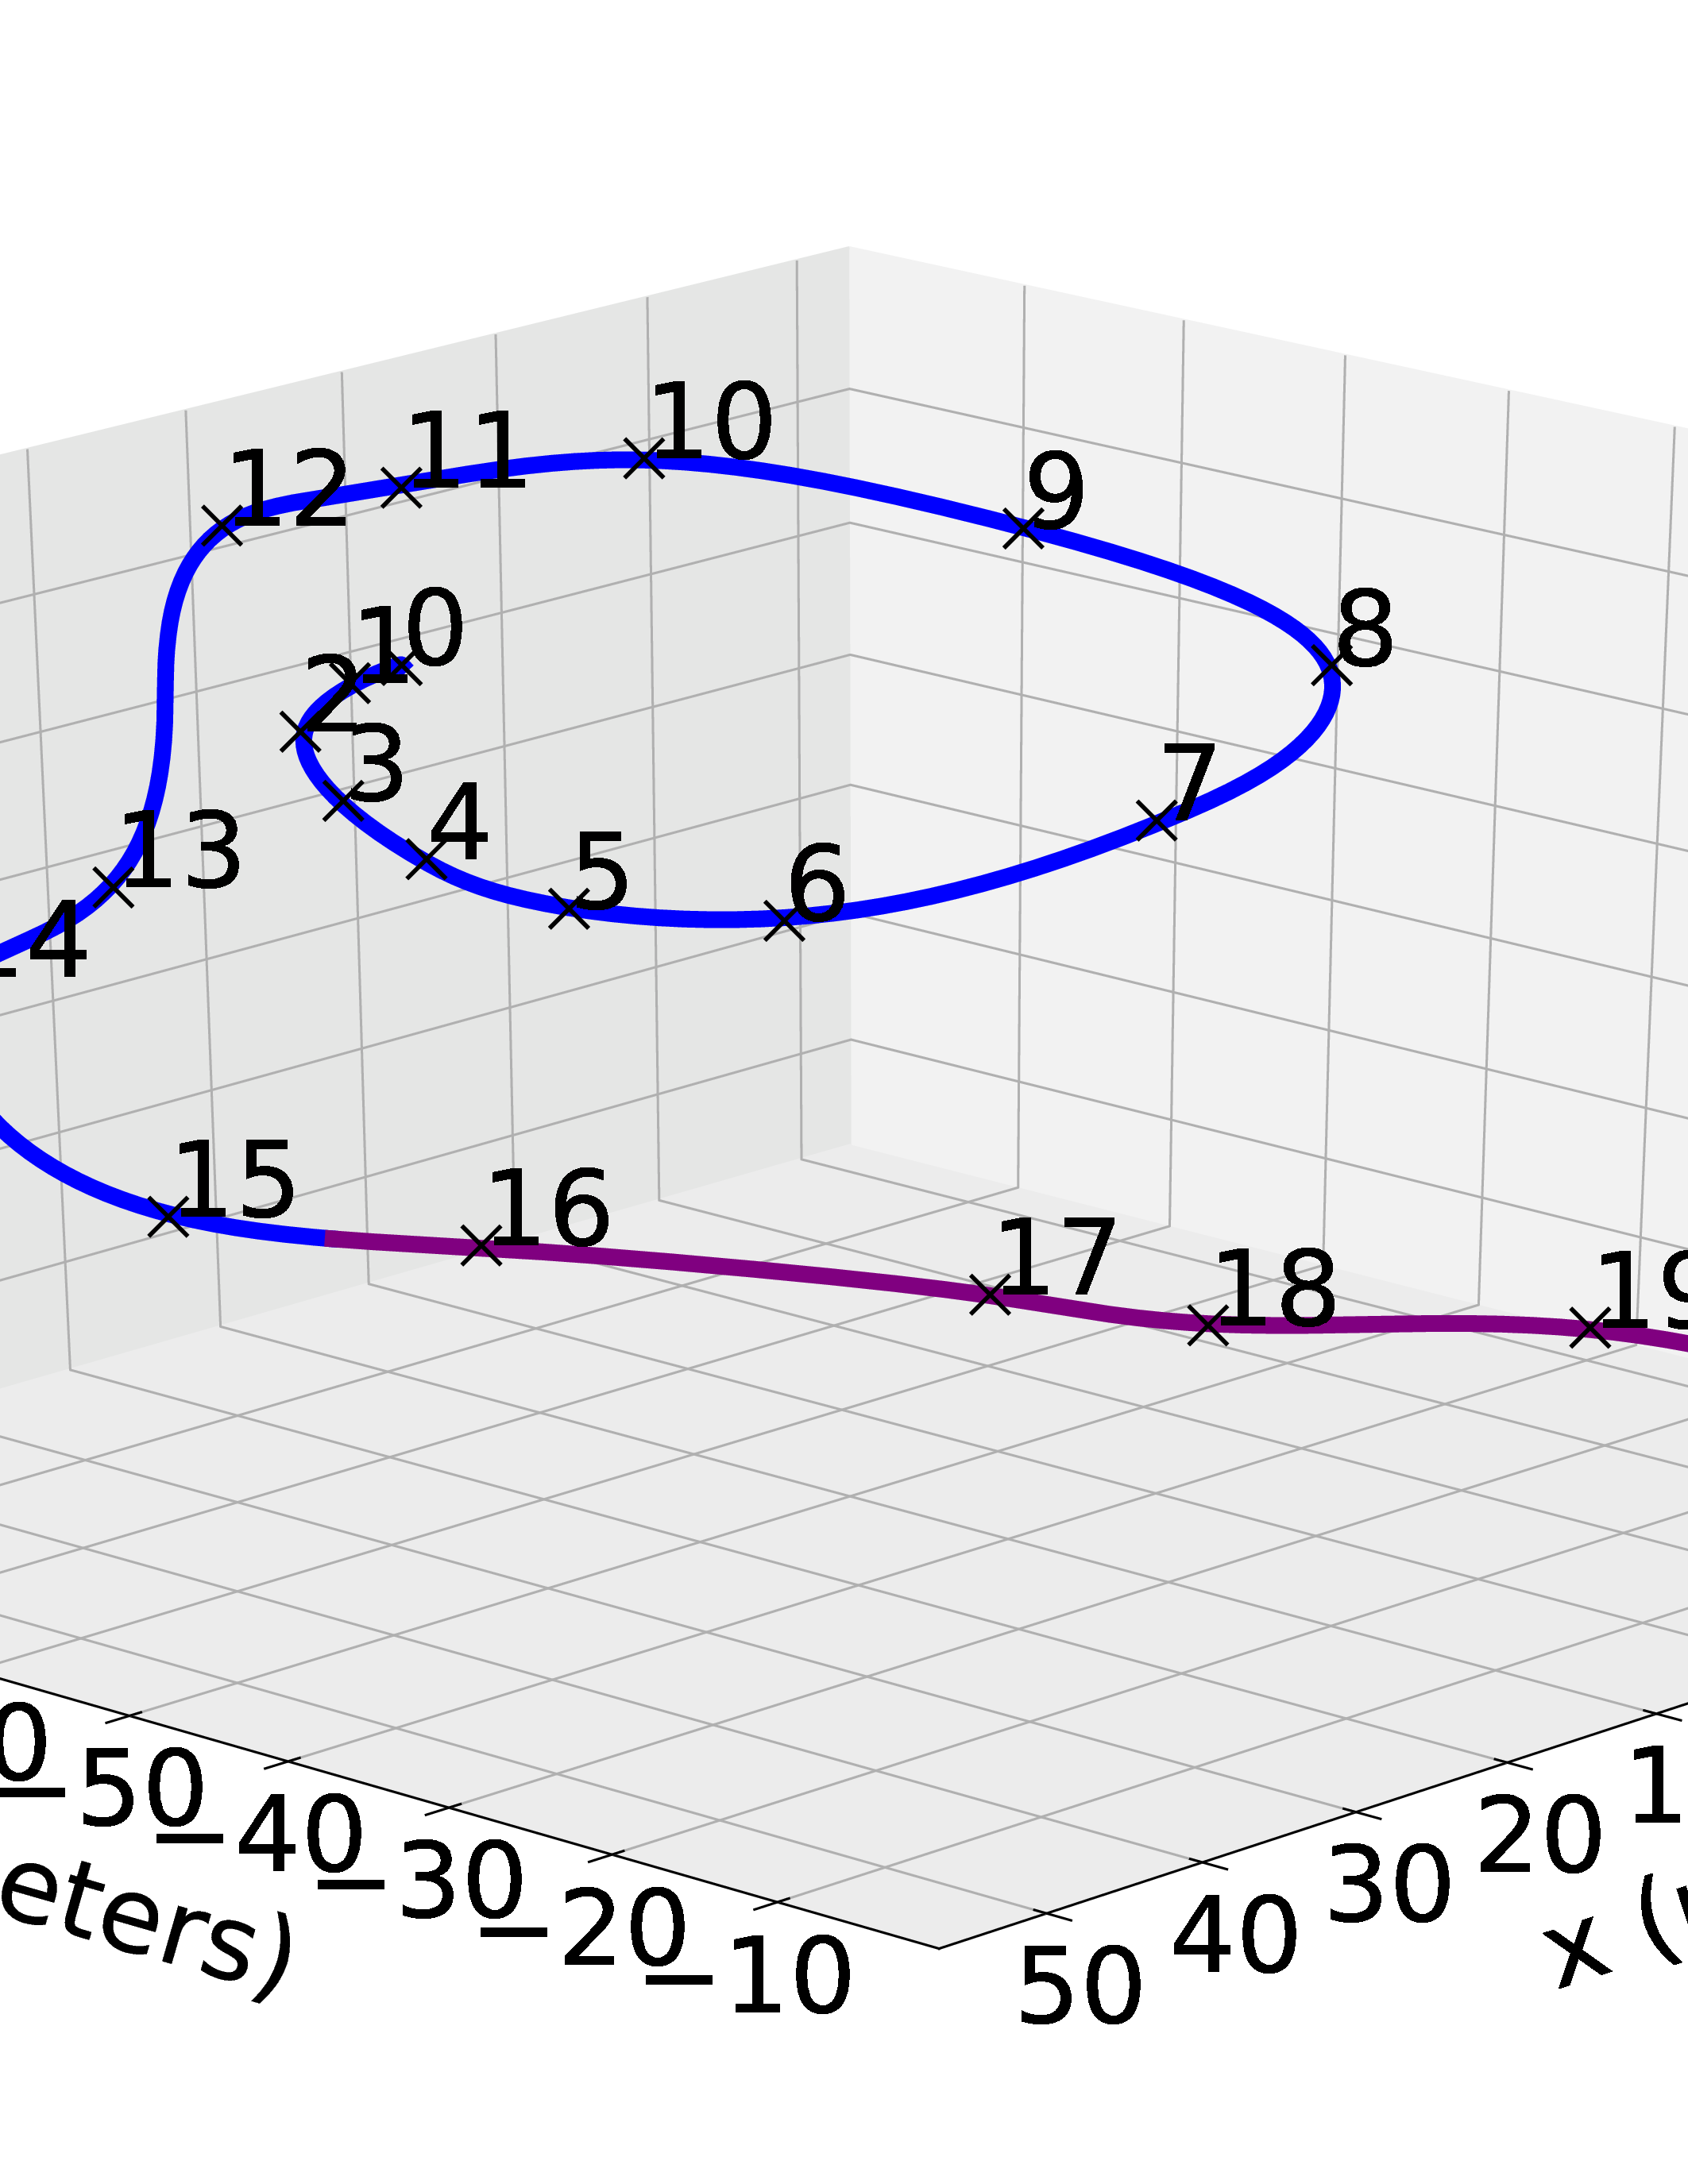}
\includegraphics[width=0.49\linewidth]{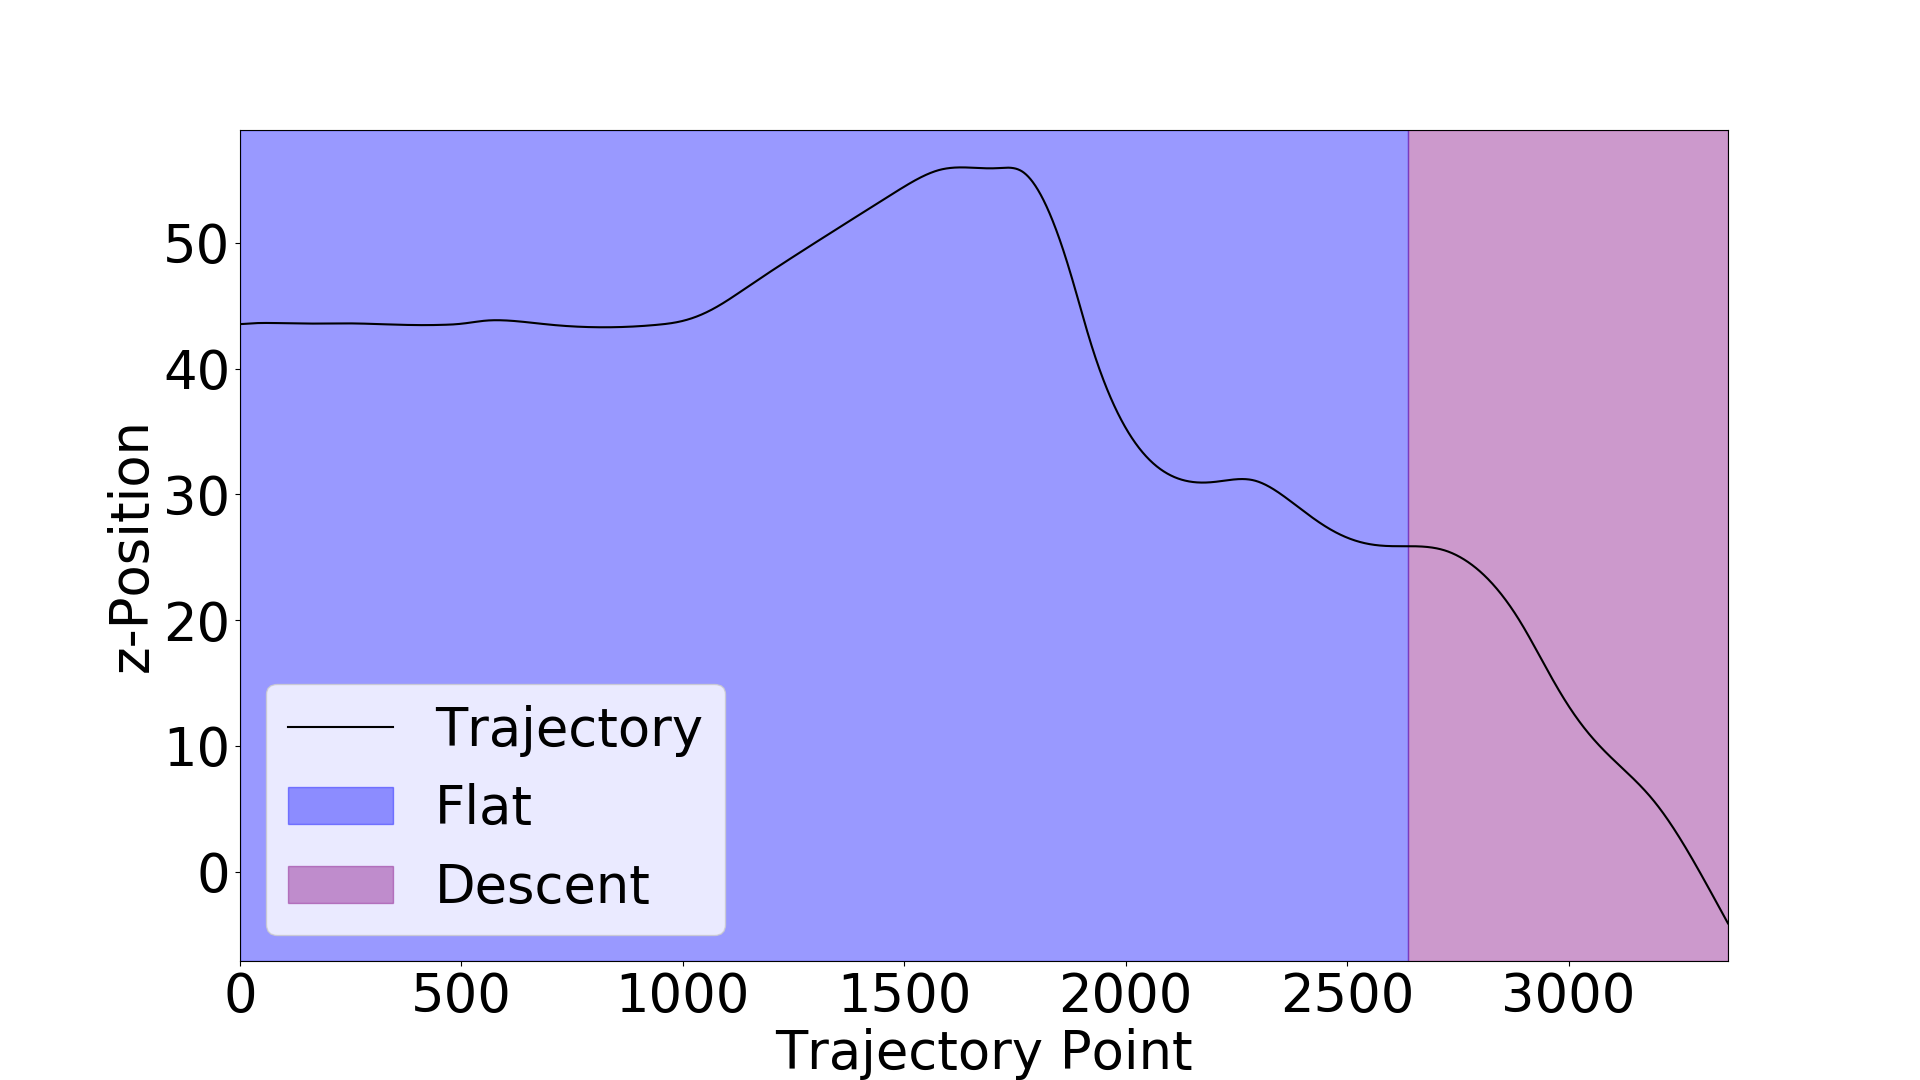}
\captionof*{figure}{Height Difference $30m$, Min Duration $2s$.}

\includegraphics[width=0.49\linewidth]{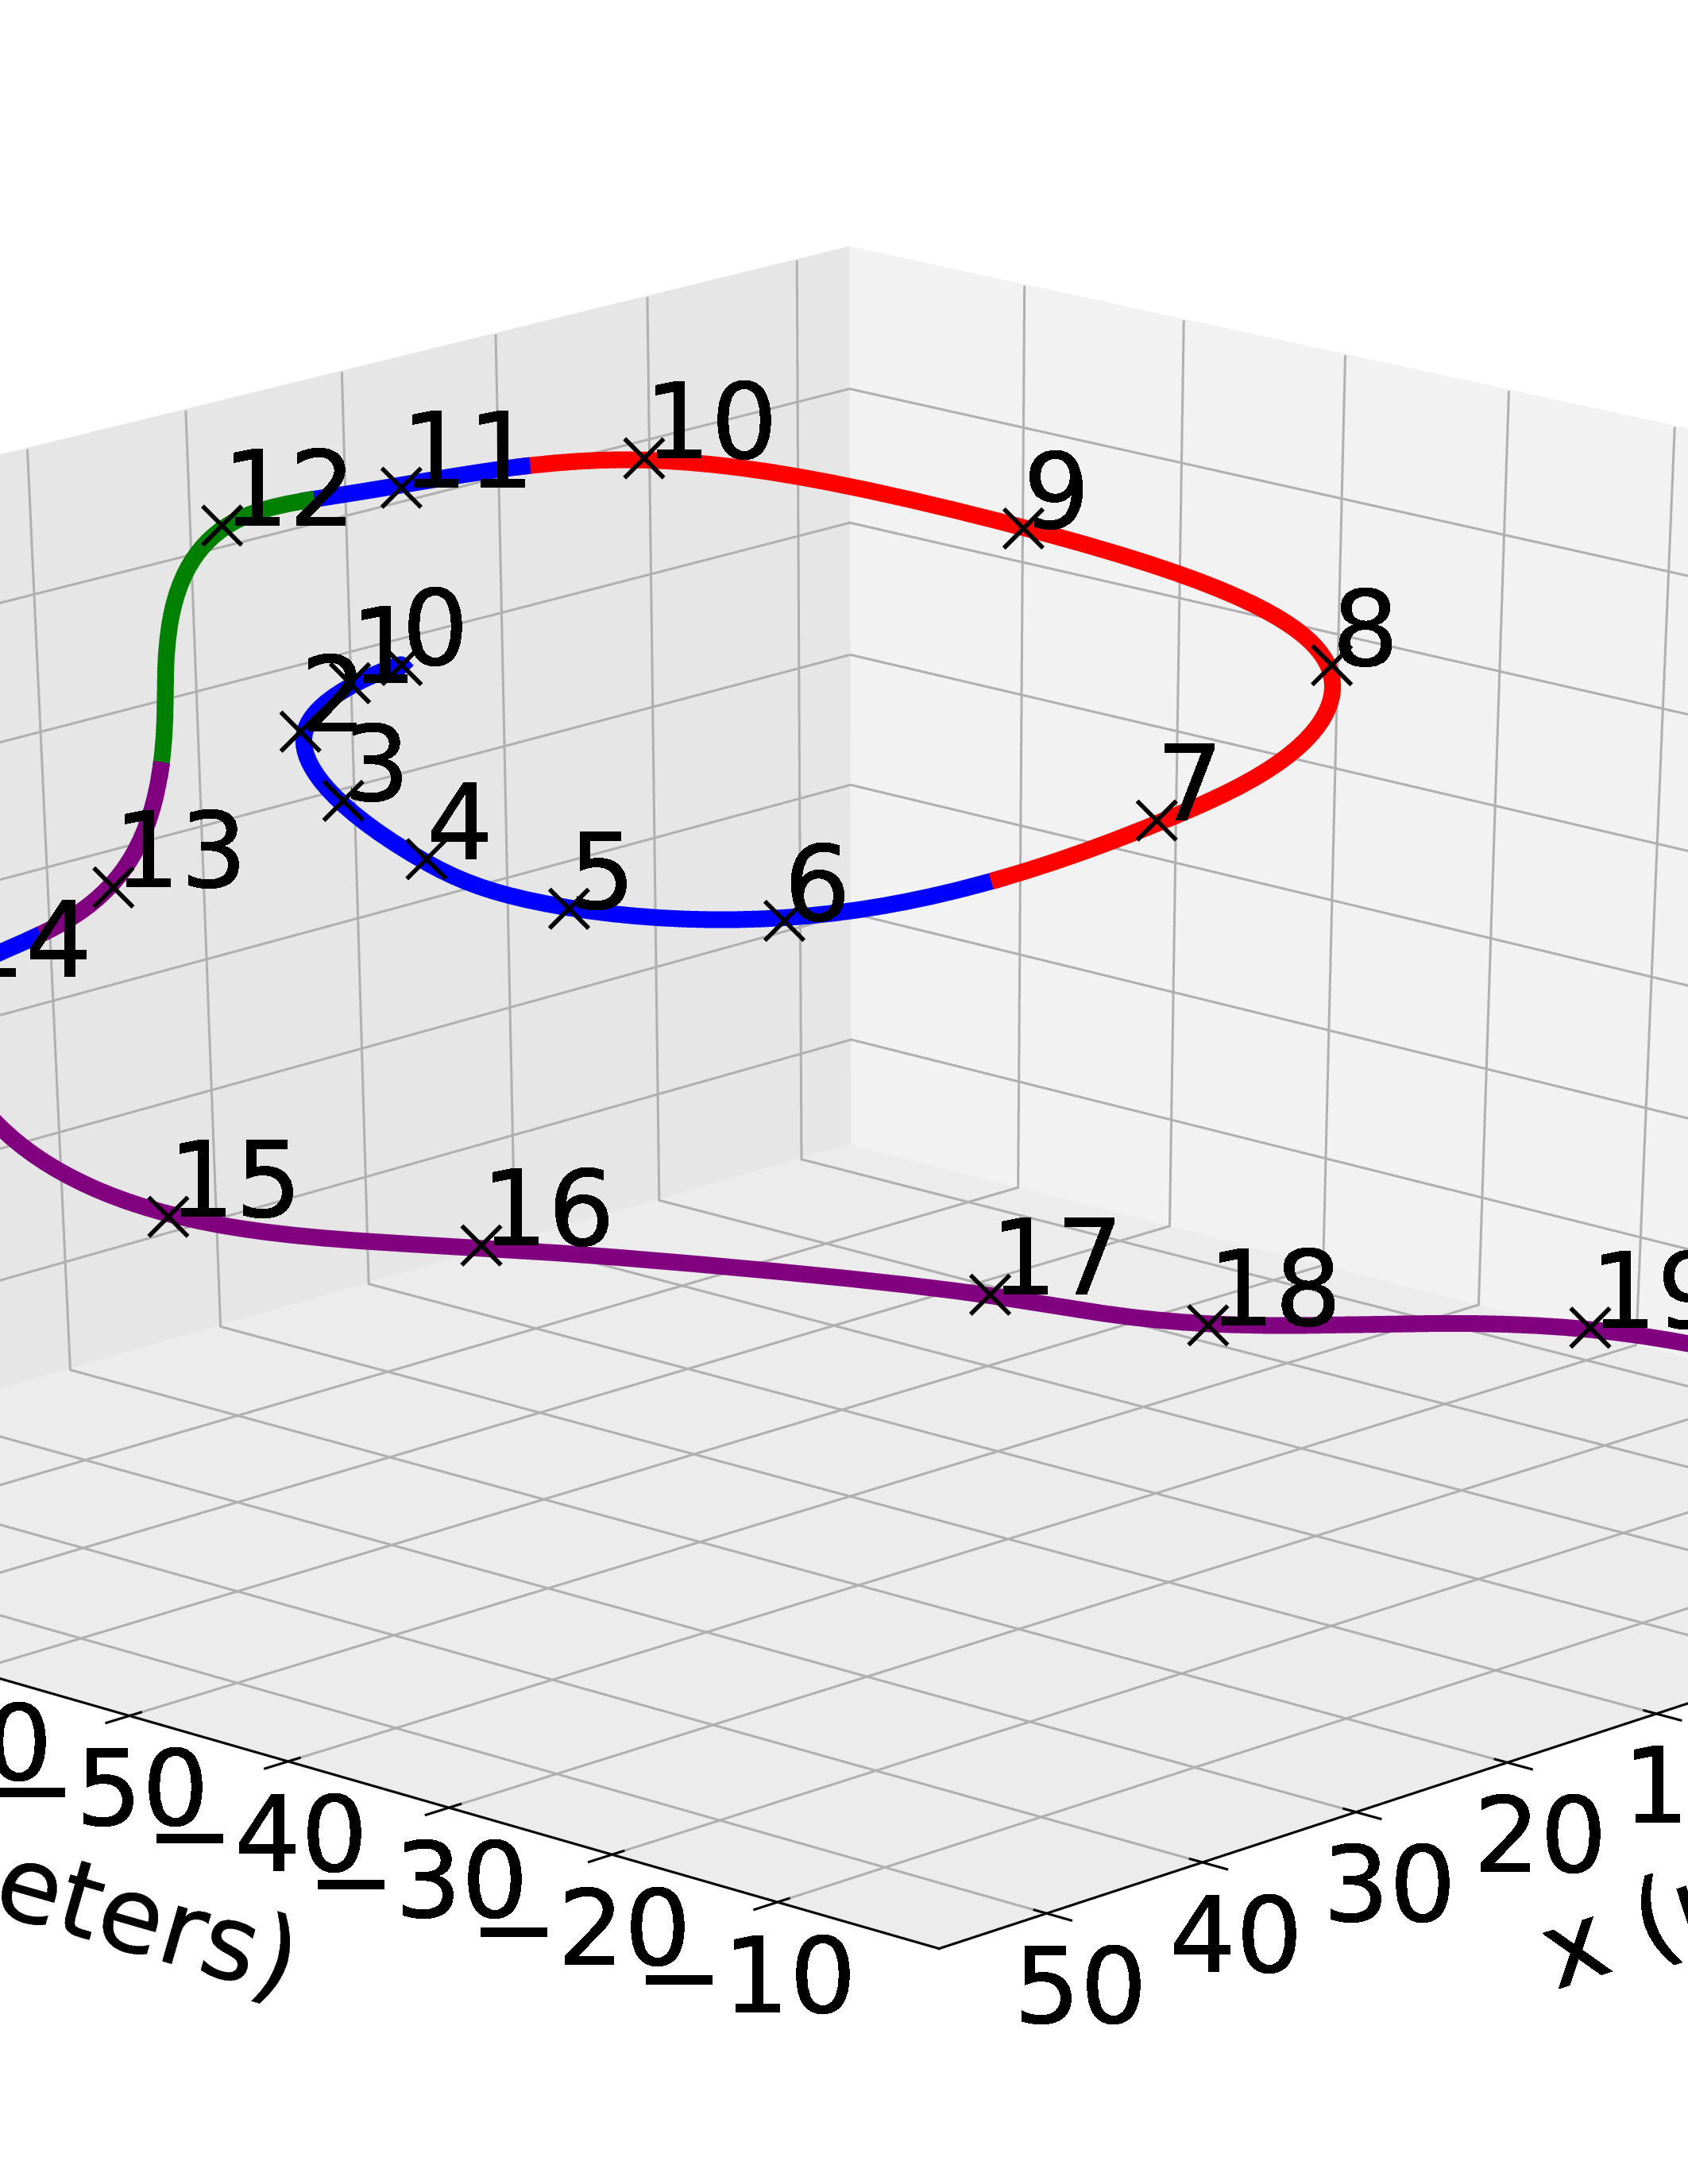}
\includegraphics[width=0.49\linewidth]{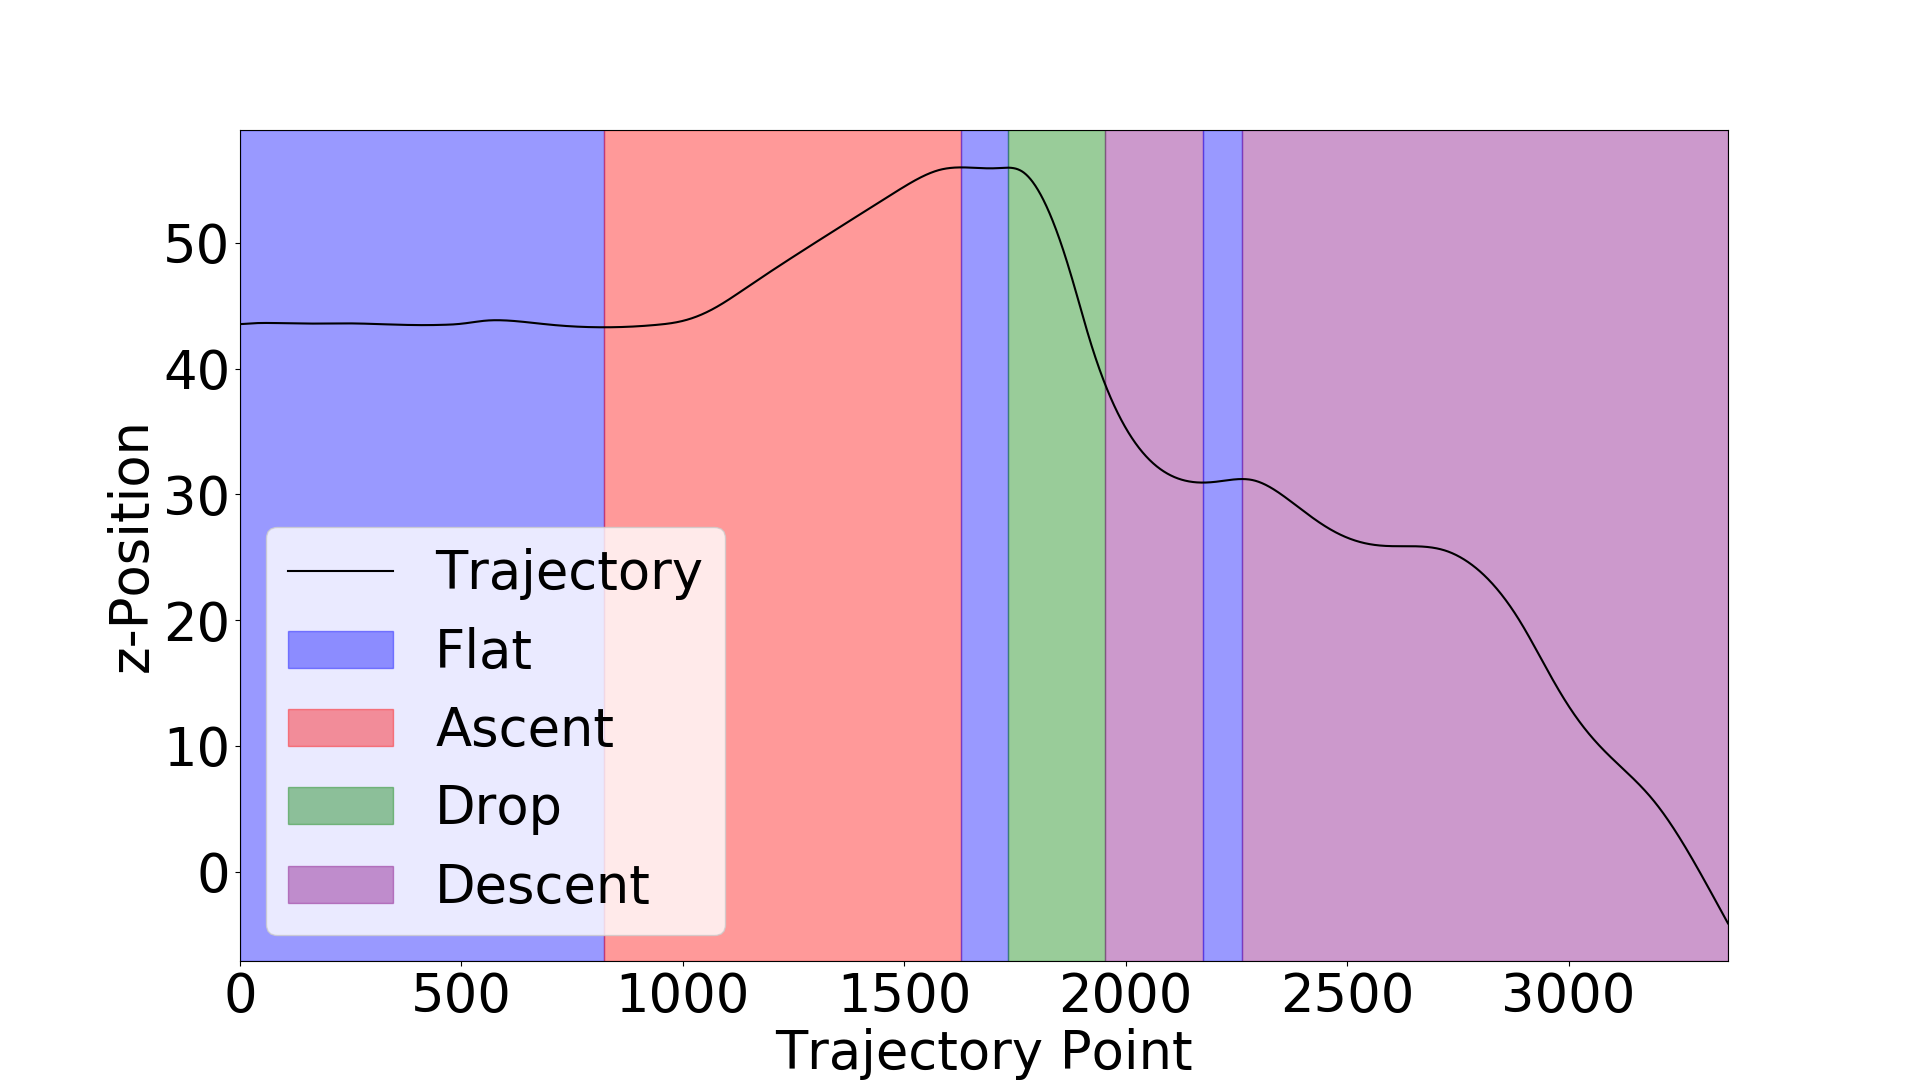}
\captionof*{figure}{Height Difference $1m$, Min Duration $1s$.}

\includegraphics[width=0.49\linewidth]{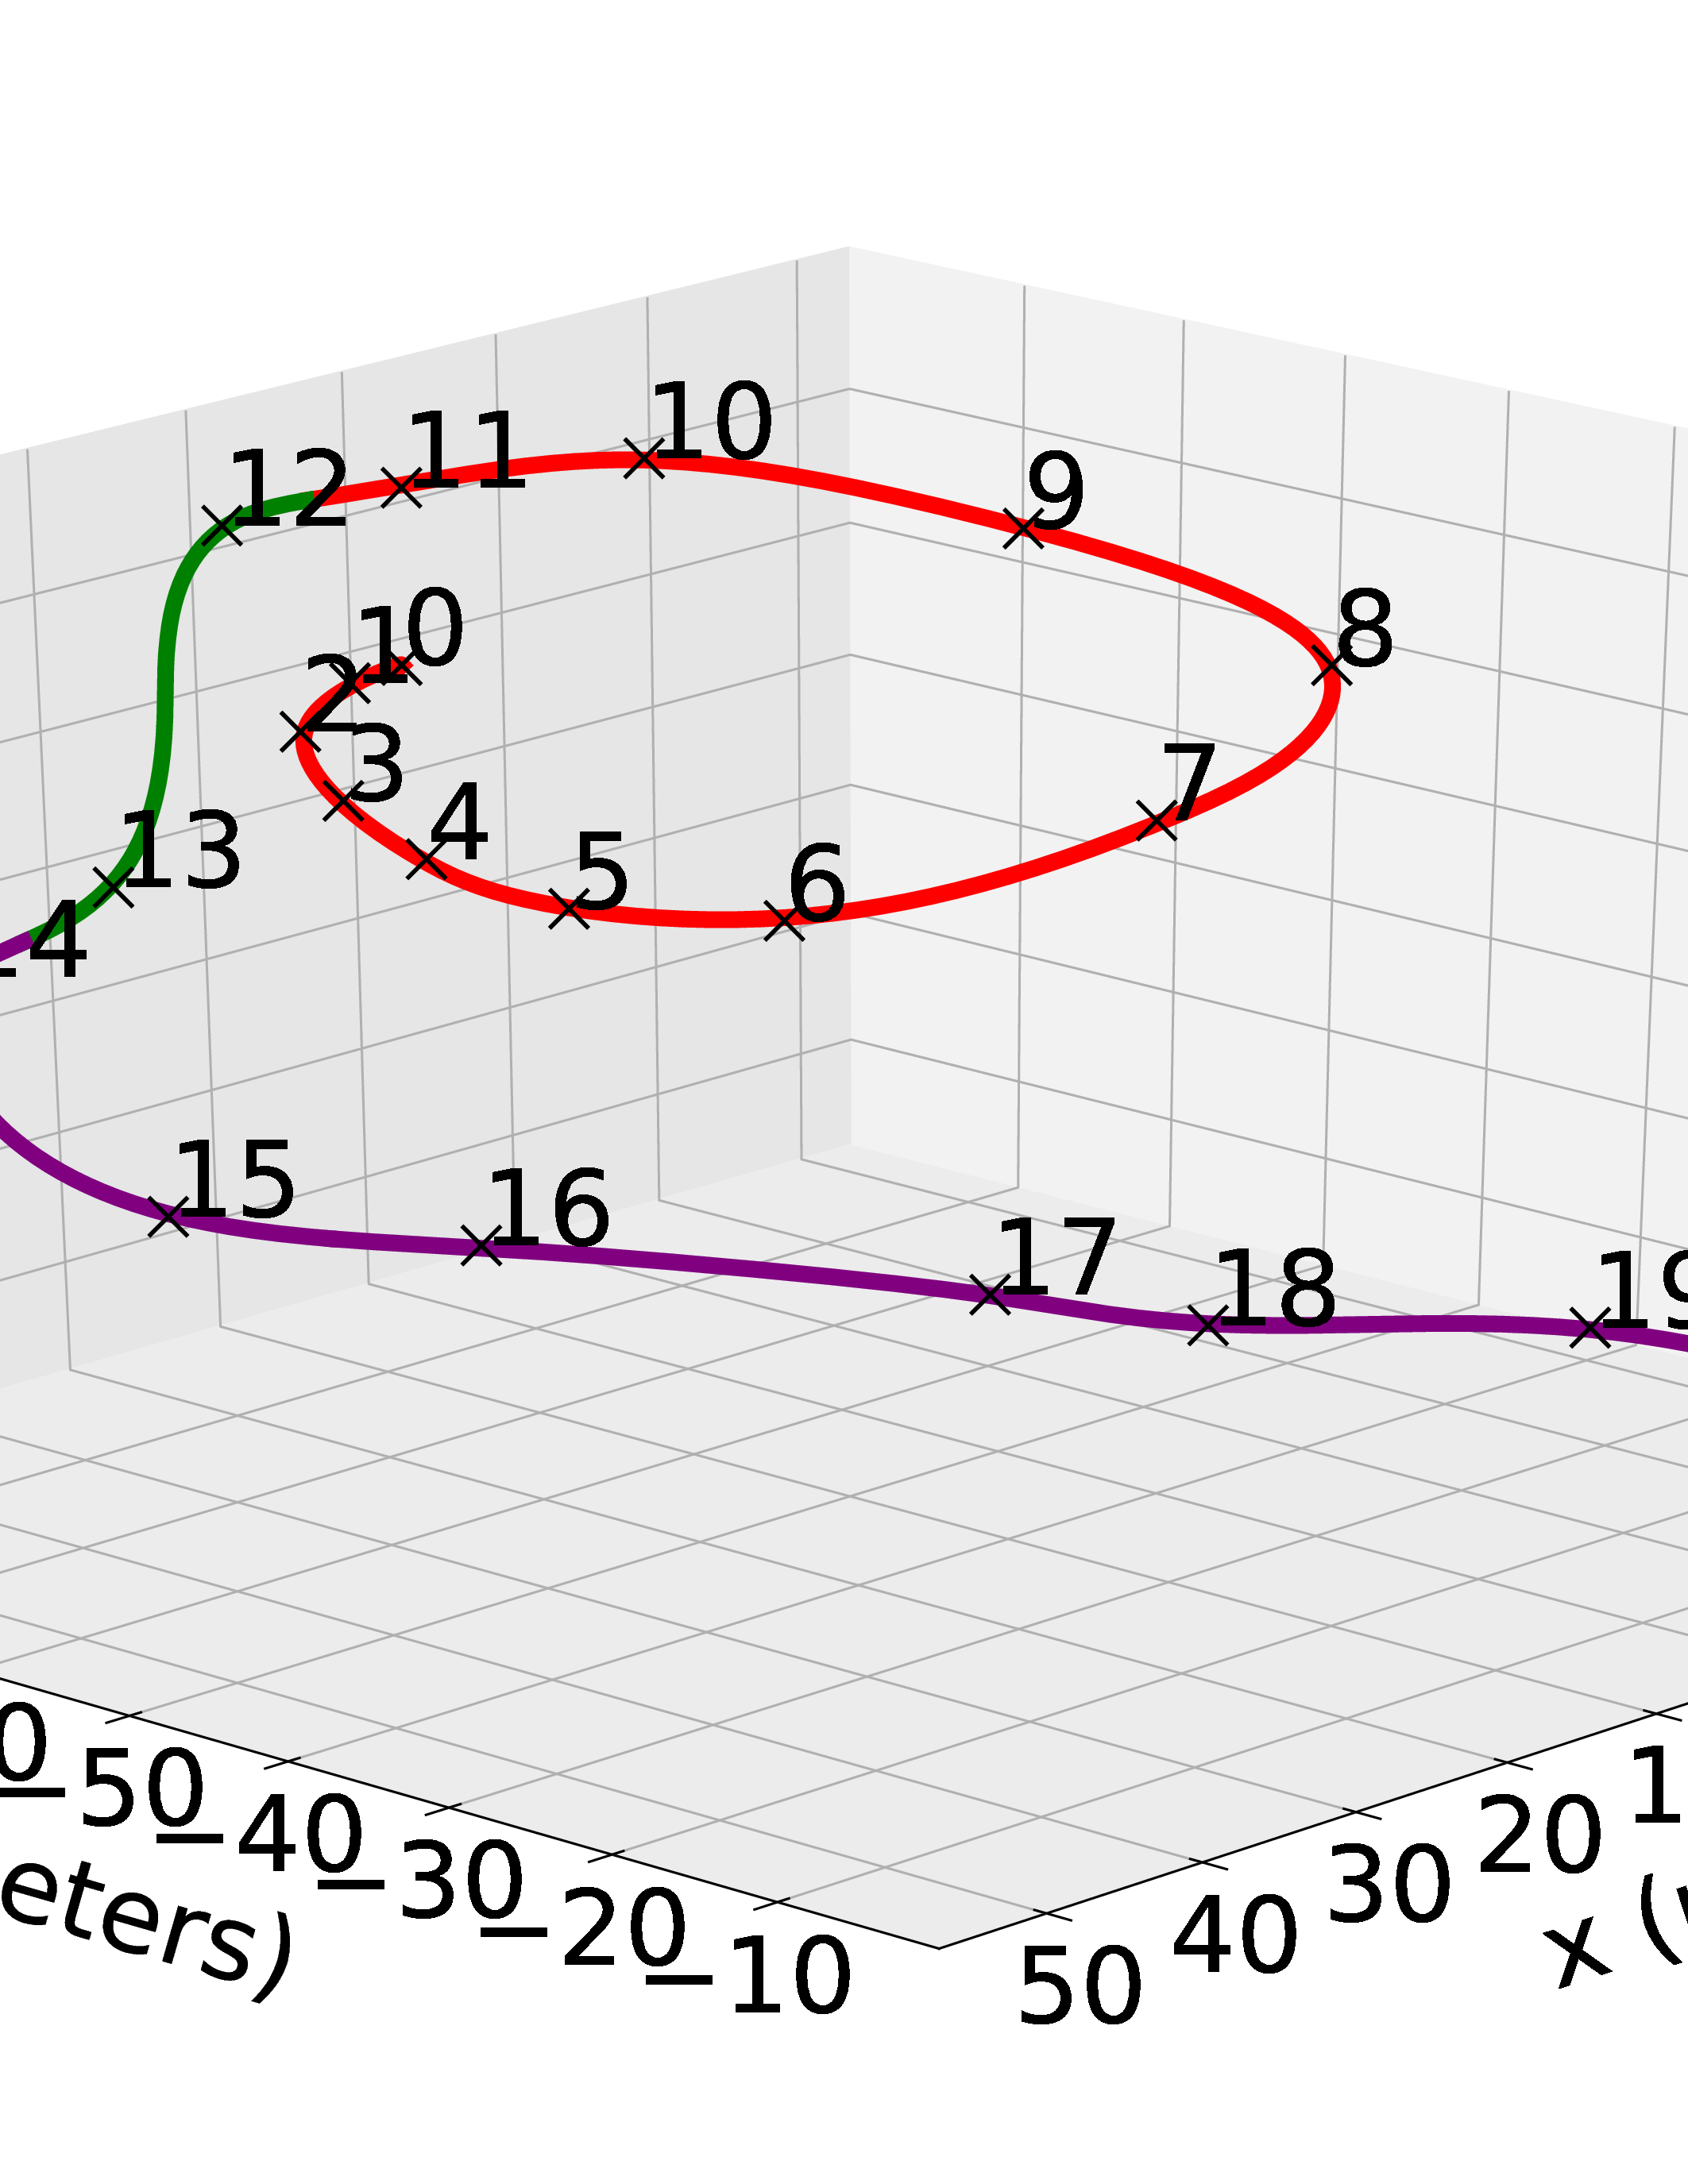}
\includegraphics[width=0.49\linewidth]{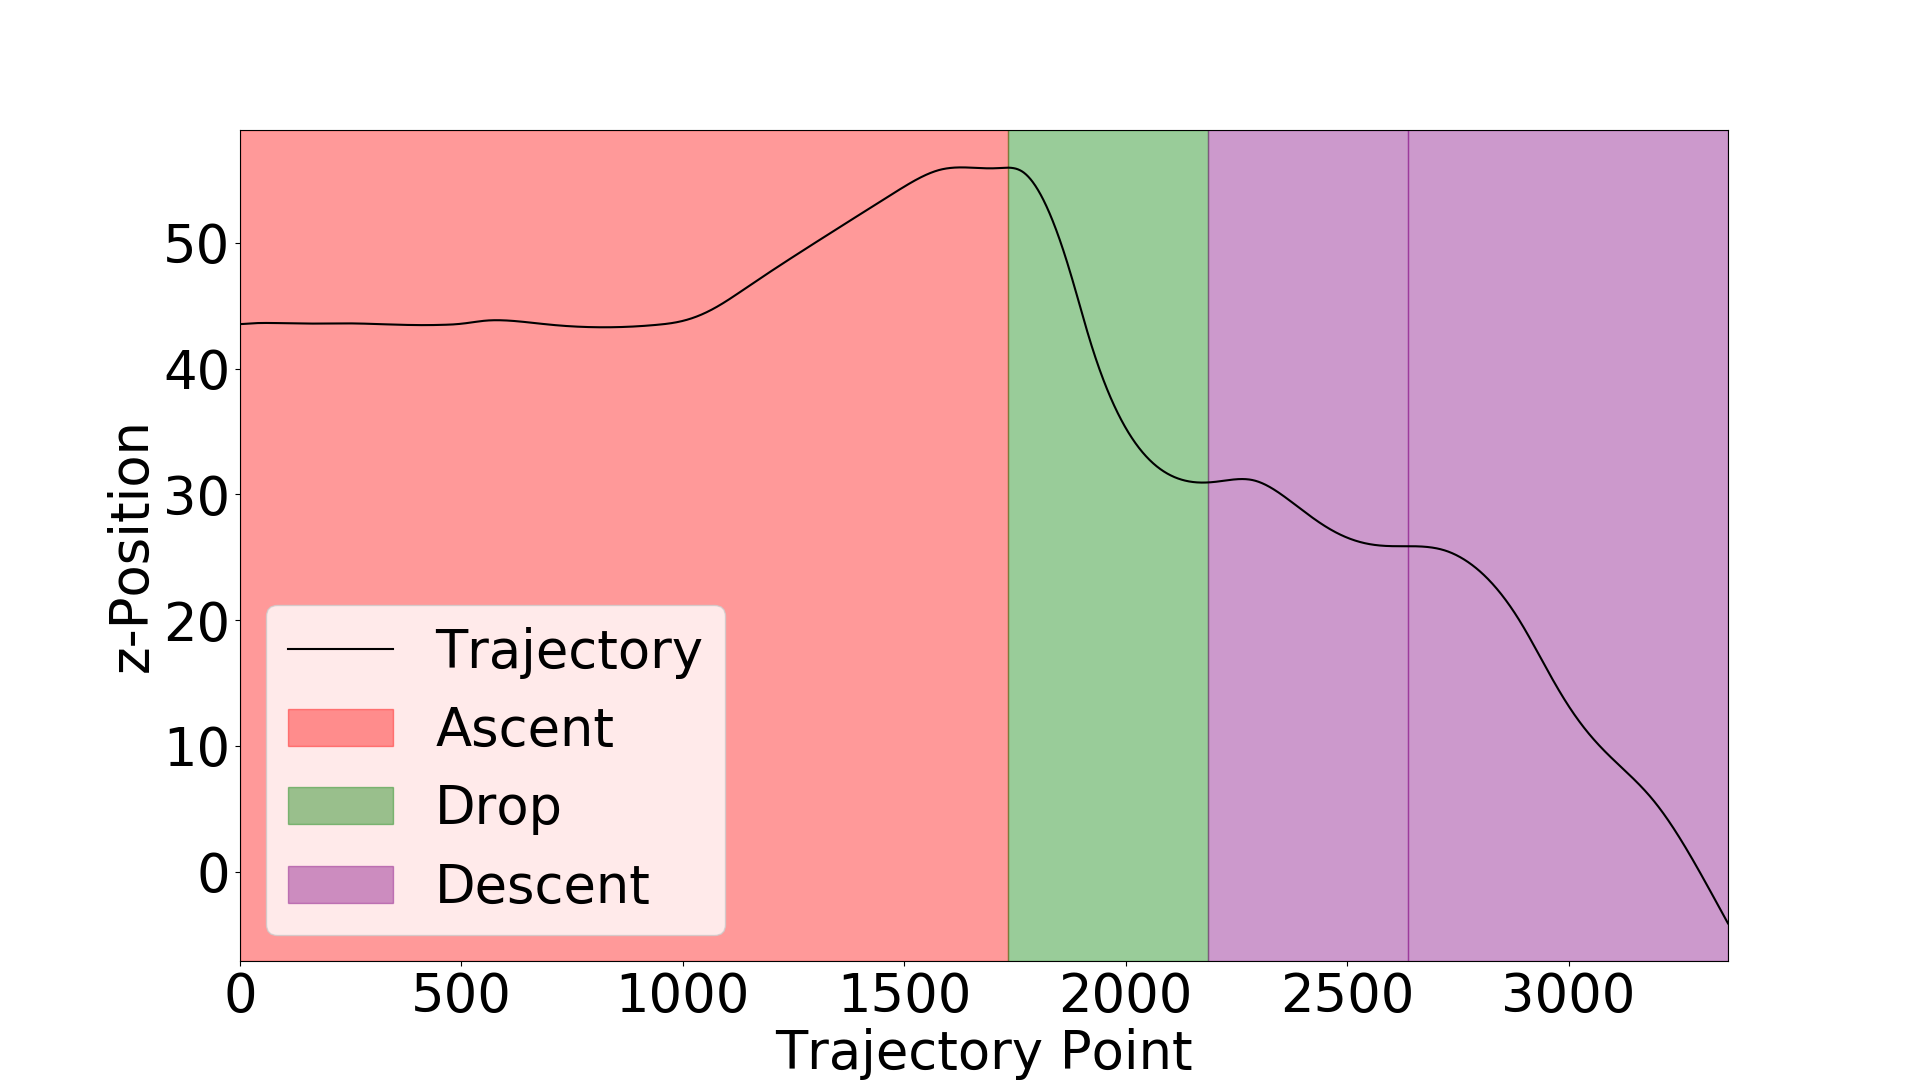}
\captionof{figure}{Height Difference $1m$, Min Duration $5s$.}
\label{fig:choosing_traj_segment}
\end{center}

\clearpage

\subsection{Controller Stability} \label{app:controller_stability}

\rebuttal{
To increase the stability of the controller between segments, we perform nonlinear MPC optimization with a real-time iteration (RTI) scheme \cite{diehl2009controlstab}. The fact that only a single optimization iteration is done for each timestamp allows a smooth transition of the commanded actions while switching segments. A qualitative analysis is illustrated by Figure~\ref{fig:appendix_control_stab}. The controller's outputs remain smooth over time during switching for any pair of segments.
}

\begin{center}
\includegraphics[width=\linewidth]{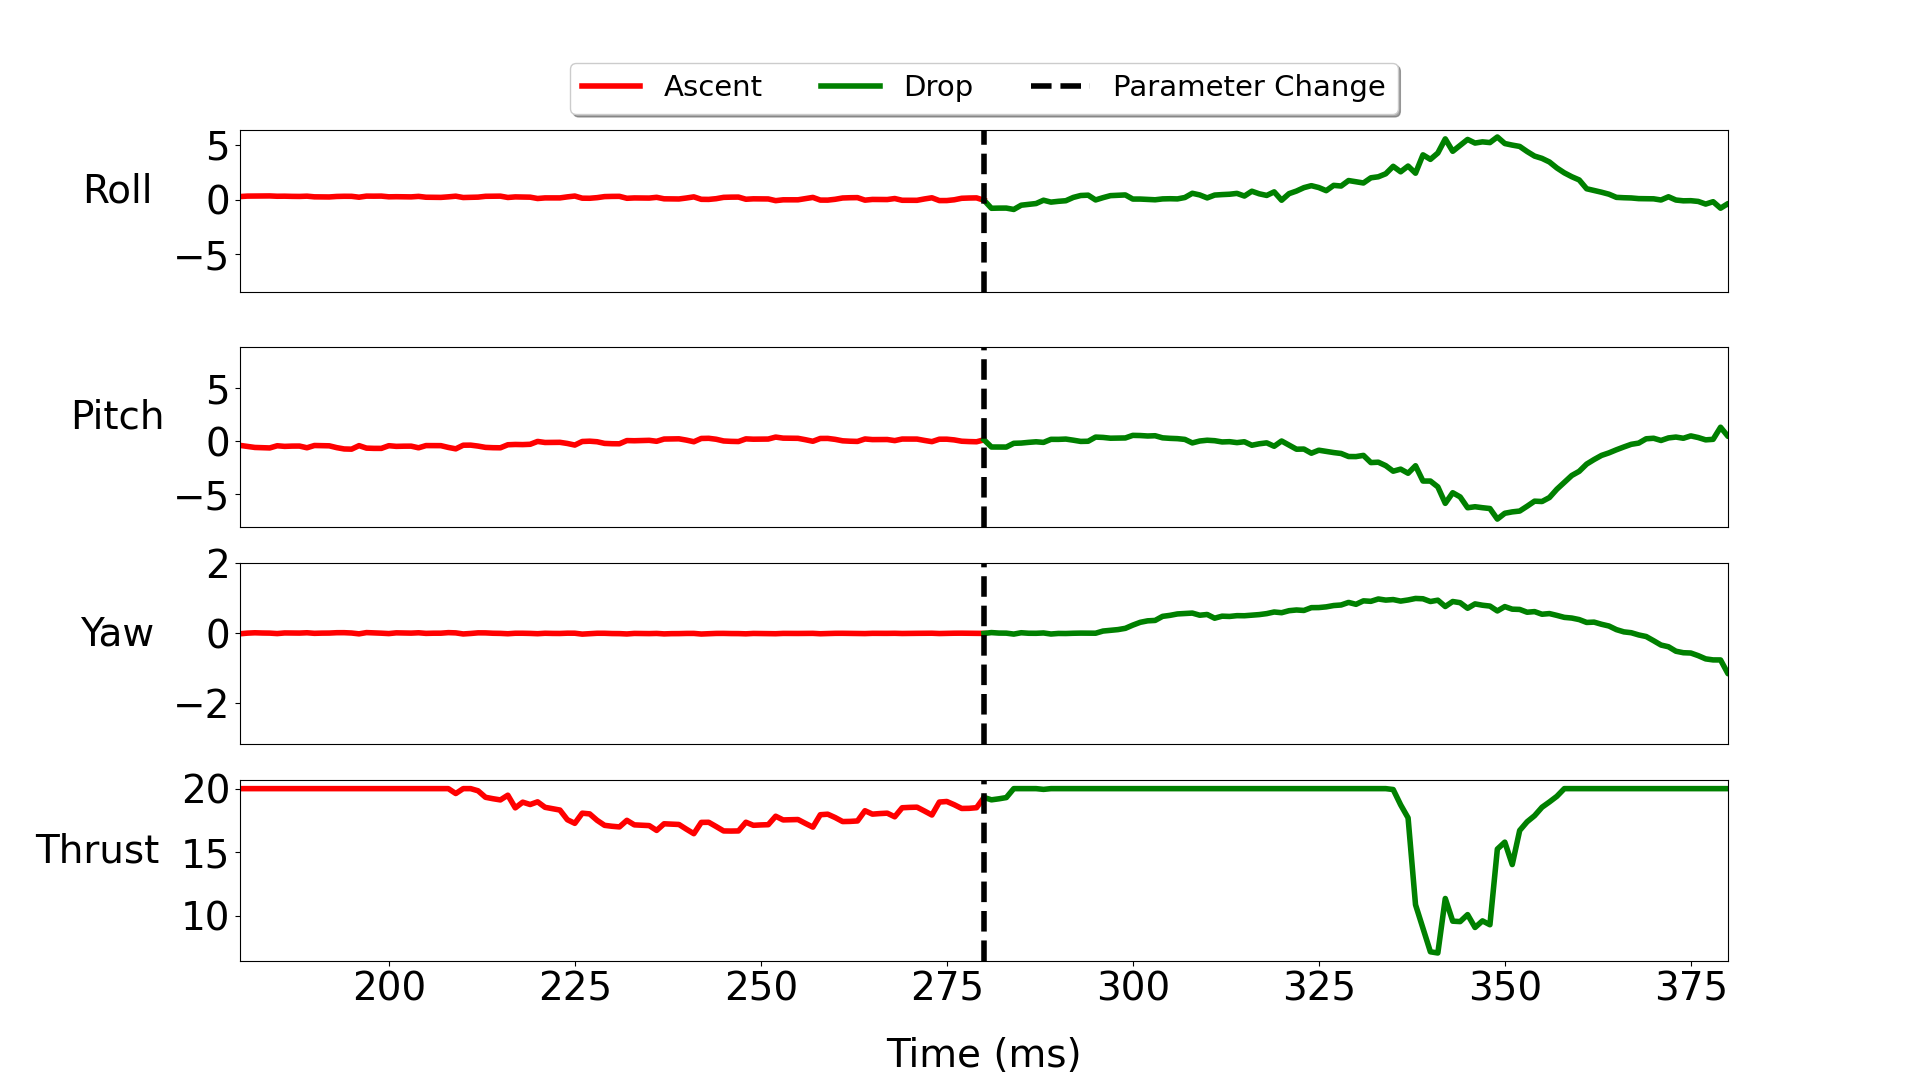}
\includegraphics[width=\linewidth]{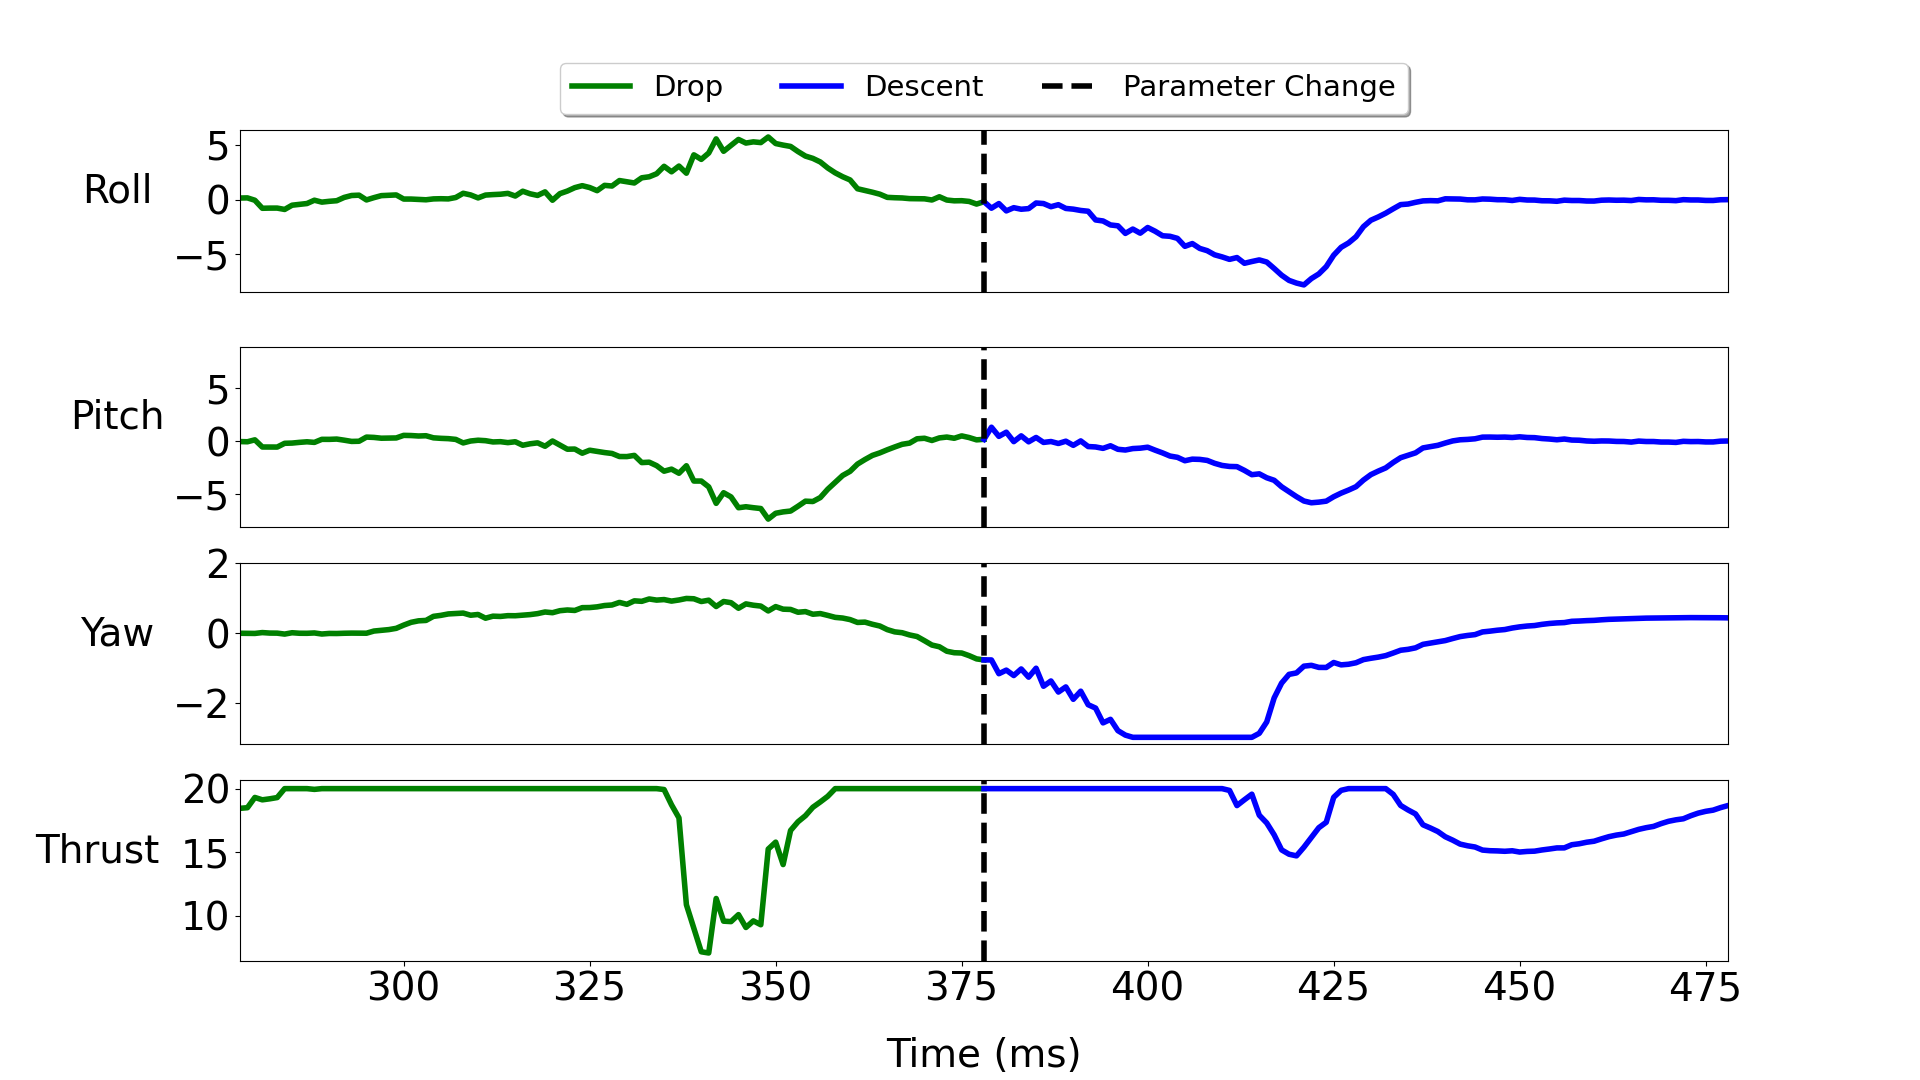}
\includegraphics[width=\linewidth]{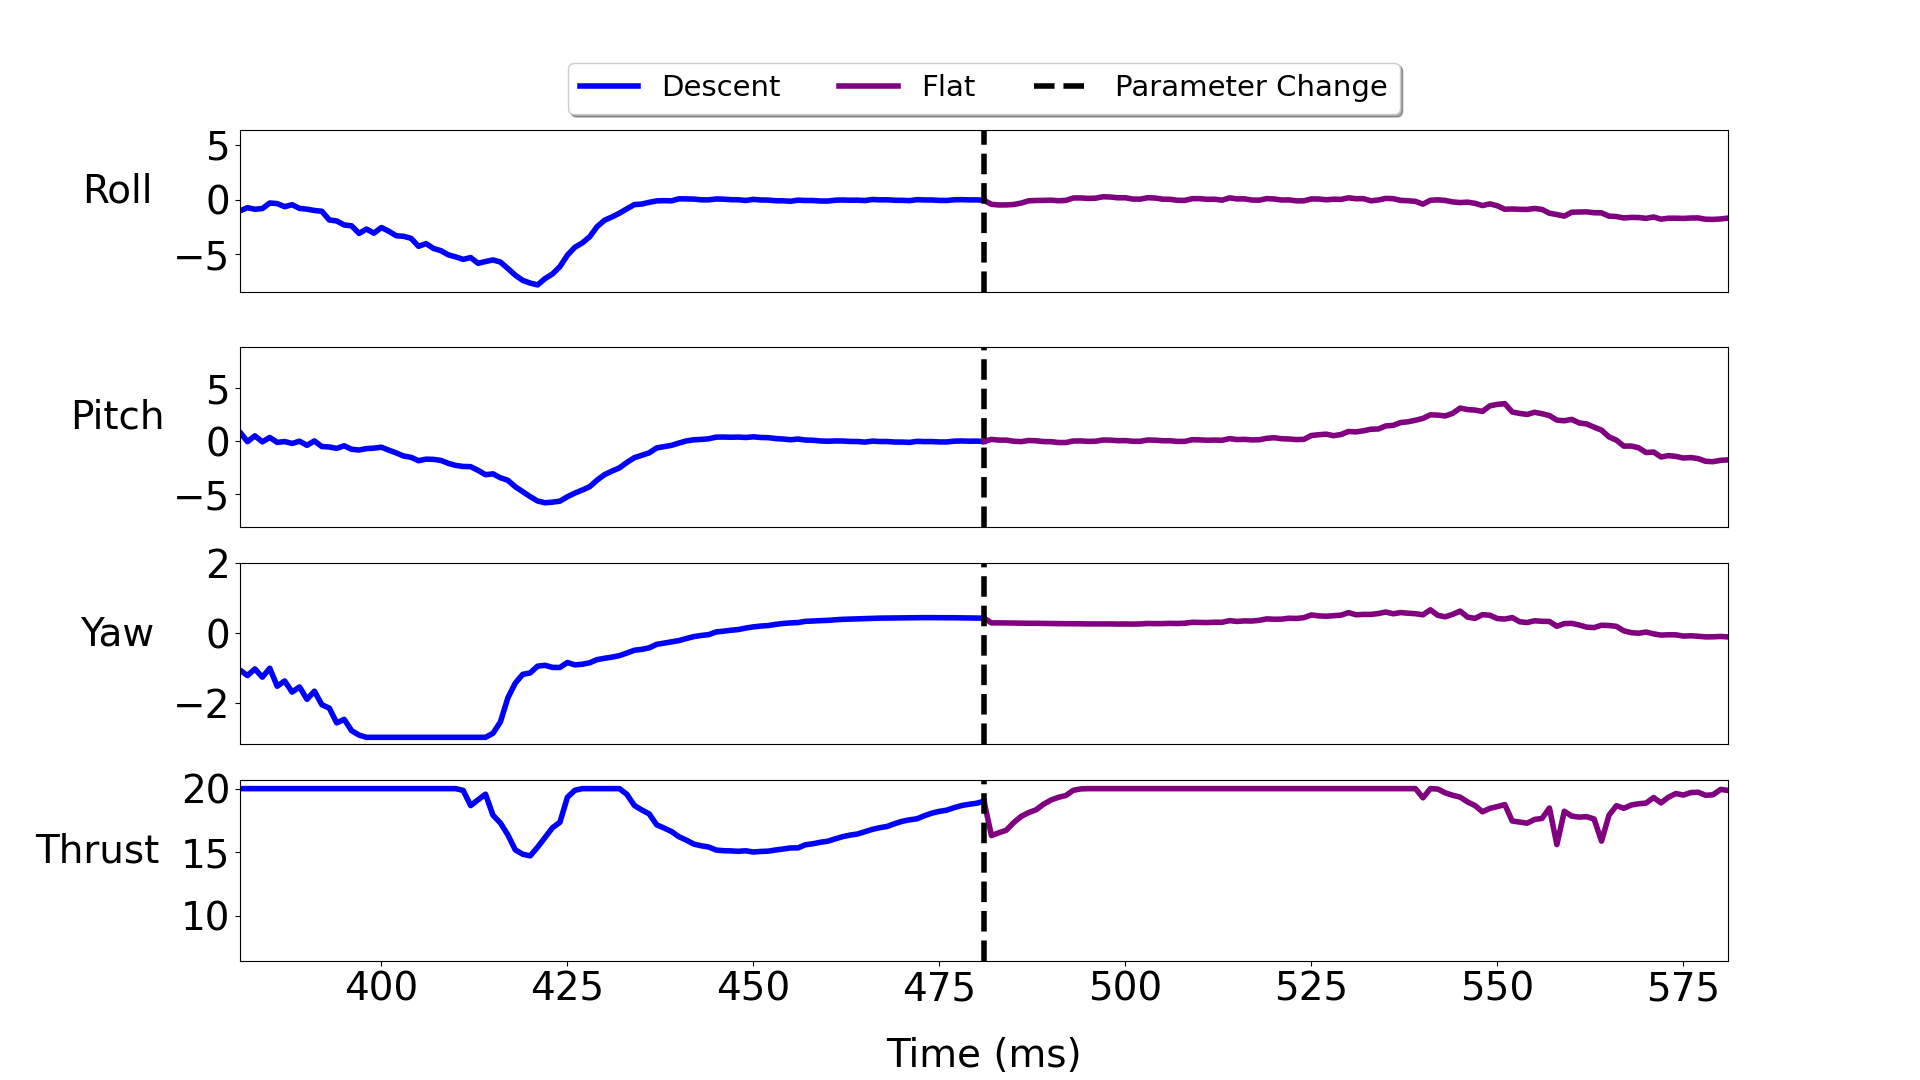}
\captionof{figure}{Effects of parameter change on the stability of the controller on the Drop track. The controller's outputs remain smooth over time during switching for any pair of segments.}
\label{fig:appendix_control_stab}
\end{center}
